# Supplementary material for: BIISQ: Bayesian nonparametric discovery of Isoforms and Individual Specific Quantification
Source: arXiv:1703.08260 ancillary file (2017-03-24)
Supplement: Supplementary file 1 [file BIISQ-supplement.pdf]

# BIISQ: Bayesian nonparametric discovery of Isoforms and Individual Specific Quantification supplementary data

Derek Aguiar[1], Li-Fang Cheng[2], Bianca Dumitrascu[3], Fantine Mordelet[4], Athma Pai[5], & Barbara E Engelhardt[1,6]

[1] *Department of Computer Science, Princeton University, Princeton, NJ*

[2] *Department of Electrical Engineering, Princeton University, Princeton, NJ*

[3] *Lewis Sigler Institute, Princeton University, Princeton, NJ*

[4] *Institute for Genome Sciences and Policy, Duke University, Durham, NC*

[5] *Department of Biology, Massachusetts Institute of Technology, Cambridge, MA*

[6] *Center for Statistics and Machine Learning, Princeton University, Princeton, NJ*

| | |
|---|---|
| Supplementary Figure 1 | An example to demonstrate isoform discovery evaluation criteria. |
| Supplementary Figure 2 | Recall and precision for BEERS data by number of transcripts. |
| Supplementary Figure 3 | Recall and precision for BEERS data by number of exons. |
| Supplementary Figure 4 | The number of correctly inferred and expressed transcripts in BEERS data by exon composition. |
| Supplementary Figure 5 | The number of correctly inferred and expressed transcripts in BEERS data by coverage. |
| Supplementary Figure 6 | Read aligner performance (precision) on Iso-Seq data. |
| Supplementary Figure 7 | Read aligner performance (true positives) on Iso-Seq data. |
| Supplementary Figure 8 | Correlation of expression values for shared transcripts across methods. |
| Supplementary Figure 9 | The number of correctly inferred and expressed transcripts in Iso-Seq data by exon composition. |
| Supplementary Figure 10 | The number of correctly inferred and expressed transcripts in Iso-Seq data by span. |
| Supplementary Figure 11 | Method runtimes as a function of gene length on Iso-Seq data. |
| Supplementary Figure 12 | Method runtimes as a function of read length on Iso-Seq data. |
| Supplementary Figure 13 | Method runtimes as a function of the number of exons on Iso-Seq data. |
| Supplementary Figure 14 | Method runtimes as a function of span on Iso-Seq data. |
| Supplementary Figure 15 | The density of genes with varying numbers of alternative isoforms by (left) population and (right) sex. |
| Supplementary Figure 16 | Genotype PCs for Geuvadis data. |

| | |
|---|---|
| Supplementary Figure 17 | BIISQ cis-eQTL -log(p-values) vs. GEUVADIS study (EUR population) cis-eQTL -log(p-values). |
| Supplementary Figure 18 | BIISQ cis-eQTL -log(p-values) vs. GEUVADIS study (YRI population) cis-eQTL -log(p-values). |
| Supplementary Figure 19 | BIISQ cis-trQTL -log(p-values) vs. GEUVADIS study (EUR population) cis-trQTL -log(p-values). |
| Supplementary Figure 20 | BIISQ cis-eQTL -log(p-values) vs. BIISQ cis-trQTL -log(p-values). |
| Supplementary Figure 21 | GEUVADIS study cis-eQTL -log(p-values) vs. GEUVADIS study (EUR population) cis-trQTL -log(p-values). |
| Supplementary Figure 22 | GEUVADIS study cis-eQTL -log(p-values) vs. GEUVADIS study (YRI population) cis-trQTL -log(p-values). |
| Supplementary Figure 23 | Theoretical vs. sample quantiles for variant enrichment. |
| Supplementary Figure 24 | A graphical model for the generation of reads in RNA-seq data from $M$ samples. |
| Supplementary Table 1 | Iso-Seq gold standard. |
| Supplementary Table 2 | GEUVADIS population specific hypergeometric tests. |
| Supplementary Table 3 | GEUVADIS super-population specific hypergeometric tests. |
| Supplementary Table 4 | GEUVADIS sex specific hypergeometric tests. |
| Supplementary Table 5 | PEER factor optimization. |
| Supplementary Table 6 | Variant enrichment sample descriptions. |
| Supplementary Table 7 | Functionary categories for enrichment analysis. |
| Supplementary Table 8 | Functional enrichment for genes with at least one trQTL. |
| Supplementary Table 9 | Functional enrichment for isoforms with $> 1$ transcripts. |
| Supplementary Table 10 | Functional enrichment for isoforms with $> 4$ transcripts. |

| | |
|---|---|
| Supplementary Table 11 | Functional enrichment for isoforms with $> 6$ transcripts. |
| Supplementary Table 12 | Model and variational parameters, conditional distributions and expectations. |
| Supplementary Table 13 | Updates for variational parameters in the BIISQ model. |
| Supplementary Note | Read mapping likelihood |
| Supplementary Methods | Additional notes on the BIISQ model, posterior inference, and simulations. |

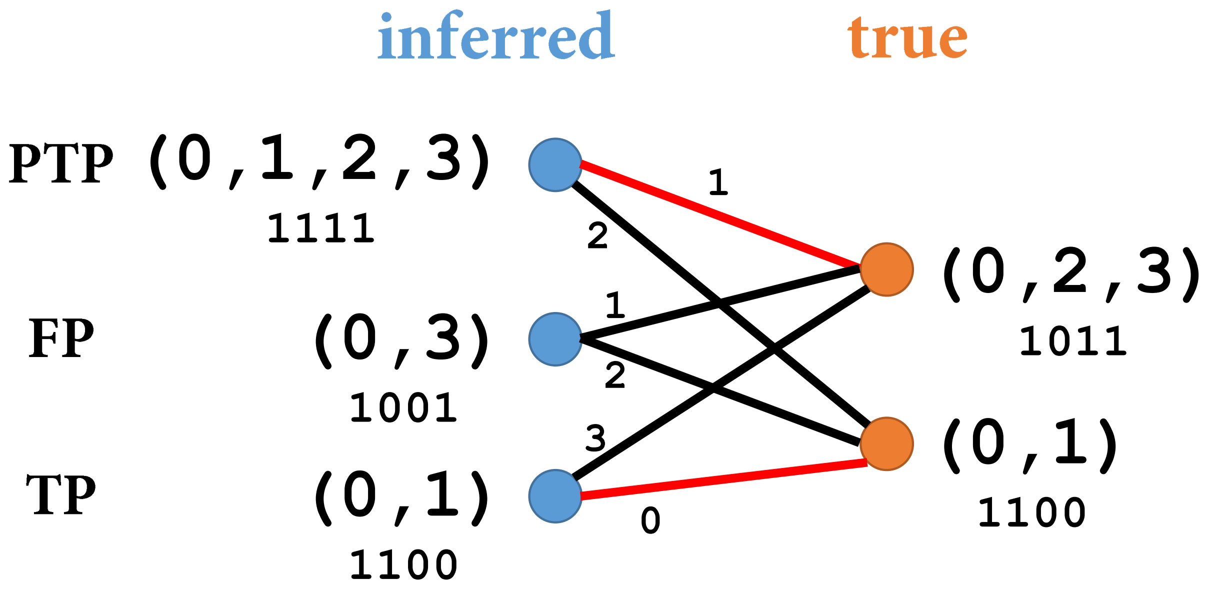


Figure 1: **An example to demonstrate isoform discovery evaluation criteria.** Algorithmically inferred isoforms are shown on the left; true isoforms are depicted on the right. The maximum cardinality minimum weight matching between the inferred and true isoforms is shown in orange edges and defines pairs of inferred and true isoforms that are maximally similar. Pairs with exon distance $> 0$ are partial true positives (PTP), with distance $= 0$ are true positives, and inferred isoforms without a matching true isoform are false positives.

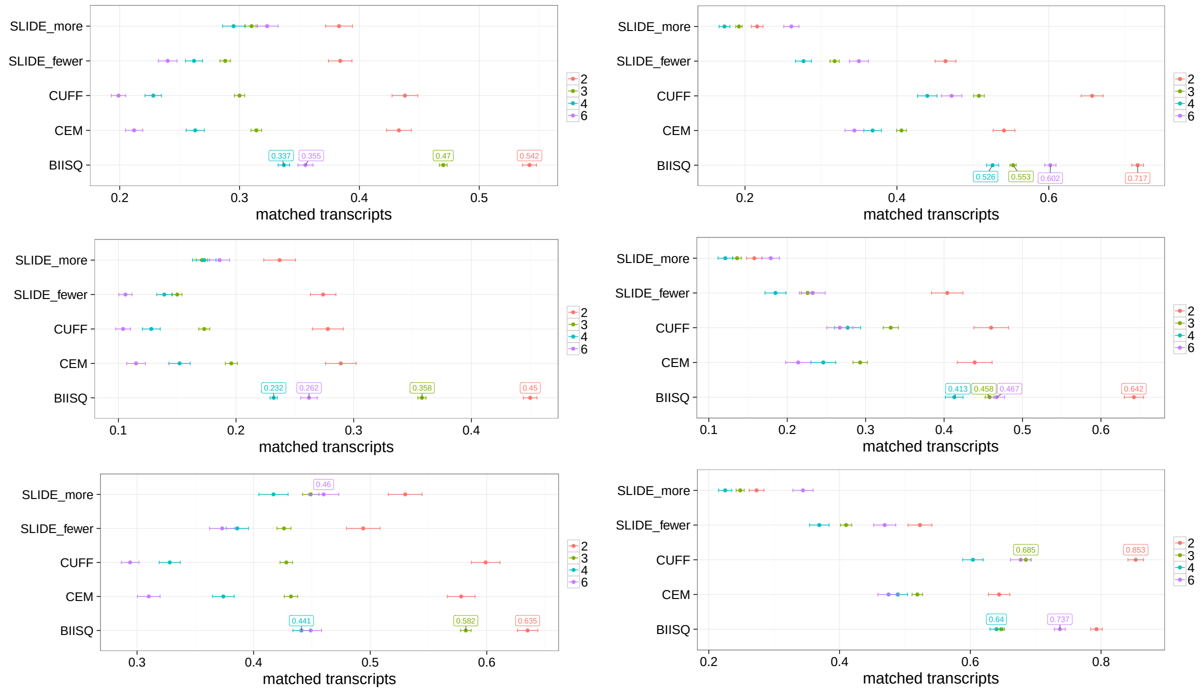


Figure 2: **Recall and precision for BEERS data by number of transcripts.** (Left) Recall and (right) precision for BEERS data by number of transcripts per gene for (top row) both thresholds 0.0 and 0.2, (middle row) threshold 0.0 and (bottom row) threshold 0.2.

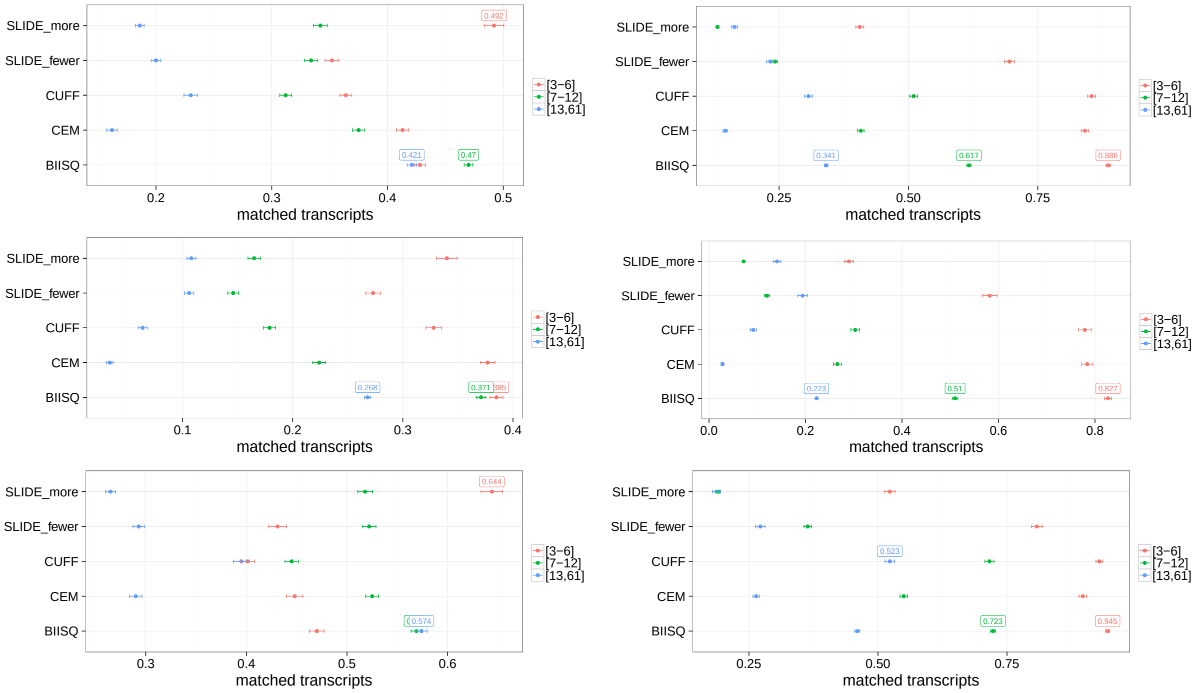


Figure 3: **Recall and precision for BEERS data by number of exons.** (Left) Recall and (right) precision for BEERS data by number of exons per gene for (top row) both thresholds $0.0$ and $0.2$, (middle row) threshold $0.0$ and (bottom row) threshold $0.2$.

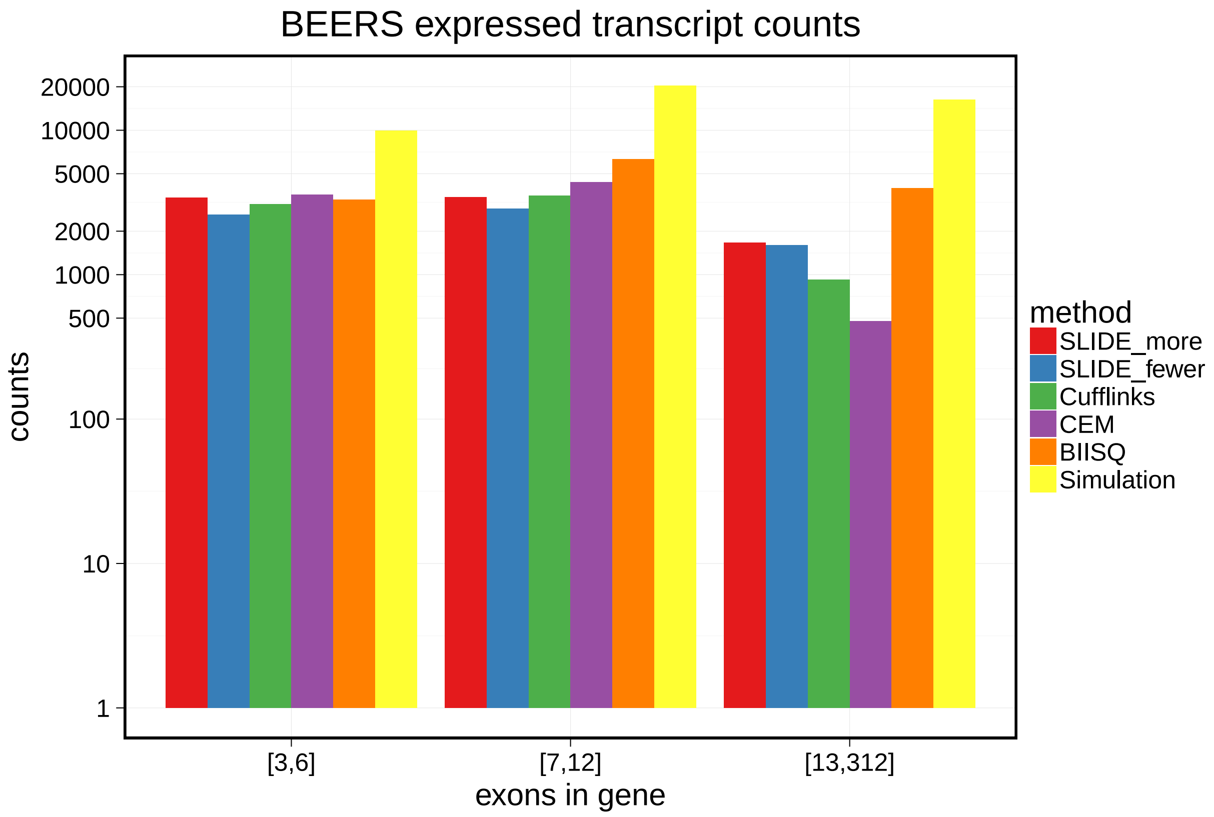


Figure 4: **The number of correctly inferred and expressed transcripts in BEERS data by exon composition.** Genes are divided into three roughly equally sized groups (x-axis) and the number of transcripts inferred by each method is given on the y-axis. The *Simulation* method denotes the known simulated transcript baseline.

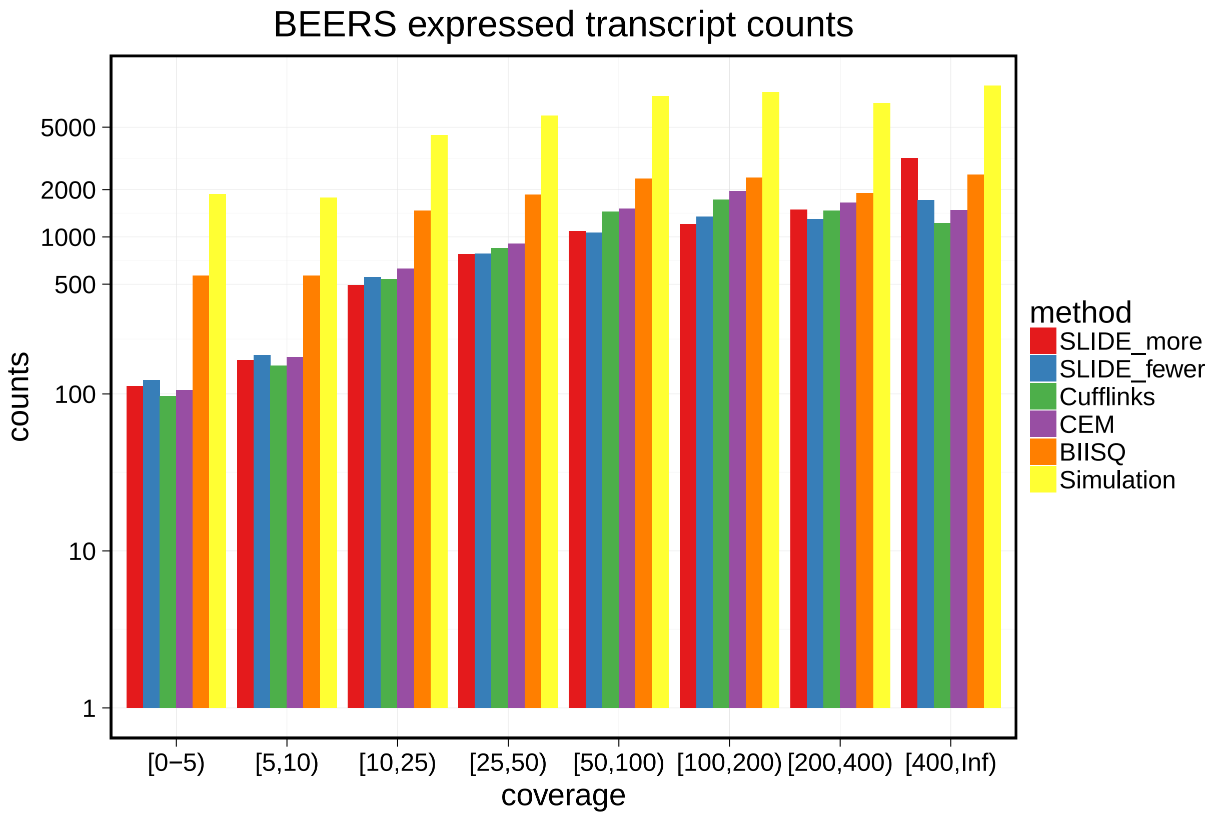


Figure 5: **The number of correctly inferred and expressed transcripts in BEERS data by coverage.** BEERS simulated transcripts were divided into roughly equally sized groups based on coverage (x-axis). The number of inferred transcripts by each method is given on the y-axis. The *Simulation* method denotes the known simulated transcript baseline.

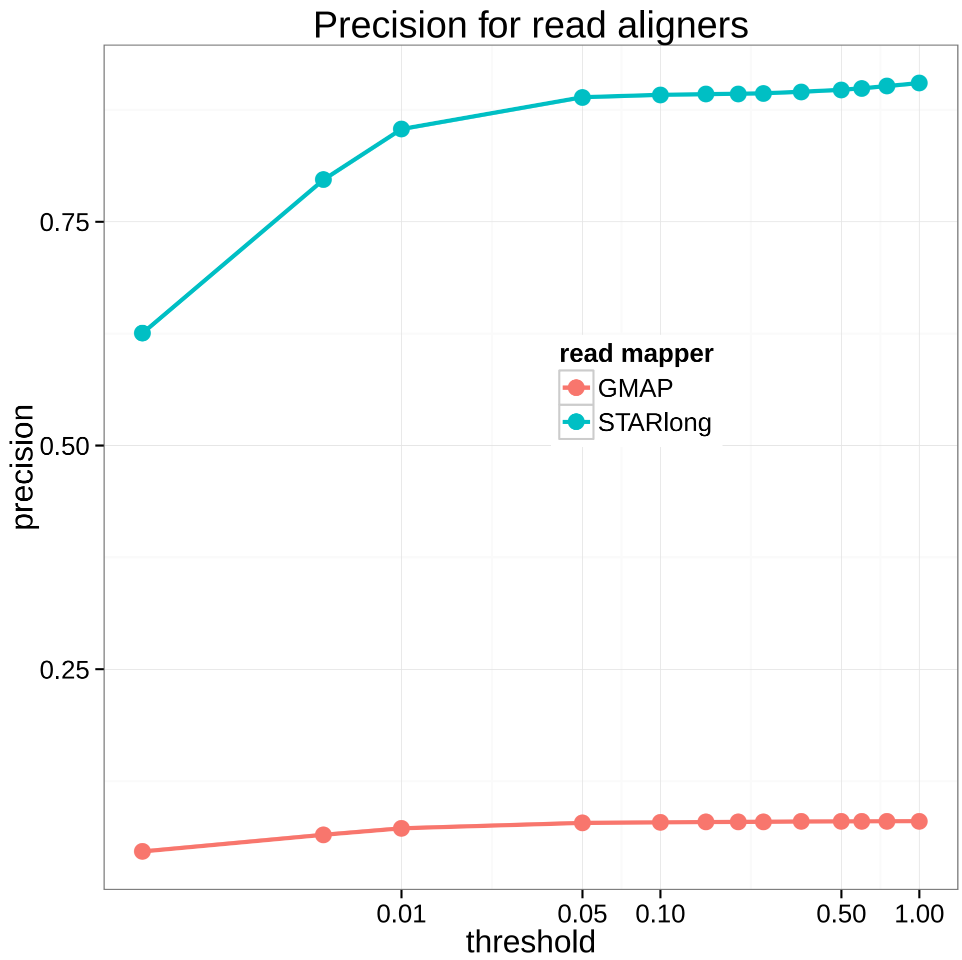


Figure 6: **Read aligner performance (precision) on Iso-Seq data.** Full-length non-chimeric transcripts generated from PacBio Iso-Seq technology was mapped back to the whole human transcriptome from brain, heart, and liver tissue [1]. We mapped assembled transcripts to known annotations to reconstruct gene models for the eight interesting genes in Table 1. The threshold denotes the percentage of non-clipped bases in the read that is allowed to map to non-exonic annotations. STARlong produces much fewer mappings, but with an order of magnitude higher precision.

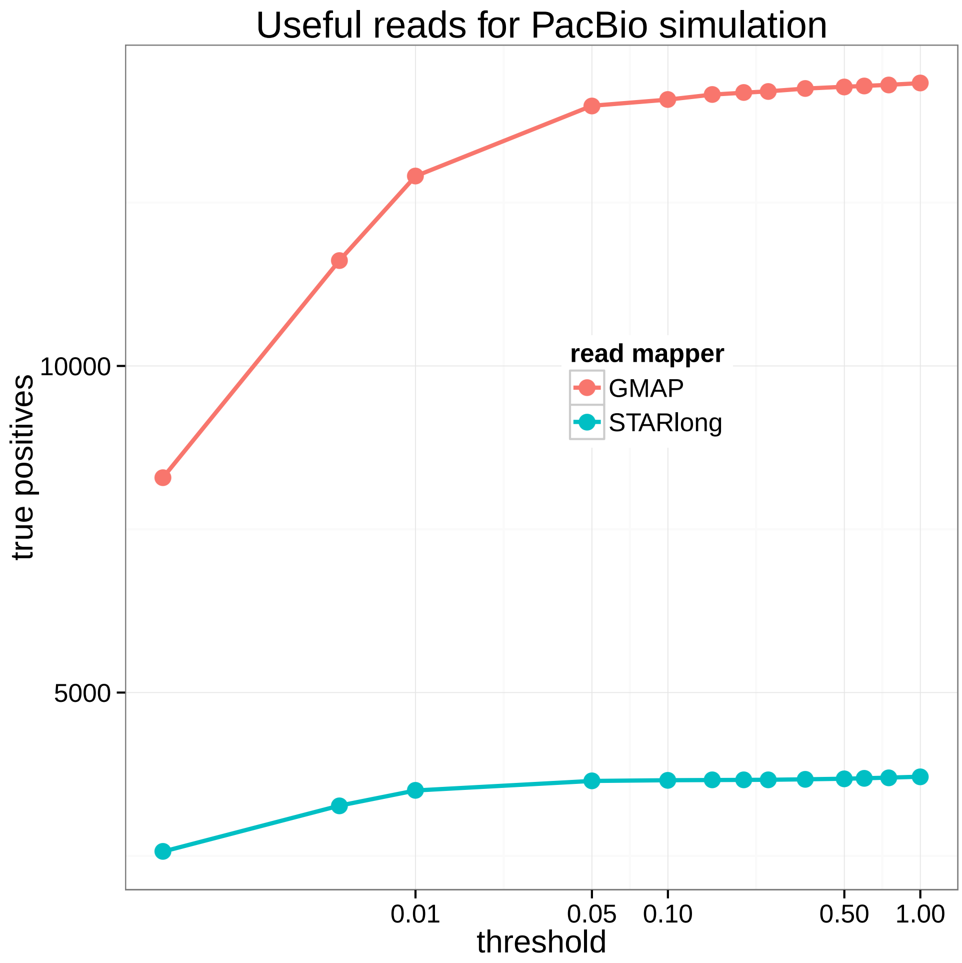


Figure 7: **Read aligner performance (true positives) on Iso-Seq data.** Full-length non-chimeric transcripts generated from PacBio Iso-Seq technology was mapped back to the whole human transcriptome from brain, heart, and liver tissue [1]. We mapped assembled transcripts to known annotations to reconstruct gene models for the eight interesting genes in Table 1. The threshold denotes the percentage of non-clipped bases in the read that is allowed to map to non-exonic annotations. While Figure 6 shows superior precision for STARlong, the presence of annotation enables the filtering of true positives and false positives and GMAP produces more aligned true positives.

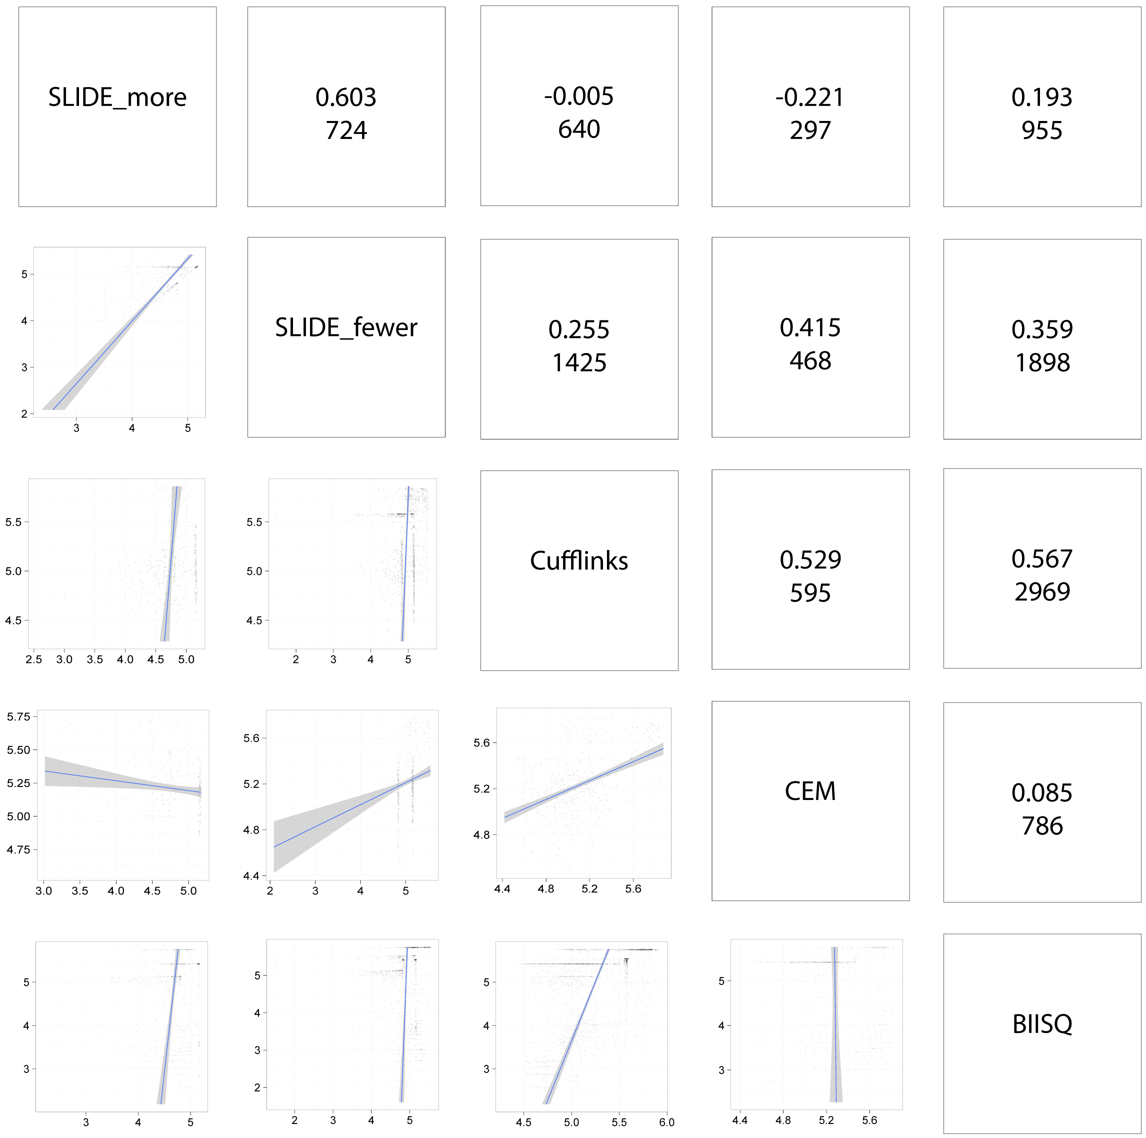


Figure 8: **Correlation of expression values for shared transcripts across methods in the PacBio Iso-Seq data.** Correlation of inferred RPKM between the five methods are plotted where they intersect below the diagonal. Pearson $r$ and the number of observations are given in the upper diagonal.

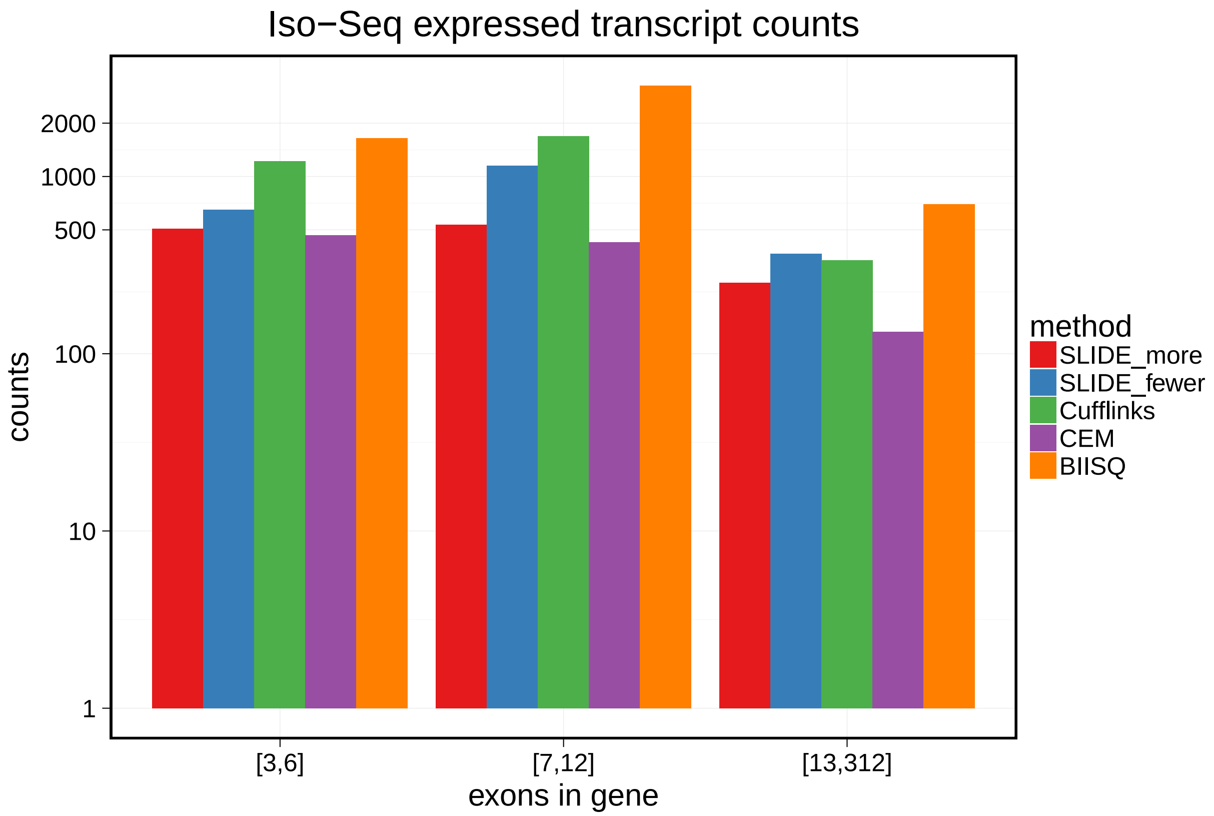


Figure 9: **The number of correctly inferred and expressed transcripts in Iso-Seq data by exon composition.** Genes are divided into three roughly equally sized groups (x-axis) and the number of transcripts inferred by each method is given on the y-axis.

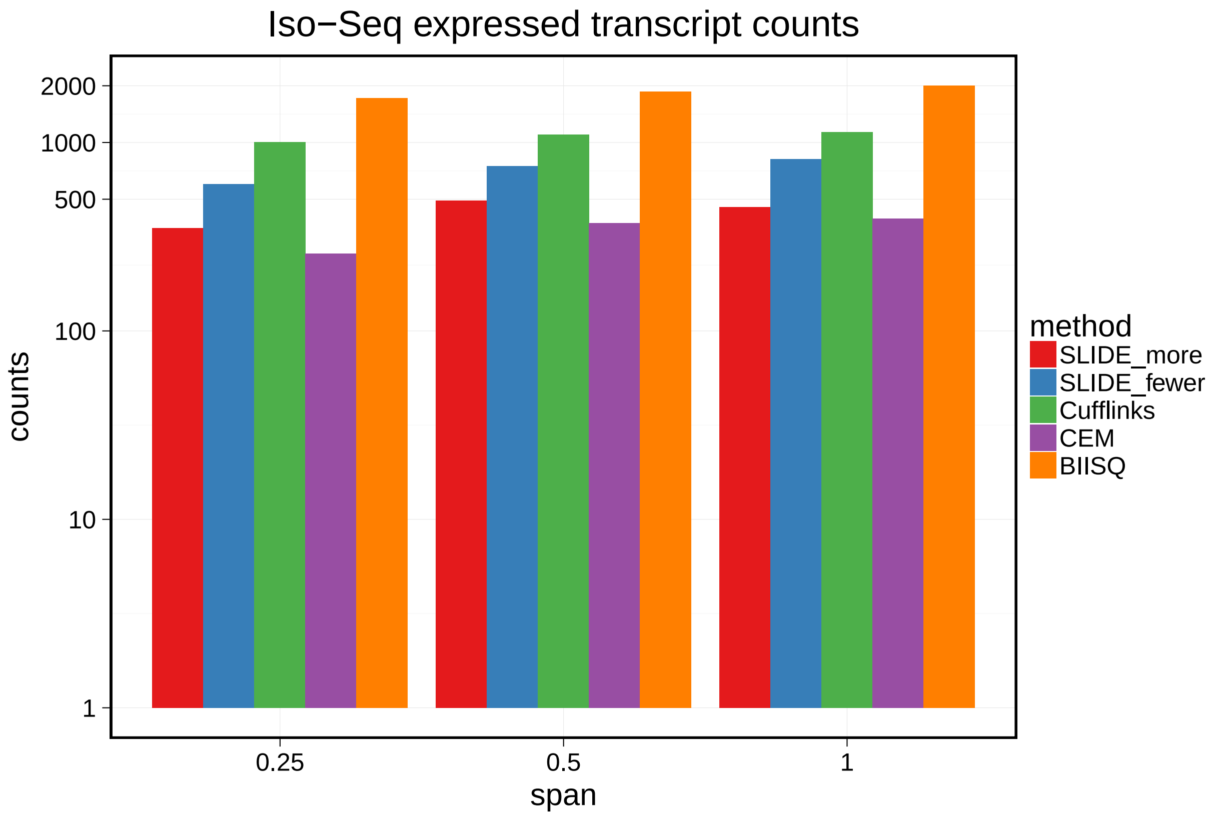


Figure 10: **The number of correctly inferred and expressed transcripts in Iso-Seq data by span.** Iso-Seq generated transcripts were divided into roughly equally sized groups based on span (x-axis). The number of inferred transcripts by each method is given on the y-axis.

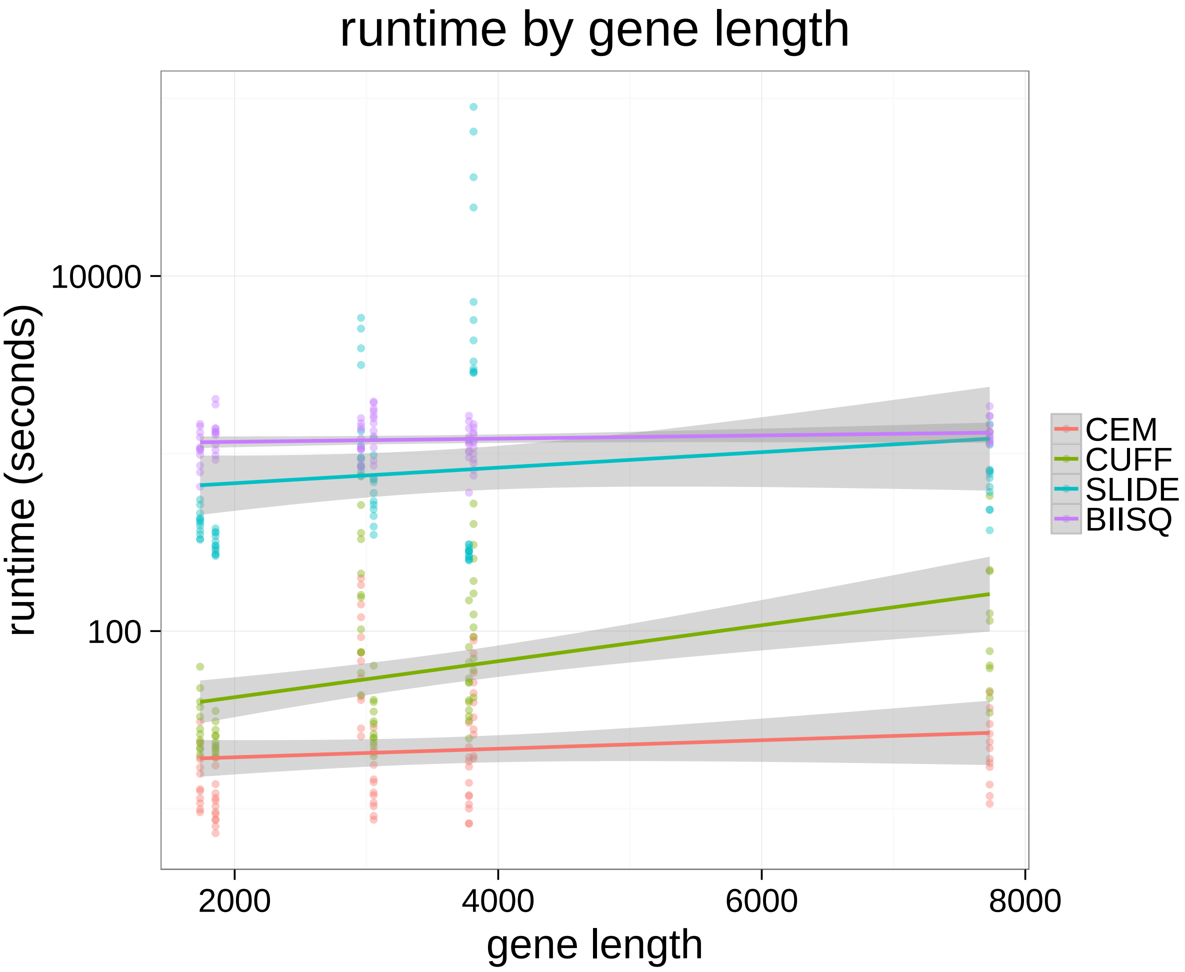


Figure 11: **Method runtimes as a function of gene length on Iso-Seq data.** Runtime is measured in seconds and BIISQ runtimes are an average across 20 runs and do not include the one-time preprocessing for converting aligned reads to read-terms.

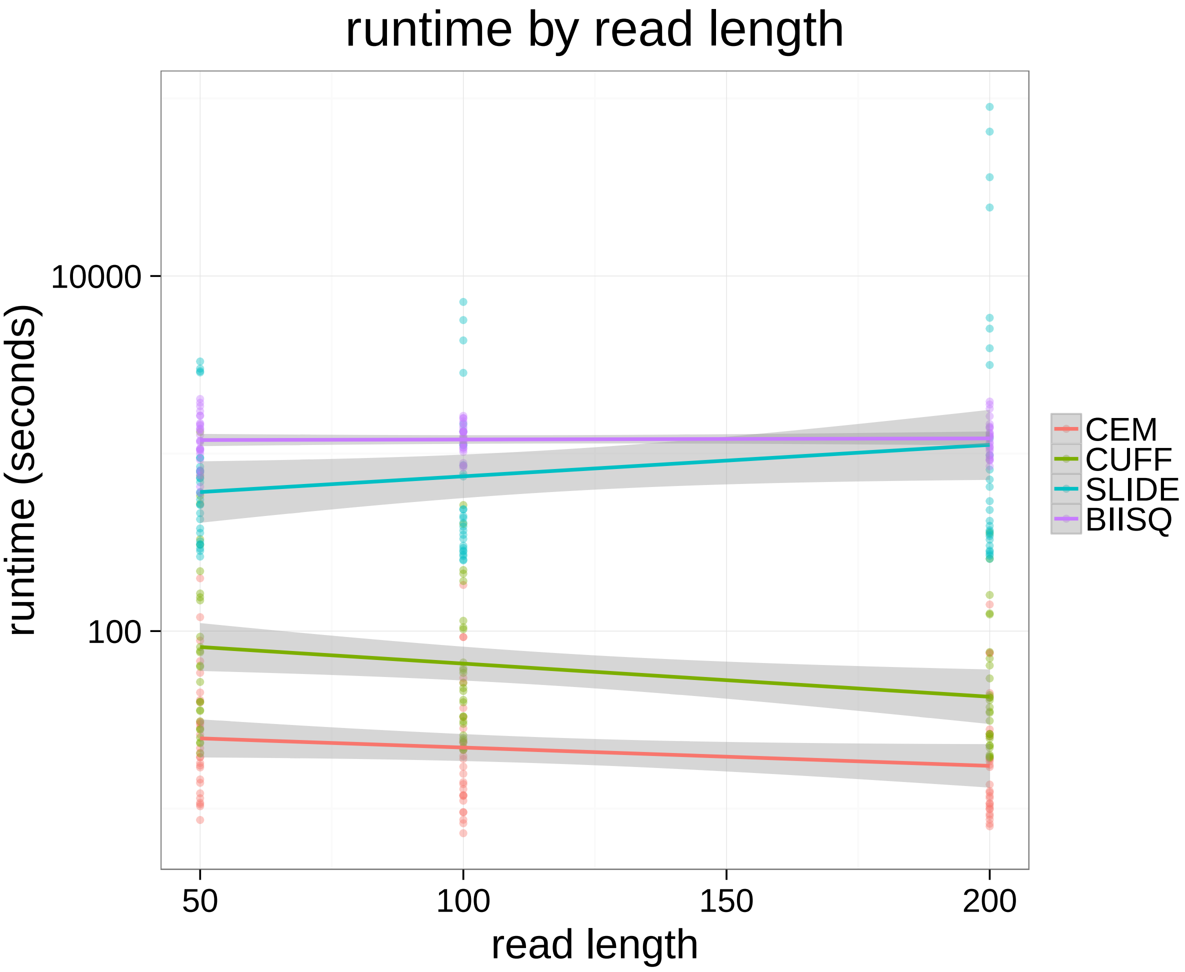


Figure 12: **Method runtimes as a function of read length on Iso-Seq data.** Runtime is measured in seconds and BIISQ runtimes are an average across 20 runs and do not include the one-time preprocessing for converting aligned reads to read-terms.

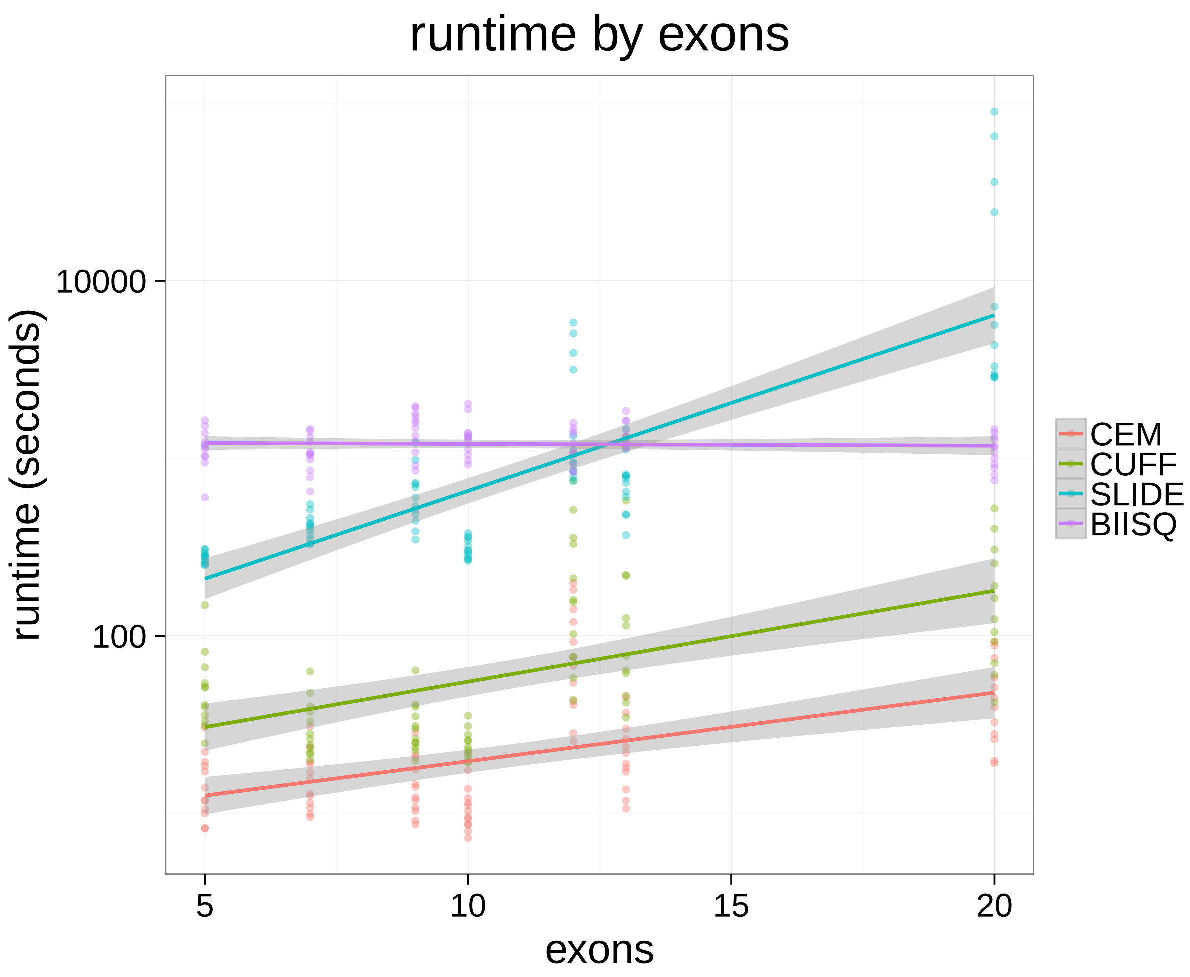


Figure 13: **Method runtimes as a function of the number of exons on Iso-Seq data.** Runtime is measured in seconds and BIISQ runtimes are an average across 20 runs and do not include the one-time preprocessing for converting aligned reads to read-terms.

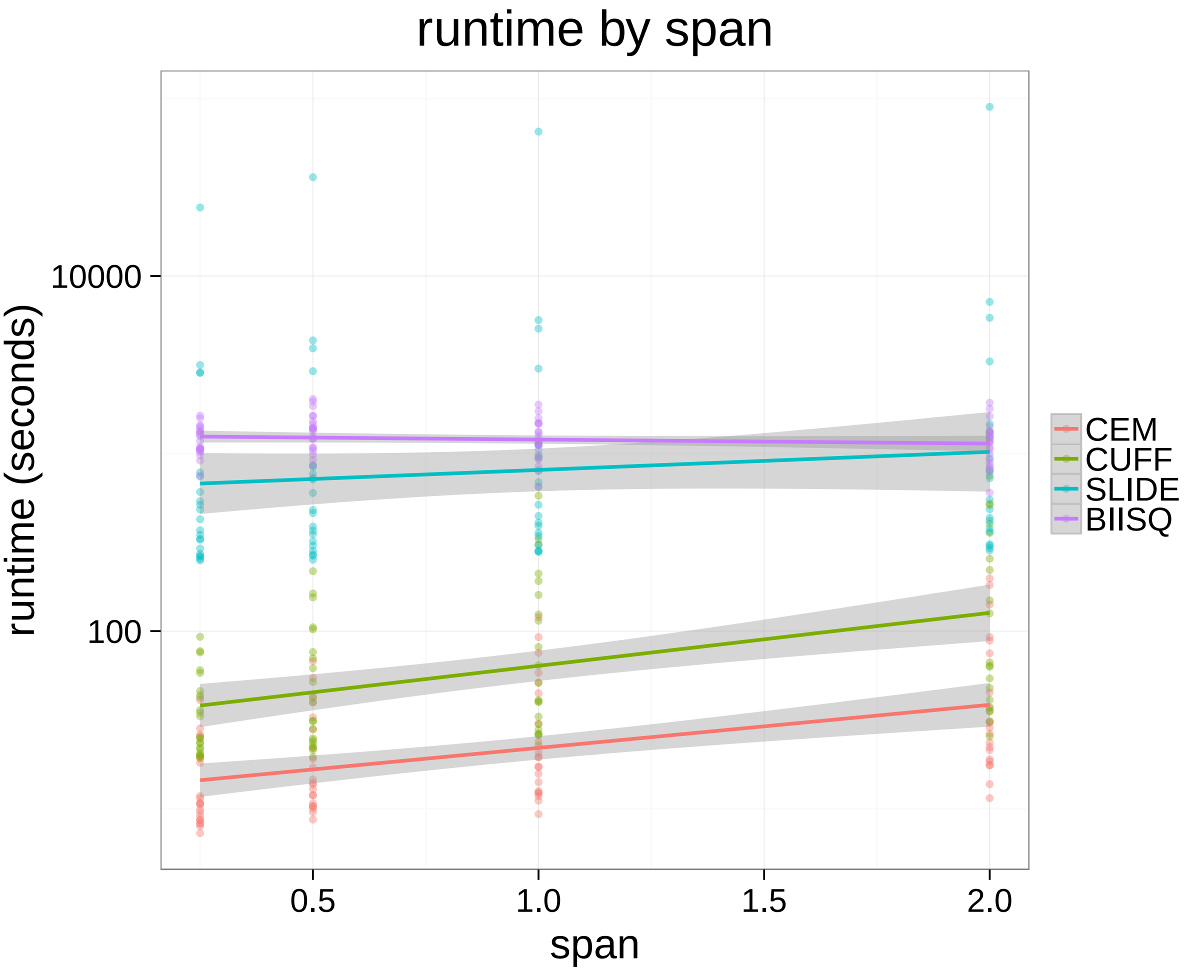


Figure 14: **Method runtimes as a function of span on Iso-Seq data.** Runtime is measured in seconds and BIISQ runtimes are an average across 20 runs and do not include the one-time preprocessing for converting aligned reads to read-terms.

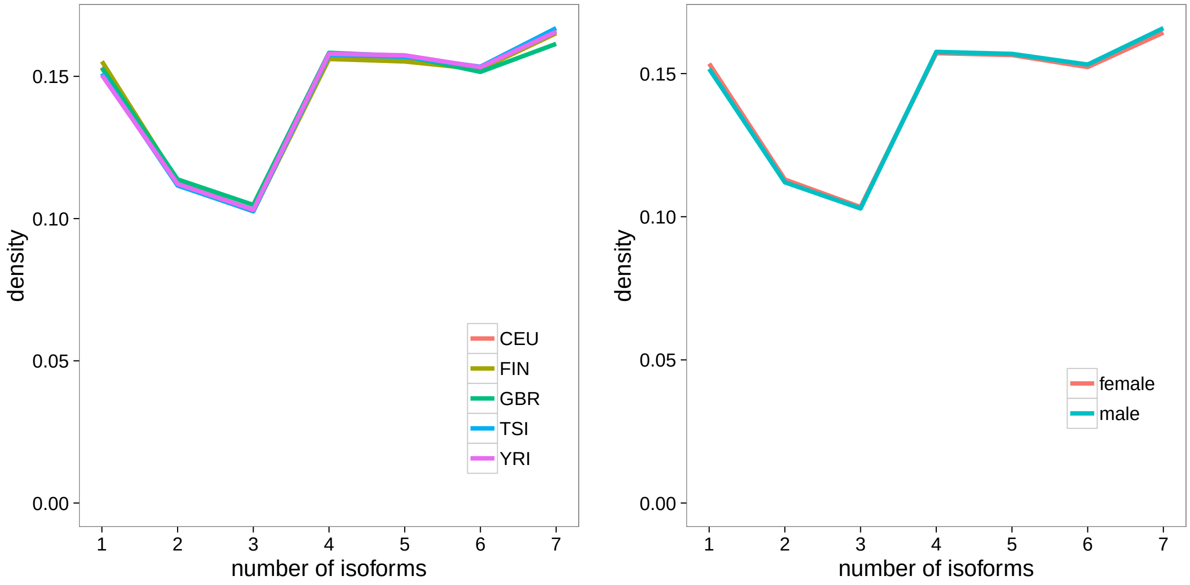


Figure 15: **The density of genes with varying numbers of alternative isoforms by (left) population and (right) sex.**

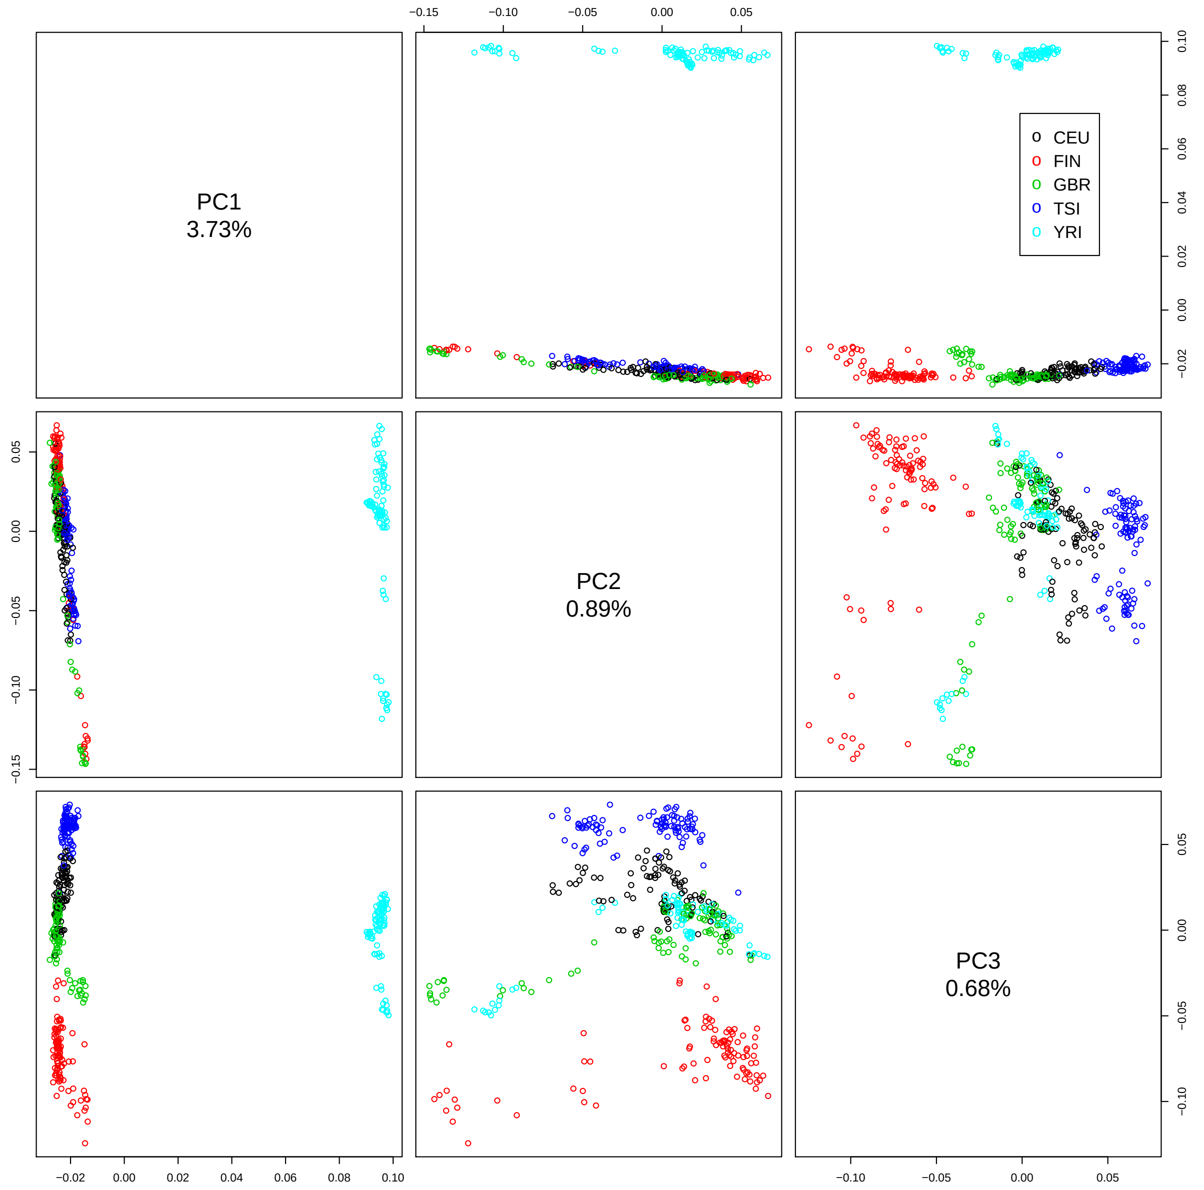


Figure 16: **Genotype principal components (PCs) for Geuvadis data.** Population groups in the GEUVADIS data cluster well given the first three genotype PCs which are used as covariates in the cis-trQTL linear regression model to correct for population structure.

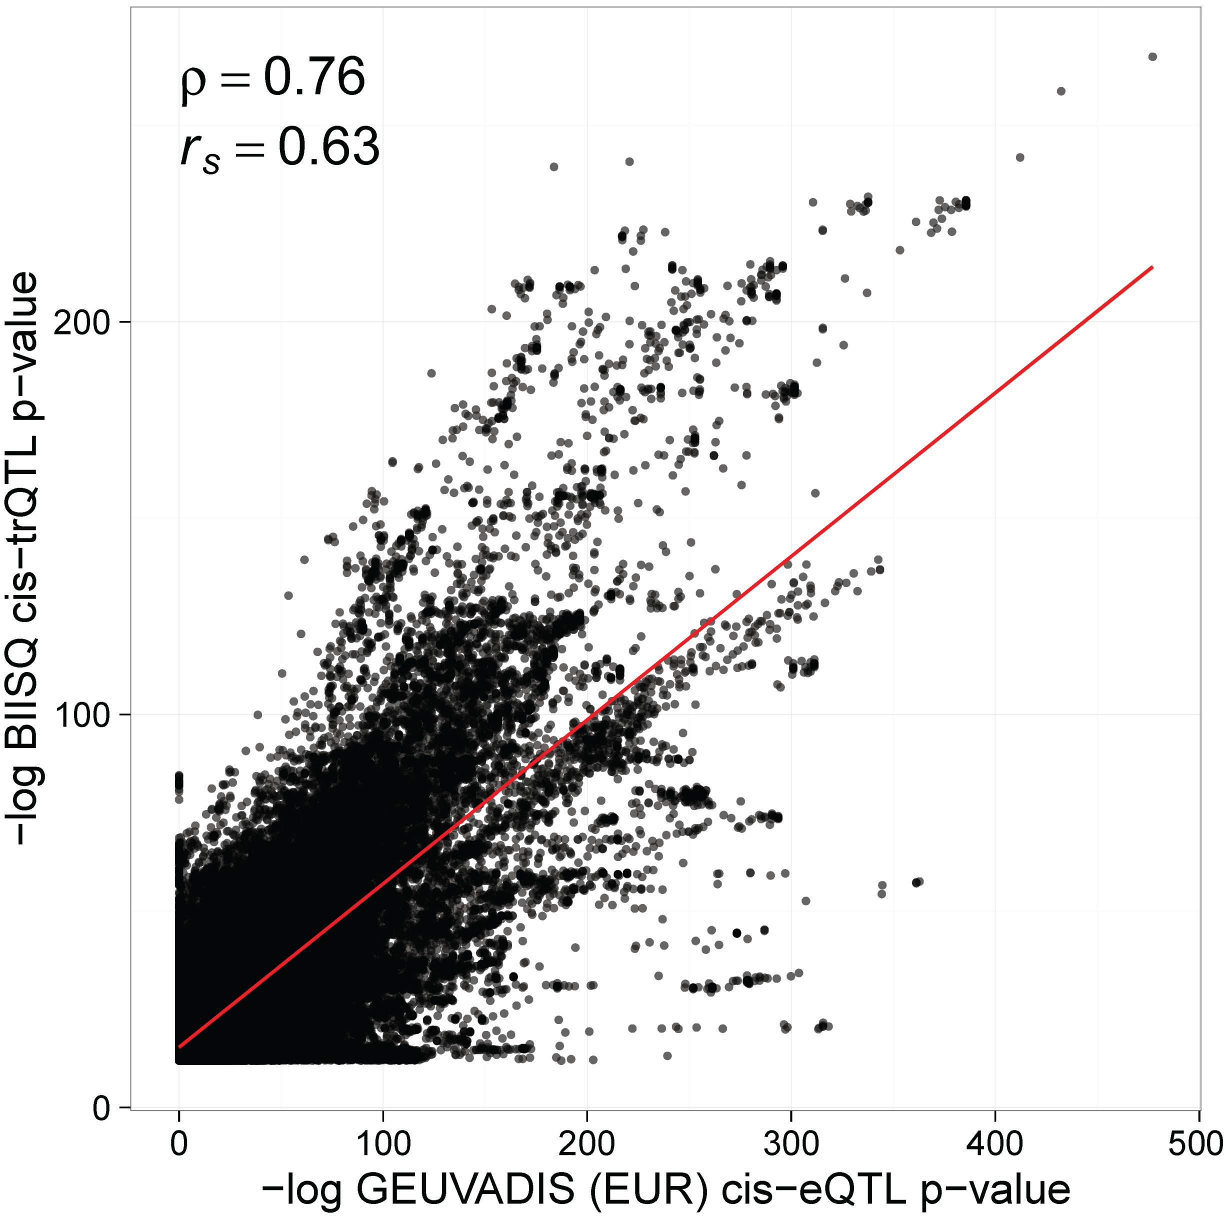


Figure 17: BIISQ **cis-eQTL -log(p-values) vs. GEUVADIS study (EUR population) cis-eQTL -log(p-values).** T-test for significant deviation from $\rho = 0$ and $r_s = 0$ yields $p \leq 2.2 \times 10^{-16}$ and $p \leq 2.2 \times 10^{-16}$ respectively.

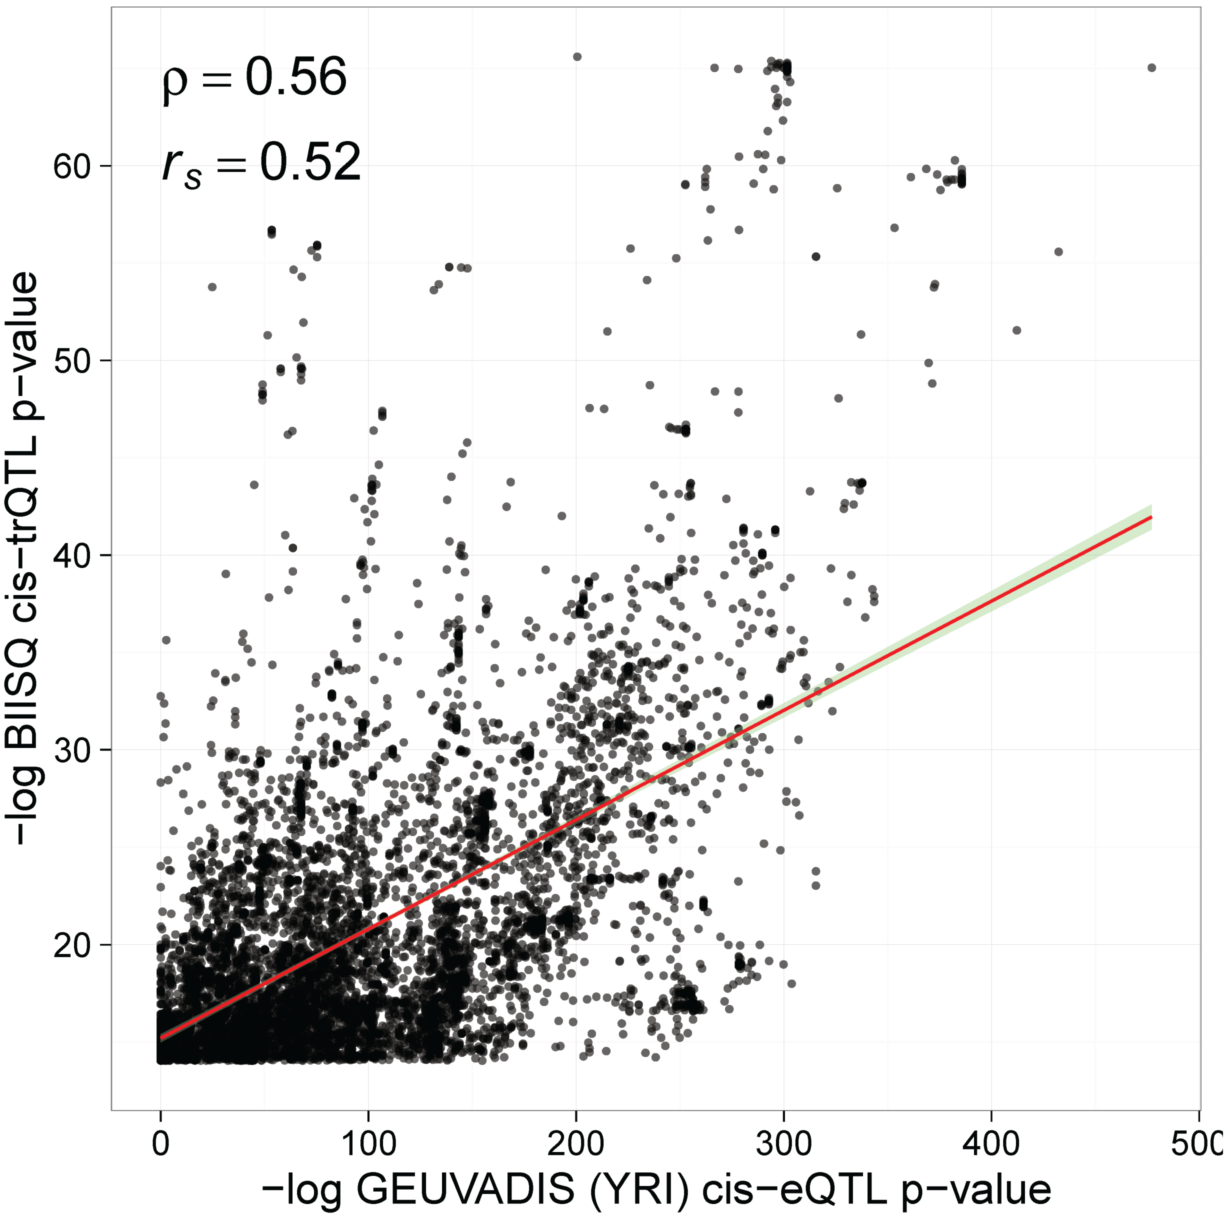


Figure 18: BIISQ **cis-eQTL -log(p-values) vs. GEUVADIS study (YRI population) cis-eQTL -log(p-values).** T-test for significant deviation from $\rho = 0$ and $r_s = 0$ yields $p \leq 2.2 \times 10^{-16}$ and $p \leq 2.2 \times 10^{-16}$ respectively.

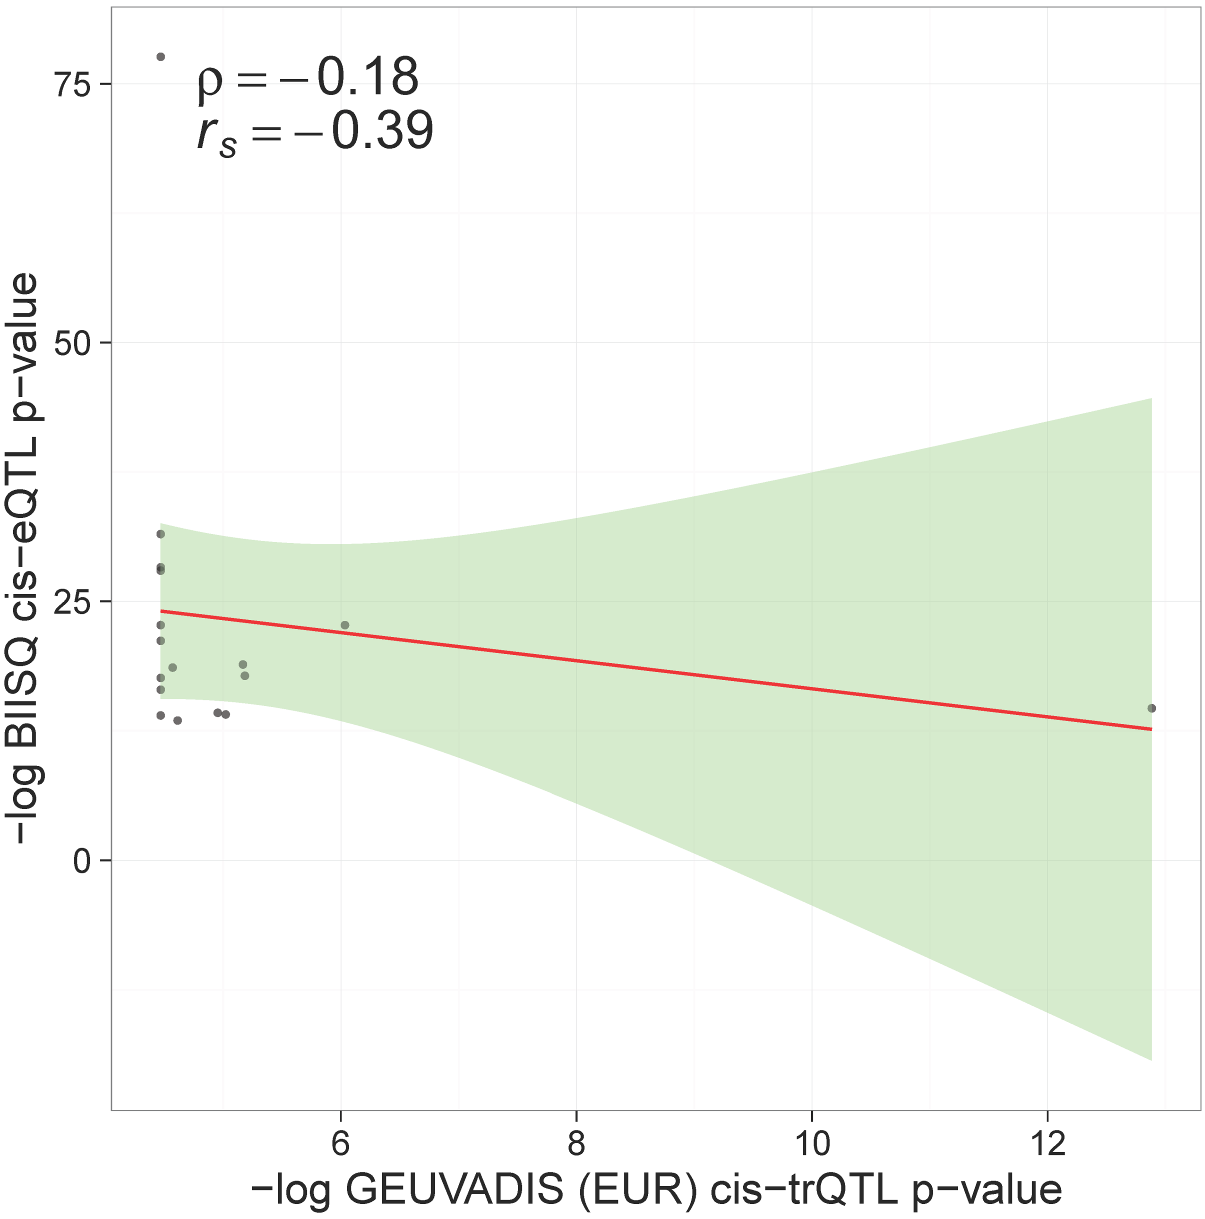


Figure 19: BIISQ **cis-trQTL -log(p-values) vs. GEUVADIS study (EUR population) cis-trQTL -log(p-values).** T-test for significant deviation from $\rho = 0$ and $r_s = 0$ yields $p \leq 0.49$ and $p \leq 0.12$ respectively.

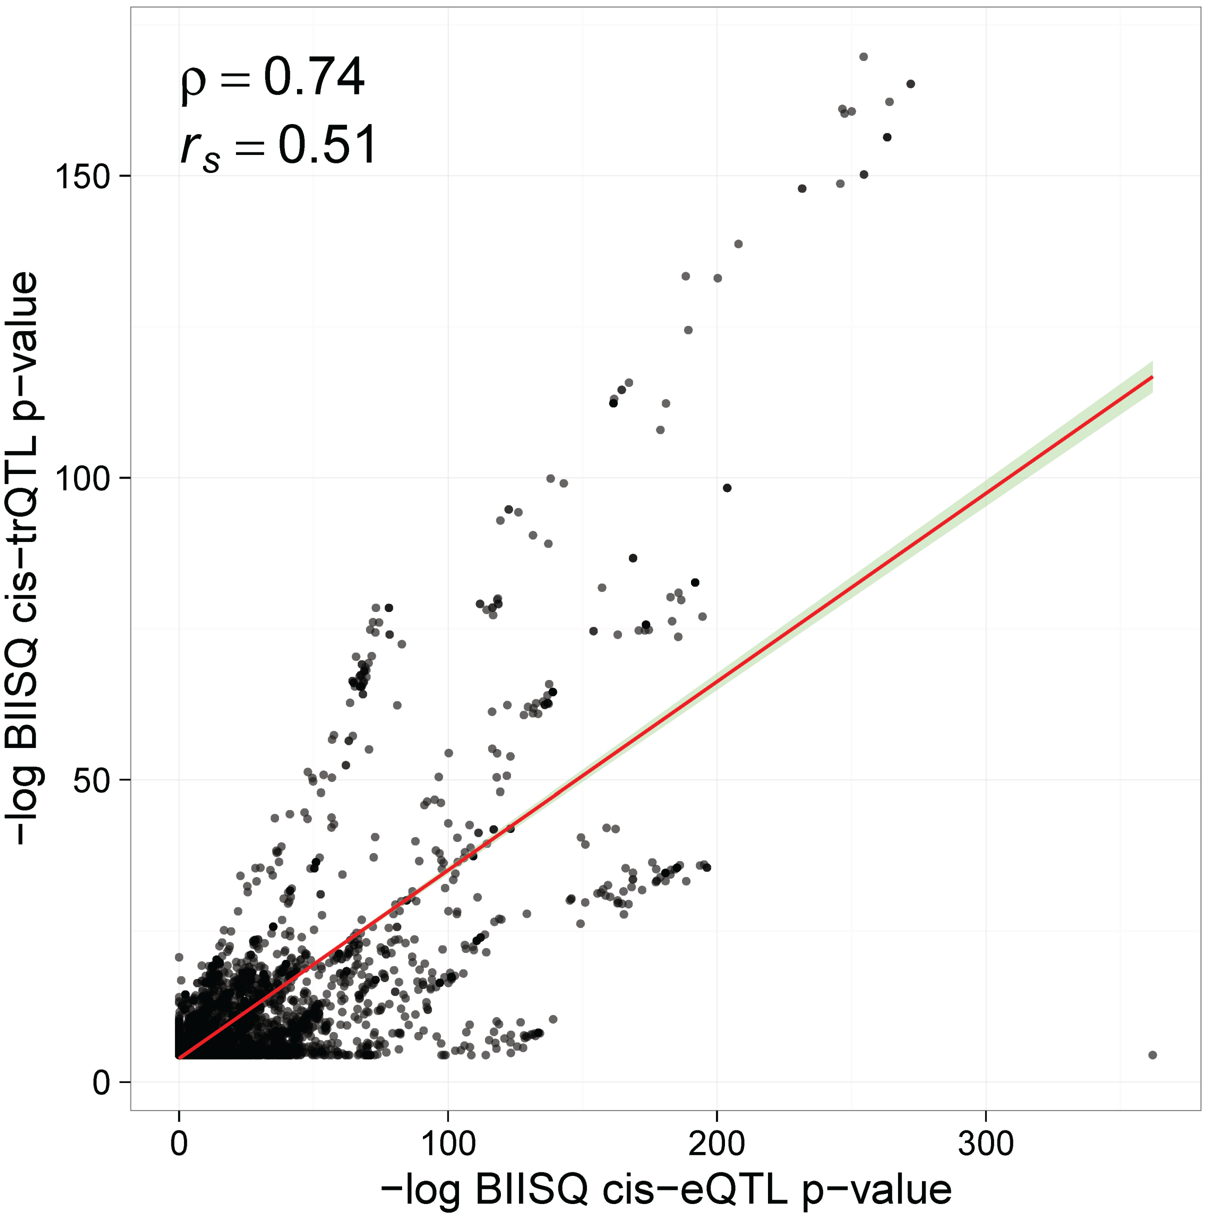


Figure 20: BIISQ **cis-eQTL -log(p-values) vs. BIISQ cis-trQTL -log(p-values).** T-test for significant deviation from $\rho = 0$ and $r_s = 0$ yields $p \leq 2.2 \times 10^{-16}$ and $p \leq 2.2 \times 10^{-16}$ respectively.

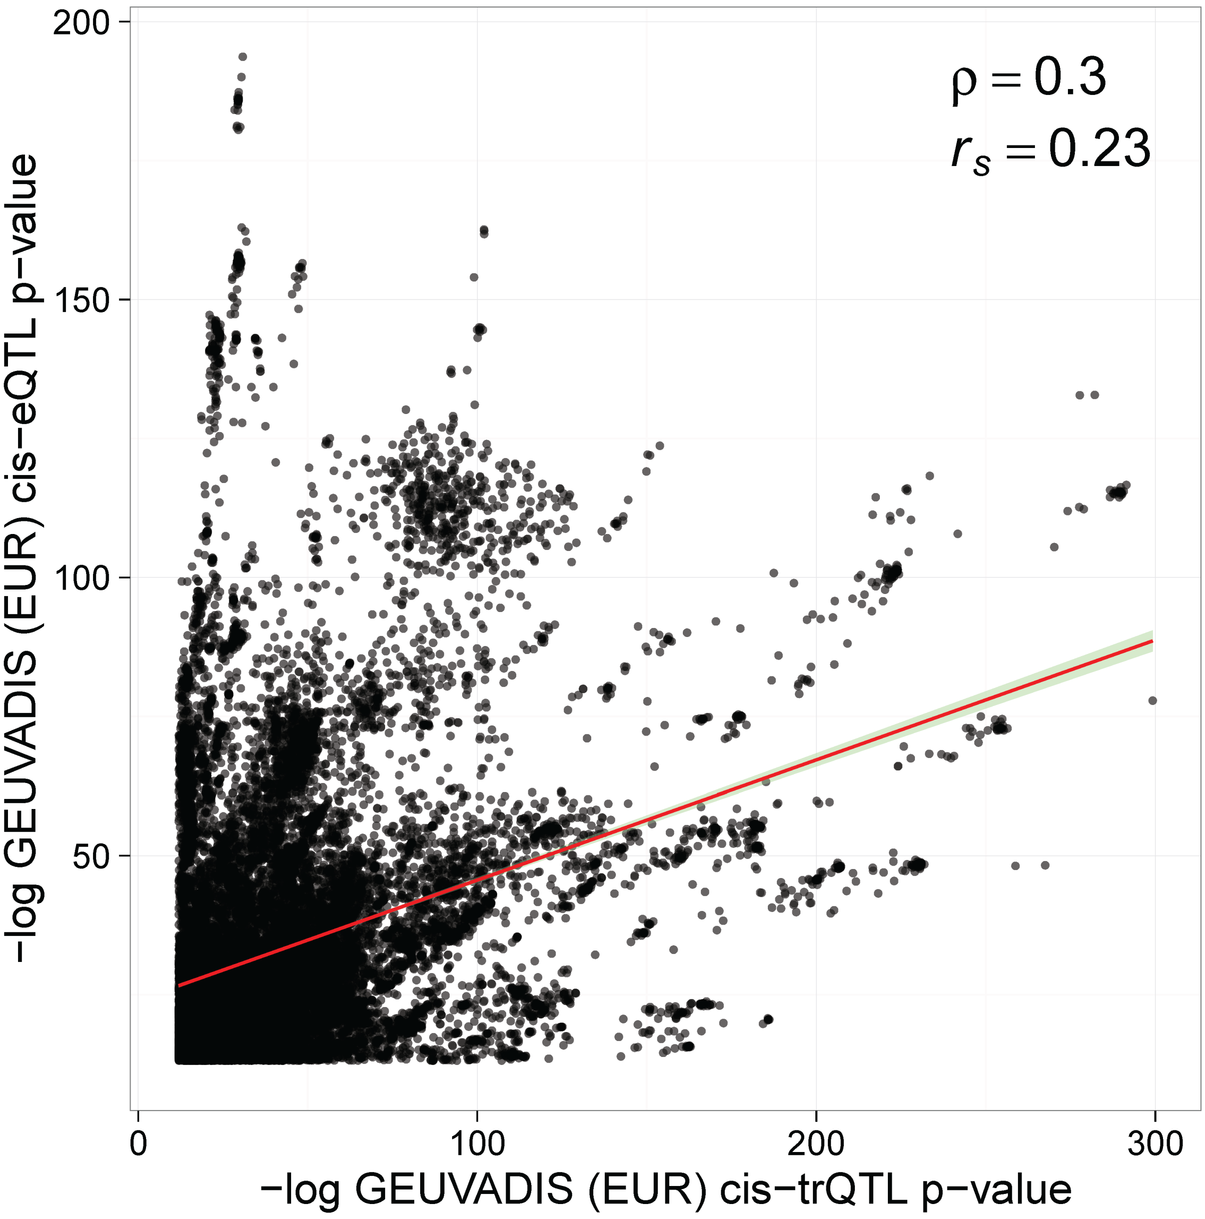


Figure 21: **GEUVADIS study cis-eQTL -log(p-values) vs. GEUVADIS study (EUR population) cis-trQTL -log(p-values).** T-test for significant deviation from $\rho = 0$ and $r_s = 0$ yields $p \leq 2.2 \times 10^{-16}$ and $p \leq 2.2 \times 10^{-16}$ respectively.

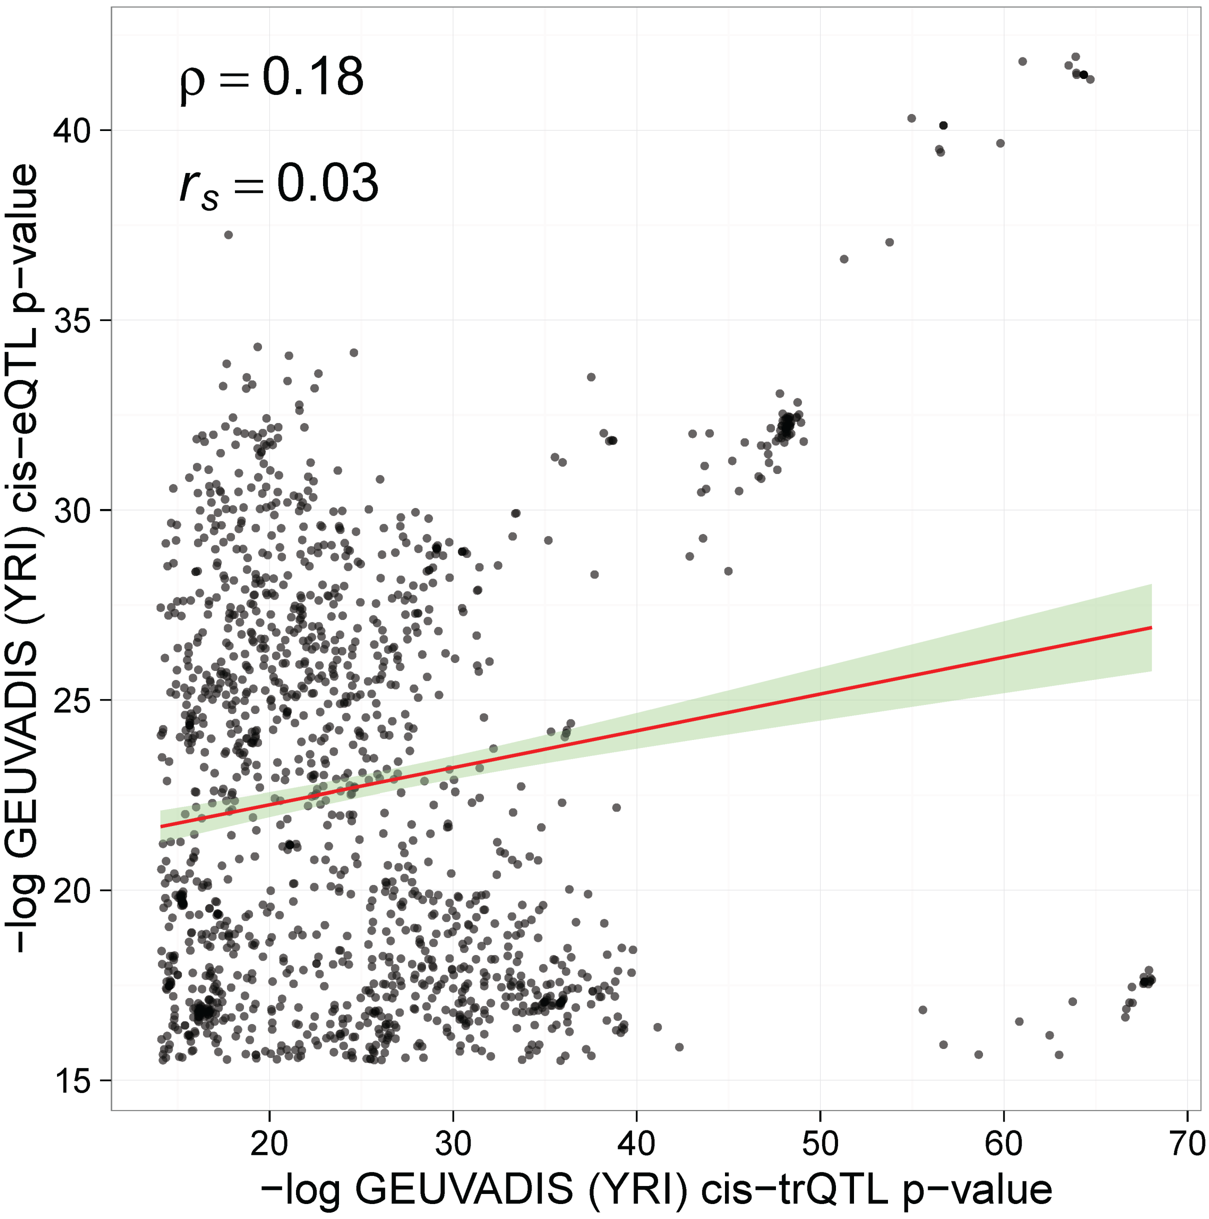


Figure 22: **GEUVADIS study cis-eQTL -log(p-values) vs. GEUVADIS study (YRI population) cis-trQTL -log(p-values).** T-test for significant deviation from $\rho = 0$ and $r_s = 0$ yields $p \leq 8.69 \times 10^{-13}$ and $p \leq 0.21$ respectively.

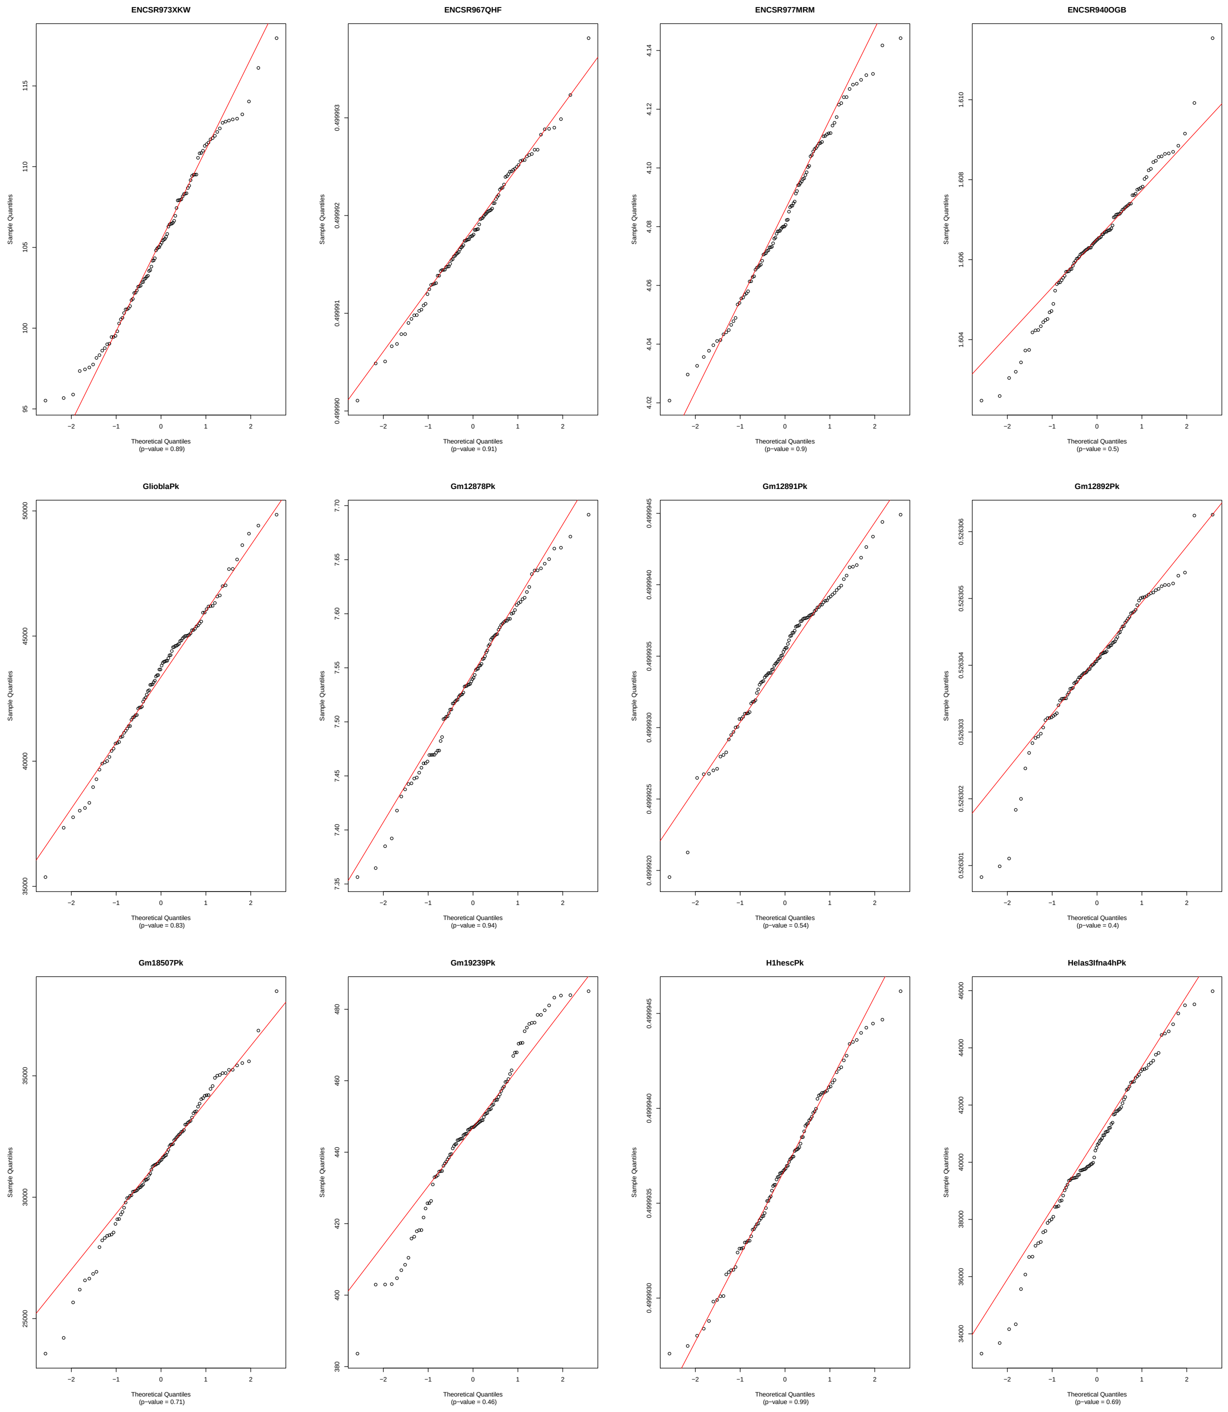

ENCSR973XKW
Theoretical Quantiles
(p−value = 0.89)
ENCSR967QHF
Theoretical Quantiles
(p−value = 0.91)
ENCSR977MRM
Theoretical Quantiles
(p−value = 0.9)
ENCSR940OGB
Theoretical Quantiles
(p−value = 0.5)
GlioblaPk
Theoretical Quantiles
(p−value = 0.83)
Gm12878Pk
Theoretical Quantiles
(p−value = 0.94)
Gm12891Pk
Theoretical Quantiles
(p−value = 0.54)
Gm12892Pk
Theoretical Quantiles
(p−value = 0.4)
Gm18507Pk
Theoretical Quantiles
(p−value = 0.71)
Gm19239Pk
Theoretical Quantiles
(p−value = 0.46)
H1hescPk
Theoretical Quantiles
(p−value = 0.99)
Helas3Ifna4hPk
Theoretical Quantiles
(p−value = 0.69)
Sample Quantiles

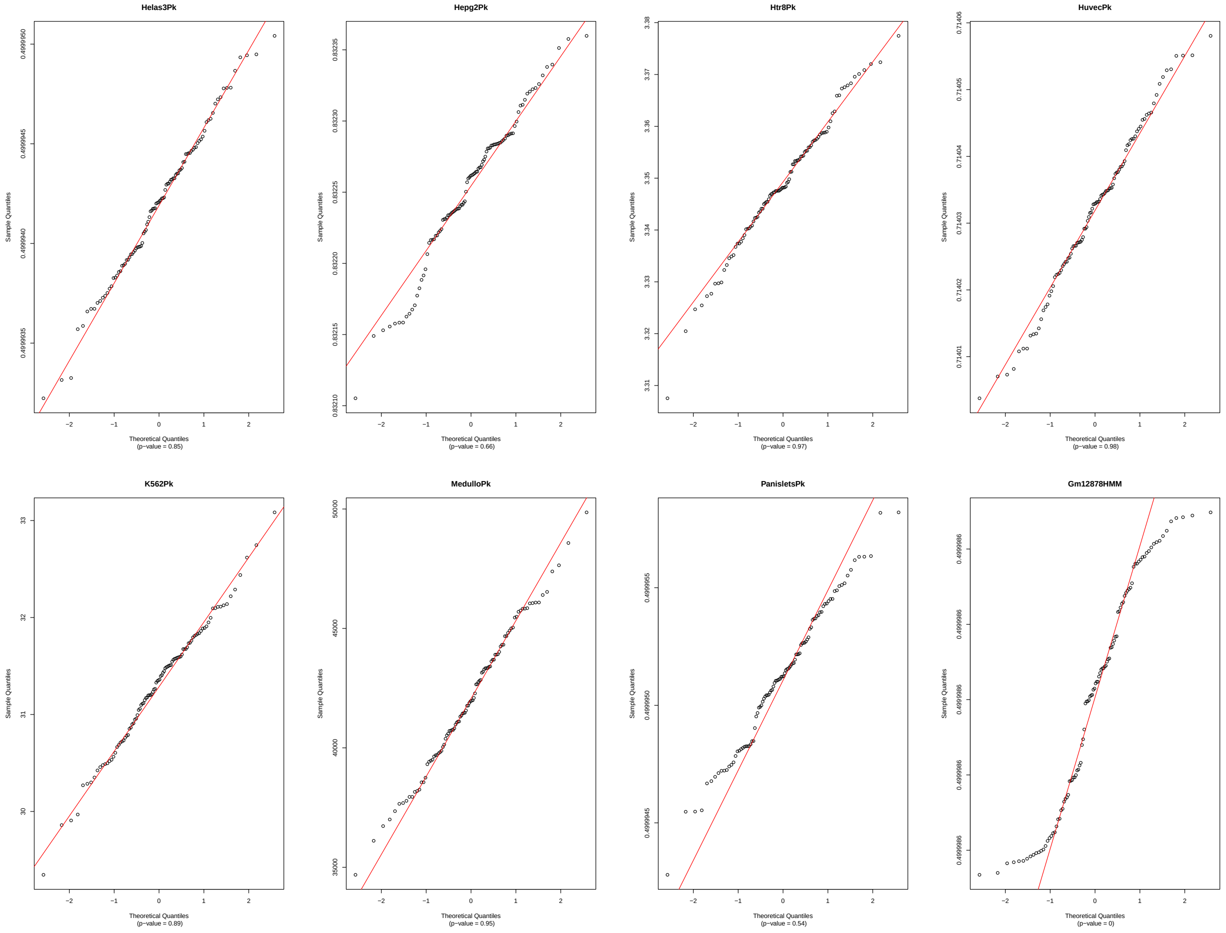


Figure 23: **Theoretical vs. sample quantiles for variant enrichment.** Only sample Gm12878HMM deviates significantly from normal (p-value $\leq 2.2 \times 10^{-16}$).

Table 1: **Iso-Seq gold standard.** Columns include internal ID, chromosome, transcription start site (TSS), transcription end site (TES), and gene symbol.

| internal ID | Chr | TSS | TES | gene symbol |
|---|---|---|---|---|
| $IDISQ\_3426$ | chr15 | 45879574 | 45901903 | *BLOC1S6* |
| $IDISQ\_3491$ | chr15 | 80352035 | 80430726 | *ZFAND6* |
| $IDISQ\_3930$ | chr17 | 76670132 | 76778389 | *CYTH1* |
| $IDISQ\_4630$ | chr21 | 27252863 | 27543410 | *APP* |
| $IDISQ\_4902$ | chr1 | 154179184 | 154193113 | *C1orf43* |
| $IDISQ\_5157$ | chr4 | 88394490 | 88450618 | *SPARCL1* |
| $IDISQ\_5405$ | chr5 | 141348670 | 141368742 | *RNF14* |

Table 2: **GEUVADIS population specific hypergeometric tests.** Overrepresented sets of population specific variants in selected genes with population specific transcript ratios were tested against the set of all non-selected protein coding genes.

| MAF threshold | pop threshold | p-value |
|---|---|---|
| 0.05 | 0.75 | 1.00 |
| 0.05 | 0.80 | 1.00 |
| 0.05 | 0.85 | 1.00 |
| 0.10 | 0.75 | 1.00 |
| 0.10 | 0.80 | 1.00 |
| 0.10 | 0.85 | 0.36 |
| 0.15 | 0.75 | 0.078 |
| 0.15 | 0.80 | 0.019 |
| 0.15 | 0.85 | $1.62 \times 10^{-4}$ |

Table 3: **GEUVADIS super-population specific hypergeometric tests.** Overrepresented sets of super-population specific variants in selected genes with population specific transcript ratios were tested against the set of all non-selected protein coding genes.

| MAF threshold | super pop threshold | p-value |
|---|---|---|
| 0.05 | 0.75 | $1.42 \times 10^{-5}$ |
| 0.05 | 0.80 | 1.00 |
| 0.05 | 0.85 | 1.00 |
| 0.10 | 0.75 | $3.69 \times 10^{-3}$ |
| 0.10 | 0.80 | 1.00 |
| 0.10 | 0.85 | 1.00 |
| 0.15 | 0.75 | $5.71 \times 10^{-3}$ |
| 0.15 | 0.80 | 1.00 |
| 0.15 | 0.85 | 1.00 |

Table 4: **GEUVADIS sex specific hypergeometric tests.** Overrepresented sets of sex specific variants in selected genes with sex specific transcript ratios were tested against the set of all non-selected protein coding genes. NA values indicate fewer than 100 variants selected in total (summed over sex specific and non-sex specific genes as identified by likelihood ratio tests).

| MAF threshold | sex threshold | p-value |
|---|---|---|
| 0.05 | 0.60 | $3.01 \times 10^{-4}$ |
| 0.05 | 0.65 | 0.022 |
| 0.05 | 0.70 | 0.036 |
| 0.10 | 0.60 | 0.0058 |
| 0.10 | 0.65 | 0.42 |
| 0.10 | 0.70 | NA |
| 0.15 | 0.60 | 0.58 |
| 0.15 | 0.65 | NA |
| 0.15 | 0.70 | NA |

Table 5: **PEER factor optimization.** We varied the number of PEER factors and computed the number of cis-trQTL-gene pairs and genes with a cis-trQTL with and without $FDR < 0.05$. The optimal number of PEER factors is $15$ giving a total of $314$ significant cis-trQTLs.

| peer K | var-gene pairs | genes |
|---|---|---|
| 5 | 319 | 33 |
| 10 | 310 | 35 |
| 15 | 314 | 35 |
| 20 | 272 | 26 |
| 25 | 269 | 29 |
| 30 | 267 | 25 |
| 35 | 267 | 26 |
| 40 | 266 | 22 |
| 45 | 283 | 28 |
| 50 | 218 | 17 |

Table 6: **Variant enrichment sample descriptions.** The samples described as *DNaseI/FAIRE/ChIP Synthesis* are a combination of open chromatin regions and transcription factor binding sites from DNaseI hypersensitivity (HS), Formaldehyde-Assisted Isolation of Regulatory Elements (FAIRE), and chromatin immunoprecipitation (ChIP) for regulatory factors described by the ENCODE project [2].

| Sample ID | Accession | Cell type | Description | Ref |
|---|---|---|---|---|
| Bcell-1 | ENCSR973XKW | B cell | Promoter-like regions using DNase and H3K4me3 for B cell | 2 |
| Bcell-2 | ENCSR967QHF | B cell | Enhancer-like regions using DNase-only for B cell | 2 |
| Bcell-3 | ENCSR977MRM | B cell | Enhancer-like regions using DNase and H3K27ac for B cell | 2 |
| Bcell-4 | ENCSR940OGB | B cell | Enhancer-like regions using DNase-only for B cell | 2 |
| LCL-1 | GSM936082 | B-lymphocyte | Chromatin State Segmentation, Multi-assay Synthesis. Source data from ChIP-seq data from the Broad Histone UCSC track for nine factors and nine cell types. | 3 |
| LCL-2 | ENCSR918FQM | B-lymphocyte | DNaseI/FAIRE/ChIP Synthesis from ENCODE/OpenChrom(Duke/UNC/UTA) | 2 |
| LCL-3 | ENCSR601DAI | B-lymphocyte | DNaseI/FAIRE/ChIP Synthesis from ENCODE/OpenChrom(Duke/UNC/UTA) | 2 |
| LCL-4 | ENCSR893EGV | B-lymphocyte | DNaseI/FAIRE/ChIP Synthesis from ENCODE/OpenChrom(Duke/UNC/UTA) | 2 |
| LCL-5 | ENCSR273KTY | B-lymphocyte | DNaseI/FAIRE/ChIP Synthesis from ENCODE/OpenChrom(Duke/UNC/UTA) | 2 |
| LCClusters-1 | No Accession | LeafCutter | DNaseI/FAIRE/ChIP Synthesis from ENCODE/OpenChrom(Duke/UNC/UTA) | 2 |
| Glioblast-1 | ENCSR934HWL | glioblastoma | the H54 and D54 cells come from surgical resection froma glioblastoma multiforme patient. DNaseI/FAIRE/ChIP Synthesis from ENCODE/OpenChrom(Duke/UNC/UTA) | 2 |
| EStemCell-1 | ENCSR236BTH | embryonic stem cell | DNaseI/FAIRE/ChIP Synthesis from ENCODE/OpenChrom(Duke/UNC/UTA) | 2 |
| CervicalC-1 | ENCSR563SKA | cervical carcinoma | DNaseI/FAIRE/ChIP Synthesis from ENCODE/OpenChrom(Duke/UNC/UTA) | 2 |
| CervicalC-2 | ENCSR236YNV | cervical carcinoma | DNaseI/FAIRE/ChIP Synthesis from ENCODE/OpenChrom(Duke/UNC/UTA) | 2 |
| HepatoC-1 | ENCSR283COF | hepatocellular carcinoma | DNaseI/FAIRE/ChIP Synthesis from ENCODE/OpenChrom(Duke/UNC/UTA) | 2 |
| TrophoB-1 | ENCSR066RYF | trophoblast | DNaseI/FAIRE/ChIP Synthesis from ENCODE/OpenChrom(Duke/UNC/UTA) | 2 |
| Endothelial-1 | ENCSR518LJU | umbilical vein endothelial cell | DNaseI/FAIRE/ChIP Synthesis from ENCODE/OpenChrom(Duke/UNC/UTA) | 2 |
| MLeukemia-1 | ENCSR122HHF | mesoderm leukemia | DNaseI/FAIRE/ChIP Synthesis from ENCODE/OpenChrom(Duke/UNC/UTA) | 2 |
| MedulloB-1 | ENCSR237MJM | medulloblastoma | DNaseI/FAIRE/ChIP Synthesis from ENCODE/OpenChrom(Duke/UNC/UTA) | 2 |
| PancreasI-1 | ENCSR441NJL | pancreatic islets | DNaseI/FAIRE/ChIP Synthesis from ENCODE/OpenChrom(Duke/UNC/UTA) | 2 |

Table 7: **Gene annotation categories used in enrichment analysis.**

| abbreviation | description |
|---|---|
| UniProt tissue | literature mined annotations of gene expression specificity |
| InterPro | family and domain classifications for proteins from InterPro |
| KEGG | pathway annotations created from the KEGG database |
| GO-BP | biological processes gene ontology annotations |
| GO-CC | cellular component gene ontology annotations |
| GO-MF | molecular function gene ontology annotations |
| SwissProt | SwissProt or Uniprot and the Protein Information Resource keywords |
| UniProt seq-feature | the annotation category “Uniprot Sequence Feature” that describes regions or sites of interest for proteins |
| OMIM | gene annotations built from the Online Mendelian Inheritance in Man NCBI database |

Table 8: **Functional enrichment for genes with at least one trQTL.**

| Category | Term | Count | List Total | Pop Hits | Pop Total | Fold Enrichment | PValue | Bonferroni | BH FDR |
|---|---|---|---|---|---|---|---|---|---|
| UP_SEQ_FEATURE | sequence variant | 470 | 649 | 12444 | 20064 | 1.167644607 | 1.10E-08 | 2.09E-05 | 2.09E-05 |
| UP_KEYWORDS | Polymorphism | 462 | 667 | 12023 | 20042 | 1.154634028 | 3.20E-07 | 1.26E-04 | 1.26E-04 |
| KEGG_PATHWAY | hsa04740:Olfactory transduction | 33 | 246 | 399 | 6891 | 2.316798093 | 1.06E-05 | 0.002488606 | 0.002488606 |
| UP_KEYWORDS | Olfaction | 33 | 667 | 439 | 20042 | 2.258731682 | 3.02E-05 | 0.011839567 | 0.00593741 |
| UP_KEYWORDS | Glycoprotein | 194 | 667 | 4542 | 20042 | 1.283423018 | 6.84E-05 | 0.026572524 | 0.006710373 |
| UP_KEYWORDS | Sensory transduction | 40 | 667 | 604 | 20042 | 1.989932186 | 6.42E-05 | 0.024993107 | 0.008401422 |
| UP_KEYWORDS | Membrane | 282 | 667 | 7098 | 20042 | 1.193791101 | 1.38E-04 | 0.052776887 | 0.010785537 |
| UP_SEQ_FEATURE | glycosylation site:N-linked (GlcNAc...) | 180 | 649 | 4235 | 20064 | 1.313989554 | 3.65E-05 | 0.067165059 | 0.034166194 |
| GOTERM_MF_DIRECT | GO:0004984 olfactory receptor activity | 32 | 561 | 425 | 16483 | 2.212251232 | 5.72E-05 | 0.036114597 | 0.036114597 |
| UP_KEYWORDS | Disulfide bond | 144 | 667 | 3357 | 20042 | 1.288921223 | 7.64E-04 | 0.260071361 | 0.048961045 |

Table 9: **Functional enrichment for isoforms with $> 1$ transcripts.**

| Category | Term | Count | List Total | Pop Hits | Pop Total | Fold Enrichment | PValue | Bonferroni | BH FDR |
|---|---|---|---|---|---|---|---|---|---|
| UP_KEYWORDS | Alternative splicing | 9043 | 13804 | 10581 | 20042 | 1.240857539 | 0 | 0 | 0 |
| UP_SEQ_FEATURE | splice variant | 6546 | 13613 | 7761 | 20064 | 1.243145586 | 0 | 0 | 0 |
| UP_KEYWORDS | Phosphoprotein | 6275 | 13804 | 7493 | 20042 | 1.215889491 | 3.70E-287 | 2.65E-284 | 1.33E-284 |
| UP_KEYWORDS | Proteomics identification | 2125 | 13804 | 2405 | 20042 | 1.282862059 | 1.69E-124 | 1.21E-121 | 4.04E-122 |
| UP_KEYWORDS | Cytoplasm | 3907 | 13804 | 4750 | 20042 | 1.194224313 | 7.76E-124 | 5.56E-121 | 1.39E-121 |
| UP_KEYWORDS | Acetylation | 2912 | 13804 | 3426 | 20042 | 1.234070922 | 2.38E-123 | 1.71E-120 | 3.41E-121 |
| GOTERM_MF_DIRECT | GO:0005515 protein binding | 6994 | 11974 | 8706 | 16483 | 1.105869728 | 3.65E-122 | 1.27E-118 | 1.27E-118 |
| GOTERM_CC_DIRECT | GO:0005829 cytosol | 2719 | 12629 | 3217 | 17701 | 1.184641617 | 6.68E-82 | 9.53E-79 | 9.53E-79 |
| UP_KEYWORDS | Nucleotide-binding | 1540 | 13804 | 1774 | 20042 | 1.260384961 | 7.00E-75 | 5.02E-72 | 8.36E-73 |
| UP_KEYWORDS | ATP-binding | 1230 | 13804 | 1384 | 20042 | 1.290342876 | 3.99E-73 | 2.86E-70 | 4.09E-71 |
| UP_KEYWORDS | Coiled coil | 2190 | 13804 | 2649 | 20042 | 1.200323375 | 1.18E-66 | 8.49E-64 | 1.06E-64 |
| GOTERM_CC_DIRECT | GO:0005654 nucleoplasm | 2173 | 12629 | 2561 | 17701 | 1.189265955 | 1.80E-66 | 2.57E-63 | 1.28E-63 |
| GOTERM_CC_DIRECT | GO:0005737 cytoplasm | 3855 | 1.26E+04 | 4.80E+03 | 17701 | 1.125906876 | 1.35E-61 | 1.93E-58 | 6.43E-59 |
| UP_TISSUE | Brain | 6275 | 13204 | 8256 | 18913 | 1.088676762 | 4.14E-61 | 2.62E-58 | 2.62E-58 |
| UP_KEYWORDS | Polymorphism | 8797 | 1.38E+04 | 1.20E+04 | 20042 | 1.062326101 | 3.79E-58 | 2.72E-55 | 3.02E-56 |
| UP_SEQ_FEATURE | sequence variant | 8956 | 13613 | 12444 | 20064 | 1.06076152 | 2.08E-57 | 4.47E-53 | 2.23E-53 |
| GOTERM_CC_DIRECT | GO:0016020 membrane | 1631 | 1.26E+04 | 1.90E+03 | 17701 | 1.202543189 | 2.86E-55 | 4.08E-52 | 1.02E-52 |
| UP_KEYWORDS | Metal-binding | 2886 | 1.38E+04 | 3.64E+03 | 20042 | 1.1511477 | 4.37E-54 | 3.14E-51 | 3.14E-52 |
| UP_SEQ_FEATURE | nucleotide phosphate-binding region:ATP | 882 | 13613 | 994 | 20064 | 1.307813679 | 1.41E-55 | 3.04E-51 | 1.01E-51 |
| GOTERM_MF_DIRECT | GO:0005524 ATP binding | 1301 | 11974 | 1467 | 16483 | 1.220799064 | 8.49E-55 | 2.96E-51 | 1.48E-51 |
| UP_KEYWORDS | Cytoskeleton | 970 | 13804 | 1112 | 20042 | 1.266493759 | 1.78E-48 | 1.28E-45 | 1.16E-46 |
| UP_KEYWORDS | Disease mutation | 1987 | 13804 | 2464 | 20042 | 1.170828461 | 1.20E-44 | 8.63E-42 | 7.19E-43 |
| UP_KEYWORDS | Ubl conjugation | 1373 | 1.38E+04 | 1.67E+03 | 20042 | 1.195834406 | 7.31E-39 | 5.24E-36 | 4.03E-37 |
| UP_TISSUE | Epithelium | 2251 | 13204 | 2816 | 18913 | 1.144979607 | 1.82E-39 | 1.15E-36 | 5.77E-37 |
| UP_KEYWORDS | Nucleus | 3932 | 13804 | 5183 | 20042 | 1.101459182 | 4.22E-38 | 3.03E-35 | 2.16E-36 |
| UP_KEYWORDS | Transferase | 1335 | 13804 | 1627 | 20042 | 1.191323805 | 3.53E-36 | 2.53E-33 | 1.69E-34 |
| UP_KEYWORDS | Kinase | 628 | 13804 | 709 | 20042 | 1.286025309 | 7.03E-36 | 5.04E-33 | 3.15E-34 |
| UP_SEQ_FEATURE | mutagenesis site | 1742 | 1.36E+04 | 2.19E+03 | 20064 | 1.171843048 | 7.21E-38 | 1.55E-33 | 3.88E-34 |
| UP_KEYWORDS | Hydrolase | 1346 | 13804 | 1653 | 20042 | 1.182247253 | 2.15E-33 | 1.54E-30 | 9.05E-32 |
| UP_SEQ_FEATURE | active site:Proton acceptor | 587 | 1.36E+04 | 6.72E+02 | 20064 | 1.287456318 | 2.12E-32 | 4.57E-28 | 9.14E-29 |
| UP_SEQ_FEATURE | binding site:ATP | 491 | 13613 | 558 | 20064 | 1.296913371 | 6.79E-29 | 1.46E-24 | 2.44E-25 |
| UP_SEQ_FEATURE | domain:Protein kinase | 427 | 1.36E+04 | 4.78E+02 | 20064 | 1.316629717 | 1.78E-28 | 3.84E-24 | 5.49E-25 |
| UP_KEYWORDS | Transport | 1553 | 13804 | 1965 | 20042 | 1.147479692 | 1.89E-26 | 1.36E-23 | 7.55E-25 |
| UP_KEYWORDS | Zinc | 1844 | 13804 | 2363 | 20042 | 1.13300885 | 2.69E-26 | 1.93E-23 | 1.01E-24 |
| UP_KEYWORDS | Cell cycle | 554 | 13804 | 640 | 20042 | 1.256799207 | 6.92E-26 | 4.96E-23 | 2.48E-24 |
| UP_KEYWORDS | Protein transport | 527 | 13804 | 606 | 20042 | 1.262624169 | 1.05E-25 | 7.56E-23 | 3.60E-24 |
| UP_KEYWORDS | Magnesium | 482 | 13804 | 550 | 20042 | 1.272390611 | 3.18E-25 | 2.28E-22 | 1.04E-23 |
| GOTERM_CC_DIRECT | GO:0005739 mitochondrion | 1037 | 1.26E+04 | 1.24E+03 | 17701 | 1.174050967 | 4.18E-26 | 5.95E-23 | 1.19E-23 |
| UP_KEYWORDS | Cell projection | 575 | 13804 | 675 | 20042 | 1.236802 | 3.87E-23 | 2.77E-20 | 1.21E-21 |
| INTERPRO | IPR011009:Protein kinase-like domain | 474 | 12994 | 530 | 18205 | 1.252997755 | 3.45E-24 | 2.72E-20 | 1.36E-20 |
| INTERPRO | IPR011993:Pleckstrin homology-like domain | 390 | 1.30E+04 | 4.27E+02 | 18205 | 1.279630411 | 2.88E-24 | 2.26E-20 | 2.26E-20 |
| UP_KEYWORDS | Zinc-finger | 1413 | 1.38E+04 | 1.81E+03 | 20042 | 1.136582756 | 4.96E-21 | 3.56E-18 | 1.48E-19 |
| UP_KEYWORDS | Cell division | 337 | 13804 | 378 | 20042 | 1.294417001 | 1.20E-20 | 8.62E-18 | 3.45E-19 |
| INTERPRO | IPR000719:Protein kinase, catalytic domain | 435 | 12994 | 486 | 18205 | 1.254009448 | 2.00E-22 | 1.57E-18 | 5.24E-19 |
| UP_KEYWORDS | Serine/threonine-protein kinase | 350 | 13804 | 395 | 20042 | 1.286491899 | 2.38E-20 | 1.70E-17 | 6.56E-19 |
| UP_KEYWORDS | Mitochondrion | 890 | 13804 | 1103 | 20042 | 1.171522412 | 6.75E-20 | 4.84E-17 | 1.79E-18 |
| INTERPRO | IPR027417:P-loop containing nucleoside triphosphate hydrolase | 739 | 12994 | 871 | 18205 | 1.18870504 | 1.17E-21 | 9.18E-18 | 2.29E-18 |
| UP_KEYWORDS | Chromatin regulator | 262 | 13804 | 287 | 20042 | 1.325426049 | 1.37E-19 | 9.85E-17 | 3.52E-18 |
| UP_KEYWORDS | Endoplasmic reticulum | 854 | 1.38E+04 | 1.06E+03 | 20042 | 1.173056663 | 2.01E-19 | 1.44E-16 | 4.97E-18 |
| UP_KEYWORDS | Isopeptide bond | 815 | 13804 | 1008 | 20042 | 1.173905625 | 9.81E-19 | 7.04E-16 | 2.35E-17 |

| | | | | | | | | | |
|---|---|---|---|---|---|---|---|---|---|
| UP_KEYWORDS | DNA damage | 304 | 1.38E+04 | 3.41E+02 | 20042 | 1.294360681 | 1.06E-18 | 7.59E-16 | 2.45E-17 |
| UP_TISSUE | Uterus | 1439 | 13204 | 1833 | 18913 | 1.124483885 | 6.75E-19 | 4.27E-16 | 1.42E-16 |
| GOTERM_CC_DIRECT | GO:0070062 extracellular exosome | 2162 | 12629 | 2769 | 17701 | 1.094363432 | 8.60E-19 | 1.23E-15 | 2.04E-16 |
| UP_KEYWORDS | Host-virus interaction | 336 | 1.38E+04 | 3.84E+02 | 20042 | 1.270410751 | 1.29E-17 | 9.27E-15 | 2.90E-16 |
| UP_KEYWORDS | WD repeat | 253 | 13804 | 281 | 20042 | 1.30722489 | 5.36E-17 | 3.84E-14 | 1.16E-15 |
| GOTERM_CC_DIRECT | GO:0005813 centrosome | 369 | 12629 | 416 | 17701 | 1.243259752 | 1.17E-17 | 1.66E-14 | 2.37E-15 |
| UP_TISSUE | Placenta | 2687 | 13204 | 3558 | 18913 | 1.081724409 | 1.56E-17 | 9.85E-15 | 2.46E-15 |
| UP_KEYWORDS | Golgi apparatus | 657 | 13804 | 806 | 20042 | 1.18349502 | 2.02E-16 | 1.59E-13 | 4.55E-15 |
| UP_KEYWORDS | Mitosis | 232 | 13804 | 256 | 20042 | 1.315782563 | 1.79E-16 | 1.59E-13 | 4.66E-15 |
| INTERPRO | IPR016024:Armadillo-type fold | 313 | 12994 | 346 | 18205 | 1.267406878 | 5.14E-18 | 4.04E-14 | 8.09E-15 |
| GOTERM_BP_DIRECT | GO:0006468 protein phosphorylation | 401 | 11946 | 447 | 16412 | 1.232468554 | 8.58E-19 | 8.70E-15 | 8.70E-15 |
| KEGG_PATHWAY | hsa01100:Metabolic pathways | 987 | 4936 | 1217 | 6891 | 1.132227433 | 4.03E-17 | 1.20E-14 | 1.20E-14 |
| UP_KEYWORDS | SH3 domain | 198 | 13804 | 215 | 20042 | 1.337096763 | 6.22E-16 | 4.78E-13 | 1.33E-14 |
| UP_KEYWORDS | Helicase | 136 | 13804 | 141 | 20042 | 1.400412256 | 1.14E-15 | 7.96E-13 | 2.15E-14 |
| GOTERM_MF_DIRECT | GO:0044822 poly(A) RNA binding | 929 | 11974 | 1120 | 16483 | 1.141812245 | 3.35E-17 | 1.17E-13 | 3.89E-14 |
| GOTERM_CC_DIRECT | GO:0043231 intracellular membrane-bounded organelle | 459 | 12629 | 533 | 17701 | 1.20701958 | 5.31E-16 | 7.91E-13 | 9.89E-14 |
| GOTERM_BP_DIRECT | GO:0044281 small molecule metabolic process | 1383 | 1.19E+04 | 1.71E+03 | 16412 | 1.113735726 | 2.10E-17 | 2.13E-13 | 1.06E-13 |
| INTERPRO | IPR017441:Protein kinase, ATP binding site | 339 | 12994 | 381 | 18205 | 1.246586856 | 1.01E-16 | 8.73E-13 | 1.25E-13 |
| INTERPRO | IPR015943:WD40/YVTN repeat-like-containing domain | 298 | 1.30E+04 | 3.30E+02 | 18205 | 1.26517367 | 6.33E-17 | 8.73E-13 | 1.46E-13 |
| UP_TISSUE | Teratocarcinoma | 461 | 13204 | 546 | 18913 | 1.209381134 | 2.06E-15 | 1.34E-12 | 2.67E-13 |
| GOTERM_CC_DIRECT | GO:0005794 Golgi apparatus | 667 | 12629 | 802 | 17701 | 1.165682575 | 2.46E-15 | 3.48E-12 | 3.87E-13 |
| UP_KEYWORDS | Transit peptide | 444 | 13804 | 533 | 20042 | 1.209460999 | 2.29E-14 | 1.64E-11 | 4.32E-13 |
| UP_KEYWORDS | DNA repair | 253 | 13804 | 287 | 20042 | 1.279896147 | 3.33E-14 | 2.39E-11 | 6.12E-13 |
| UP_TISSUE | Platelet | 485 | 13204 | 579 | 18913 | 1.199825483 | 6.82E-15 | 4.29E-12 | 7.15E-13 |
| INTERPRO | IPR001849:Pleckstrin homology domain | 256 | 12994 | 281 | 18205 | 1.276384337 | 1.00E-15 | 7.86E-12 | 9.82E-13 |
| GOTERM_CC_DIRECT | GO:0005634 nucleus | 3826 | 12629 | 5071 | 17701 | 1.057499557 | 8.43E-15 | 1.20E-11 | 1.20E-12 |
| GOTERM_CC_DIRECT | GO:0005925 focal adhesion | 343 | 12629 | 391 | 17701 | 1.229550021 | 1.15E-14 | 1.65E-11 | 1.50E-12 |
| INTERPRO | IPR017986:WD40-repeat-containing domain | 272 | 12994 | 301 | 18205 | 1.266048168 | 1.72E-15 | 1.40E-11 | 1.55E-12 |
| UP_KEYWORDS | Microtubule | 248 | 13804 | 282 | 20042 | 1.276846469 | 1.15E-13 | 8.24E-11 | 2.06E-12 |
| UP_SEQ_FEATURE | repeat:WD 3 | 239 | 13613 | 269 | 20064 | 1.309511436 | 1.70E-15 | 3.58E-11 | 4.48E-12 |
| UP_KEYWORDS | Endosome | 393 | 13804 | 470 | 20042 | 1.21403386 | 2.57E-13 | 1.84E-10 | 4.49E-12 |
| UP_SEQ_FEATURE | domain:SH3 | 164 | 13613 | 176 | 20064 | 1.37339308 | 2.06E-15 | 4.54E-11 | 4.54E-12 |
| UP_SEQ_FEATURE | repeat:WD 1 | 246 | 13613 | 278 | 20064 | 1.3042294 | 1.99E-15 | 4.30E-11 | 4.78E-12 |
| UP_SEQ_FEATURE | repeat:WD 2 | 246 | 13613 | 278 | 20064 | 1.3042294 | 1.99E-15 | 4.30E-11 | 4.78E-12 |
| GOTERM_CC_DIRECT | GO:0005730 nucleolus | 676 | 12629 | 819 | 17701 | 1.156888844 | 4.08E-14 | 5.82E-11 | 4.85E-12 |
| UP_KEYWORDS | Ligase | 326 | 13804 | 383 | 20042 | 1.235819186 | 2.90E-13 | 2.08E-10 | 4.96E-12 |
| UP_TISSUE | Kidney | 1224 | 13204 | 1572 | 18913 | 1.115279663 | 8.67E-14 | 5.49E-11 | 7.84E-12 |
| UP_SEQ_FEATURE | compositionally biased region:Ser-rich | 371 | 13613 | 441 | 20064 | 1.239935216 | 7.56E-15 | 1.62E-10 | 1.48E-11 |
| UP_KEYWORDS | Guanine-nucleotide releasing factor | 135 | 13804 | 144 | 20042 | 1.361154376 | 1.34E-12 | 9.62E-10 | 2.24E-11 |
| GOTERM_CC_DIRECT | GO:0005819 spindle | 111 | 12629 | 113 | 17701 | 1.376807979 | 3.86E-13 | 5.49E-10 | 4.23E-11 |
| GOTERM_BP_DIRECT | GO:0010467 gene expression | 796 | 11946 | 958 | 16412 | 1.141527968 | 1.43E-14 | 1.45E-10 | 4.84E-11 |
| GOTERM_CC_DIRECT | GO:0005789 endoplasmic reticulum membrane | 666 | 1.26E+04 | 8.11E+02 | 17701 | 1.151018261 | 5.02E-13 | 7.15E-10 | 5.11E-11 |
| UP_KEYWORDS | Mental retardation | 238 | 13804 | 273 | 20042 | 1.265757231 | 3.17E-12 | 2.27E-09 | 5.16E-11 |
| UP_KEYWORDS | Actin-binding | 233 | 13804 | 267 | 20042 | 1.267012113 | 4.36E-12 | 3.12E-09 | 6.94E-11 |
| GOTERM_BP_DIRECT | GO:0016032 viral process | 469 | 11946 | 544 | 16412 | 1.18443966 | 4.00E-14 | 4.05E-10 | 1.01E-10 |
| UP_SEQ_FEATURE | repeat:WD 4 | 225 | 13613 | 255 | 20064 | 1.300486991 | 7.26E-14 | 1.56E-09 | 1.30E-10 |
| UP_SEQ_FEATURE | domain:PH | 217 | 13613 | 245 | 20064 | 1.305441227 | 8.37E-14 | 1.80E-09 | 1.39E-10 |
| UP_KEYWORDS | Calcium | 686 | 13804 | 868 | 20042 | 1.147467775 | 9.09E-12 | 6.52E-09 | 1.42E-10 |

| | | | | | | | | | |
|---|---|---|---|---|---|---|---|---|---|
| INTERPRO | IPR001452:Src homology-3 domain | 201 | 12994 | 219 | 18205 | 1.285877992 | 2.63E-13 | 2.07E-09 | 2.07E-10 |
| KEGG_PATHWAY | hsa04510:Focal adhesion | 189 | 4936 | 206 | 6891 | 1.280860057 | 1.84E-12 | 5.47E-10 | 2.74E-10 |

Table 10: **Functional enrichment for isoforms with $>4$ transcripts.**

| Category | Term | Count | List Total | Pop Hits | Pop Total | Fold Enrichment | PValue | Bonferroni | BH FDR |
|---|---|---|---|---|---|---|---|---|---|
| UP_KEYWORDS | Alternative splicing | 7362 | 10332 | 10581 | 20042 | 1.349664295 | 0 | 0 | 0 |
| UP_KEYWORDS | Phosphoprotein | 5277 | 10332 | 7493 | 20042 | 1.366117397 | 0 | 0 | 0 |
| UP_SEQ_FEATURE | splice variant | 5408 | 10234 | 7761 | 20064 | 1.366127098 | 0 | 0 | 0 |
| UP_KEYWORDS | Cytoplasm | 3268 | 10332 | 4750 | 20042 | 1.334581494 | 8.67E-167 | 5.98E-164 | 2.99E-164 |
| UP_KEYWORDS | Acetylation | 2444 | 10332 | 3426 | 20042 | 1.383791005 | 4.32E-147 | 2.97E-144 | 9.91E-145 |
| UP_KEYWORDS | ATP-binding | 1138 | 10332 | 1384 | 20042 | 1.595007877 | 1.23E-133 | 8.49E-131 | 2.12E-131 |
| UP_KEYWORDS | Proteomics identification | 1778 | 10332 | 2405 | 20042 | 1.434079858 | 6.40E-126 | 4.41E-123 | 8.82E-124 |
| GOTERM_MF_DIRECT | GO:0005515 protein binding | 5595 | 9153 | 8706 | 16483 | 1.157322041 | 7.39E-127 | 2.32E-123 | 2.32E-123 |
| UP_KEYWORDS | Nucleotide-binding | 1378 | 10332 | 1774 | 20042 | 1.50678838 | 3.85E-124 | 2.66E-121 | 4.43E-122 |
| GOTERM_MF_DIRECT | GO:0005524 ATP binding | 1200 | 9153 | 1467 | 16483 | 1.473071844 | 1.15E-108 | 3.60E-105 | 1.80E-105 |
| GOTERM_CC_DIRECT | GO:0005829 cytosol | 2272 | 9542 | 3217 | 17701 | 1.310133815 | 3.15E-101 | 4.28E-98 | 4.28E-98 |
| UP_TISSUE | Epithelium | 1998 | 10014 | 2816 | 18913 | 1.340033541 | 1.14E-98 | 6.53E-96 | 6.53E-96 |
| UP_SEQ_FEATURE | nucleotide phosphate-binding region:ATP | 820 | 1.02E+04 | 9.94E+02 | 20064 | 1.617333471 | 1.91E-99 | 3.32E-95 | 1.66E-95 |
| UP_KEYWORDS | Coiled coil | 1858 | 1.03E+04 | 2.65E+03 | 20042 | 1.360568499 | 1.97E-96 | 1.36E-93 | 1.94E-94 |
| GOTERM_CC_DIRECT | GO:0005654 nucleoplasm | 1856 | 9542 | 2561 | 17701 | 1.344394674 | 7.80E-96 | 1.06E-92 | 5.30E-93 |
| GOTERM_CC_DIRECT | GO:0005737 cytoplasm | 3152 | 9542 | 4799 | 17701 | 1.218411105 | 2.31E-83 | 3.14E-80 | 1.05E-80 |
| UP_KEYWORDS | Polymorphism | 6855 | 1.03E+04 | 1.20E+04 | 20042 | 1.105990184 | 9.58E-81 | 6.60E-78 | 8.25E-79 |
| GOTERM_CC_DIRECT | GO:0016020 membrane | 1407 | 9542 | 1901 | 17701 | 1.372999473 | 8.24E-81 | 1.12E-77 | 2.80E-78 |
| UP_SEQ_FEATURE | sequence variant | 6965 | 10234 | 12444 | 20064 | 1.097319823 | 6.69E-73 | 1.16E-68 | 3.87E-69 |
| UP_TISSUE | Brain | 4971 | 10014 | 8256 | 18913 | 1.137173981 | 3.53E-70 | 2.02E-67 | 1.01E-67 |
| UP_KEYWORDS | Transferase | 1151 | 10332 | 1627 | 20042 | 1.372285363 | 1.53E-60 | 1.05E-57 | 1.17E-58 |
| UP_KEYWORDS | Kinase | 572 | 10332 | 709 | 20042 | 1.564971576 | 4.94E-60 | 3.40E-57 | 3.40E-58 |
| UP_KEYWORDS | Ubl conjugation | 1171 | 1.03E+04 | 1.67E+03 | 20042 | 1.362630029 | 5.80E-59 | 4.00E-56 | 3.63E-57 |
| UP_KEYWORDS | Cytoskeleton | 819 | 10332 | 1112 | 20042 | 1.428682664 | 5.04E-54 | 3.47E-51 | 2.89E-52 |
| UP_SEQ_FEATURE | mutagenesis site | 1457 | 10234 | 2191 | 20064 | 1.303734868 | 2.00E-54 | 3.47E-50 | 8.68E-51 |
| UP_KEYWORDS | Nucleus | 3138 | 1.03E+04 | 5.18E+03 | 20042 | 1.174433392 | 6.30E-52 | 4.34E-49 | 3.34E-50 |
| UP_SEQ_FEATURE | binding site:ATP | 451 | 10234 | 558 | 20064 | 1.584581019 | 2.74E-49 | 4.75E-45 | 9.51E-46 |
| UP_SEQ_FEATURE | active site:Proton acceptor | 522 | 10234 | 672 | 20064 | 1.522906837 | 3.26E-47 | 5.66E-43 | 9.44E-44 |
| UP_SEQ_FEATURE | domain:Protein kinase | 394 | 10234 | 478 | 20064 | 1.615996559 | 4.09E-47 | 7.11E-43 | 1.02E-43 |
| UP_KEYWORDS | Disease mutation | 1591 | 1.03E+04 | 2.46E+03 | 20042 | 1.252524231 | 2.93E-44 | 2.02E-41 | 1.44E-42 |
| INTERPRO | IPR011993:Pleckstrin homology-like domain | 366 | 9861 | 427 | 18205 | 1.582424269 | 3.04E-44 | 2.05E-40 | 2.05E-40 |
| INTERPRO | IPR011009:Protein kinase-like domain | 437 | 9861 | 530 | 18205 | 1.522212528 | 1.53E-43 | 1.03E-39 | 5.17E-40 |
| UP_KEYWORDS | Hydrolase | 1108 | 10332 | 1653 | 20042 | 1.300240134 | 1.93E-40 | 1.33E-37 | 8.87E-39 |
| INTERPRO | IPR000719:Protein kinase, catalytic domain | 401 | 9861 | 486 | 18205 | 1.523273293 | 4.10E-40 | 2.77E-36 | 9.24E-37 |
| UP_KEYWORDS | Serine/threonine-protein kinase | 326 | 1.03E+04 | 3.95E+02 | 20042 | 1.600947774 | 4.44E-38 | 3.06E-35 | 1.91E-36 |
| UP_KEYWORDS | Cell cycle | 480 | 10332 | 640 | 20042 | 1.454849013 | 6.73E-35 | 4.64E-32 | 2.73E-33 |
| UP_KEYWORDS | Metal-binding | 2208 | 10332 | 3640 | 20042 | 1.176669092 | 1.03E-34 | 7.11E-32 | 3.95E-33 |
| UP_KEYWORDS | Protein transport | 457 | 10332 | 606 | 20042 | 1.462851483 | 3.14E-34 | 2.17E-31 | 1.14E-32 |
| INTERPRO | IPR016024:Armadillo-type fold | 296 | 9861 | 346 | 18205 | 1.579375282 | 1.64E-35 | 1.11E-31 | 2.77E-32 |
| UP_KEYWORDS | WD repeat | 240 | 1.03E+04 | 2.81E+02 | 20042 | 1.656767559 | 8.11E-33 | 5.59E-30 | 2.79E-31 |
| INTERPRO | IPR027417:P-loop containing nucleoside triphosphate hydrolase | 643 | 9861 | 871 | 18205 | 1.362895452 | 2.52E-34 | 1.70E-30 | 2.84E-31 |
| INTERPRO | IPR015943:WD40/YVTN repeat-like-containing domain | 283 | 9.86E+03 | 3.30E+02 | 18205 | 1.583223473 | 2.26E-34 | 1.53E-30 | 3.05E-31 |
| UP_KEYWORDS | DNA damage | 279 | 10332 | 341 | 20042 | 1.587108014 | 2.09E-31 | 1.44E-28 | 6.56E-30 |
| UP_KEYWORDS | Cell projection | 494 | 10332 | 675 | 20042 | 1.419645259 | 2.09E-31 | 1.44E-28 | 6.84E-30 |
| UP_KEYWORDS | Chromatin regulator | 242 | 10332 | 287 | 20042 | 1.635649064 | 2.84E-31 | 1.96E-28 | 8.50E-30 |
| UP_KEYWORDS | Magnesium | 414 | 10332 | 550 | 20042 | 1.460139373 | 9.17E-31 | 6.32E-28 | 2.63E-29 |
| INTERPRO | IPR017986:WD40-repeat-containing domain | 259 | 9861 | 301 | 18205 | 1.588557696 | 5.19E-32 | 3.51E-28 | 5.01E-29 |

| | | | | | | | | | |
|---|---|---|---|---|---|---|---|---|---|
| INTERPRO | IPR001849:Pleckstrin homology domain | 243 | 9861 | 281 | 18205 | 1.596502776 | 8.68E-31 | 5.86E-27 | 7.33E-28 |
| UP_SEQ_FEATURE | repeat:WD 3 | 227 | 1.02E+04 | 2.69E+02 | 20064 | 1.654419665 | 2.54E-30 | 4.42E-26 | 5.52E-27 |
| UP_SEQ_FEATURE | repeat:WD 2 | 233 | 10234 | 278 | 20064 | 1.643172779 | 3.36E-30 | 5.83E-26 | 6.48E-27 |
| UP_SEQ_FEATURE | repeat:WD 1 | 233 | 10234 | 278 | 20064 | 1.643172779 | 3.36E-30 | 5.83E-26 | 6.48E-27 |
| UP_KEYWORDS | Cell division | 298 | 10332 | 378 | 20042 | 1.52925928 | 3.73E-28 | 2.57E-25 | 1.03E-26 |
| INTERPRO | IPR017441:Protein kinase, ATP binding site | 311 | 9861 | 381 | 18205 | 1.506971843 | 1.44E-29 | 9.72E-26 | 1.08E-26 |
| UP_KEYWORDS | Isopeptide bond | 687 | 10332 | 1008 | 20042 | 1.322065174 | 4.58E-28 | 3.16E-25 | 1.21E-26 |
| UP_KEYWORDS | Helicase | 133 | 10332 | 141 | 20042 | 1.829739184 | 4.97E-28 | 3.42E-25 | 1.27E-26 |
| UP_KEYWORDS | DNA repair | 236 | 10332 | 287 | 20042 | 1.595095782 | 2.74E-27 | 1.89E-24 | 6.75E-26 |
| GOTERM_BP_DIRECT | GO:0006468 protein phosphorylation | 362 | 9148 | 447 | 16412 | 1.452902261 | 9.27E-30 | 8.51E-26 | 8.51E-26 |
| GOTERM_CC_DIRECT | GO:0005813 centrosome | 331 | 9542 | 416 | 17701 | 1.476022756 | 4.94E-28 | 6.72E-25 | 1.34E-25 |
| INTERPRO | IPR001680:WD40 repeat | 231 | 9861 | 271 | 18205 | 1.573665463 | 2.32E-27 | 1.57E-23 | 1.57E-24 |
| UP_SEQ_FEATURE | repeat:WD 4 | 213 | 10234 | 255 | 20064 | 1.637613951 | 2.90E-27 | 5.04E-23 | 5.04E-24 |
| GOTERM_MF_DIRECT | GO:0044822 poly(A) RNA binding | 791 | 9153 | 1120 | 16483 | 1.27183642 | 5.32E-27 | 1.67E-23 | 5.57E-24 |
| UP_TISSUE | Platelet | 428 | 10014 | 579 | 18913 | 1.396104866 | 9.01E-26 | 5.15E-23 | 1.72E-23 |
| UP_KEYWORDS | SH3 domain | 183 | 10332 | 215 | 20042 | 1.651084461 | 8.38E-25 | 5.78E-22 | 1.99E-23 |
| UP_TISSUE | Placenta | 2159 | 10014 | 3558 | 18913 | 1.146039362 | 1.97E-25 | 1.12E-22 | 2.25E-23 |
| UP_TISSUE | Uterus | 1179 | 10014 | 1833 | 18913 | 1.2147983 | 1.81E-25 | 1.03E-22 | 2.58E-23 |
| UP_KEYWORDS | Host-virus interaction | 295 | 10332 | 384 | 20042 | 1.490209926 | 1.42E-24 | 9.75E-22 | 3.25E-23 |
| UP_SEQ_FEATURE | domain:PH | 204 | 1.02E+04 | 2.45E+02 | 20064 | 1.632436097 | 8.70E-26 | 1.51E-21 | 1.37E-22 |
| UP_SEQ_FEATURE | repeat:WD 5 | 198 | 10234 | 237 | 20064 | 1.637905913 | 2.05E-25 | 3.57E-21 | 2.97E-22 |
| UP_KEYWORDS | Ligase | 291 | 10332 | 383 | 20042 | 1.47384182 | 5.97E-23 | 4.11E-20 | 1.33E-21 |
| SMART | SM00233:SM00233 | 243 | 5556 | 281 | 9460 | 1.472410321 | 3.00E-24 | 2.08E-21 | 2.08E-21 |
| GOTERM_MF_DIRECT | GO:0004674 protein serine/threonine kinase activity | 271 | 9153 | 331 | 16483 | 1.474395828 | 3.86E-24 | 1.21E-20 | 3.03E-21 |
| INTERPRO | IPR008271:Serine/threonine-protein kinase, active site | 254 | 9861 | 312 | 18205 | 1.50296493 | 5.77E-24 | 3.89E-20 | 3.54E-21 |
| GOTERM_BP_DIRECT | GO:0000278 mitotic cell cycle | 338 | 9148 | 428 | 16412 | 1.416799137 | 3.57E-24 | 3.28E-20 | 1.64E-20 |
| UP_KEYWORDS | Mental retardation | 217 | 10332 | 273 | 20042 | 1.541891261 | 1.48E-21 | 1.02E-18 | 3.19E-20 |
| GOTERM_CC_DIRECT | GO:0043231 intracellular membrane-bounded organelle | 395 | 9542 | 533 | 17701 | 1.374764397 | 2.32E-22 | 3.15E-19 | 5.25E-20 |
| UP_KEYWORDS | Guanine-nucleotide releasing factor | 128 | 10332 | 144 | 20042 | 1.724265497 | 4.95E-21 | 3.41E-18 | 1.03E-19 |
| INTERPRO | IPR011989:Armadillo-like helical | 182 | 9861 | 212 | 18205 | 1.584912357 | 1.93E-22 | 1.30E-18 | 1.08E-19 |
| UP_SEQ_FEATURE | domain:SH3 | 152 | 10234 | 176 | 20064 | 1.693179597 | 1.28E-22 | 2.23E-18 | 1.71E-19 |
| UP_TISSUE | Testis | 2645 | 10014 | 4482 | 18913 | 1.11456823 | 2.03E-21 | 1.16E-18 | 1.94E-19 |
| UP_KEYWORDS | Mitosis | 204 | 10332 | 256 | 20042 | 1.545777076 | 1.48E-20 | 1.02E-17 | 2.99E-19 |
| GOTERM_CC_DIRECT | GO:0005925 focal adhesion | 301 | 9542 | 391 | 17701 | 1.428065502 | 1.94E-21 | 2.64E-18 | 3.30E-19 |
| GOTERM_CC_DIRECT | GO:0005794 Golgi apparatus | 561 | 9542 | 802 | 17701 | 1.297618064 | 1.74E-21 | 2.36E-18 | 3.38E-19 |
| GOTERM_CC_DIRECT | GO:0005730 nucleolus | 571 | 9542 | 819 | 17701 | 1.293333707 | 2.41E-21 | 3.28E-18 | 3.65E-19 |
| INTERPRO | IPR001452:Src homology-3 domain | 186 | 9861 | 219 | 18205 | 1.567972906 | 8.57E-22 | 5.79E-18 | 4.45E-19 |
| GOTERM_CC_DIRECT | GO:0005739 mitochondrion | 824 | 9542 | 1238 | 17701 | 1.234709975 | 3.71E-21 | 5.05E-18 | 5.05E-19 |
| UP_KEYWORDS | Transport | 1202 | 10332 | 1965 | 20042 | 1.186584233 | 5.90E-20 | 4.06E-17 | 1.16E-18 |
| SMART | SM00320:SM00320 | 230 | 5556 | 270 | 9460 | 1.4504173 | 3.91E-21 | 2.70E-18 | 1.35E-18 |
| INTERPRO | IPR002290:Serine/threonine- / dual specificity protein kinase, catalytic domain | 223 | 9861 | 274 | 18205 | 1.502533019 | 4.08E-21 | 2.75E-17 | 1.97E-18 |
| UP_SEQ_FEATURE | compositionally biased region:Ser-rich | 322 | 10234 | 441 | 20064 | 1.431493528 | 1.95E-21 | 3.39E-17 | 2.42E-18 |
| UP_KEYWORDS | Golgi apparatus | 539 | 10332 | 806 | 20042 | 1.297210286 | 1.74E-19 | 1.20E-16 | 3.33E-18 |
| UP_KEYWORDS | Endoplasmic reticulum | 685 | 10332 | 1057 | 20042 | 1.257106999 | 2.12E-19 | 1.46E-16 | 3.96E-18 |
| GOTERM_BP_DIRECT | GO:0006281 DNA repair | 300 | 9148 | 380 | 16412 | 1.416357904 | 1.63E-21 | 1.50E-17 | 4.98E-18 |
| INTERPRO | IPR014001:Helicase, superfamily 1/2, ATP-binding domain | 104 | 9861 | 110 | 18205 | 1.745461921 | 4.08E-20 | 2.76E-16 | 1.84E-17 |
| UP_KEYWORDS | GTPase activation | 160 | 10332 | 195 | 20042 | 1.591629689 | 1.37E-18 | 9.46E-16 | 2.49E-17 |

| | | | | | | | | | |
|---|---|---|---|---|---|---|---|---|---|
| INTERPRO | IPR001650:Helicase, C-terminal | 102 | 9861 | 108 | 18205 | 1.743597111 | 1.23E-19 | 8.31E-16 | 5.19E-17 |
| UP_SEQ_FEATURE | repeat:WD 6 | 162 | 10234 | 196 | 20064 | 1.620432891 | 5.35E-20 | 9.29E-16 | 6.19E-17 |
| GOTERM_BP_DIRECT | GO:0043547 positive regulation of GTPase activity | 364 | 9.15E+03 | 4.81E+02 | 16412 | 1.357661991 | 3.94E-20 | 3.62E-16 | 9.04E-17 |
| UP_TISSUE | T-cell | 256 | 10014 | 338 | 18913 | 1.43046126 | 4.52E-18 | 2.59E-15 | 3.69E-16 |
| UP_SEQ_FEATURE | domain:Helicase C-terminal | 99 | 10234 | 108 | 20064 | 1.797146766 | 5.68E-19 | 9.86E-15 | 6.16E-16 |
| UP_KEYWORDS | Endosome | 331 | 10332 | 470 | 20042 | 1.366113541 | 3.61E-17 | 2.49E-14 | 6.38E-16 |

Table 11: **Functional enrichment for isoforms with $>6$ transcripts.**

| Category | Term | Count | List Total | Pop Hits | Pop Total | Fold Enrichment | PValue | Bonferroni | BH FDR |
|---|---|---|---|---|---|---|---|---|---|
| UP_KEYWORDS | Alternative splicing | 4639 | 6096 | 10581 | 20042 | 1.441430667 | 0 | 0 | 0 |
| UP_KEYWORDS | Phosphoprotein | 3462 | 6096 | 7493 | 20042 | 1.519033775 | 3.70E-303 | 2.35E-300 | 1.18E-300 |
| UP_SEQ_FEATURE | splice variant | 3513 | 6055 | 7761 | 20064 | 1.499905294 | 3.68E-295 | 4.33E-291 | 4.33E-291 |
| UP_KEYWORDS | ATP-binding | 859 | 6096 | 1384 | 20042 | 2.040577873 | 3.03E-140 | 1.93E-137 | 6.43E-138 |
| UP_KEYWORDS | Cytoplasm | 2143 | 6096 | 4750 | 20042 | 1.483285191 | 2.72E-134 | 1.73E-131 | 4.32E-132 |
| UP_TISSUE | Epithelium | 1430 | 5944 | 2816 | 18913 | 1.615790345 | 1.63E-119 | 7.86E-117 | 7.86E-117 |
| GOTERM_MF_DIRECT | GO:0005524 ATP binding | 899 | 5500 | 1467 | 16483 | 1.836551651 | 2.35E-116 | 5.76E-113 | 5.76E-113 |
| UP_KEYWORDS | Nucleotide-binding | 978 | 6096 | 1774 | 20042 | 1.812513871 | 7.46E-114 | 4.75E-111 | 9.49E-112 |
| UP_SEQ_FEATURE | nucleotide phosphate-binding region:ATP | 632 | 6055 | 994 | 20064 | 2.106852178 | 6.42E-110 | 7.54E-106 | 3.77E-106 |
| UP_KEYWORDS | Polymorphism | 4308 | 6096 | 12023 | 20042 | 1.178037043 | 4.08E-95 | 2.60E-92 | 4.33E-93 |
| UP_KEYWORDS | Coiled coil | 1272 | 6096 | 2649 | 20042 | 1.578705974 | 4.73E-93 | 3.01E-90 | 4.30E-91 |
| UP_SEQ_FEATURE | sequence variant | 4367 | 6055 | 12444 | 20064 | 1.162857668 | 2.79E-86 | 3.28E-82 | 1.09E-82 |
| UP_KEYWORDS | Acetylation | 1526 | 6096 | 3426 | 20042 | 1.464411985 | 1.39E-82 | 8.87E-80 | 1.11E-80 |
| GOTERM_MF_DIRECT | GO:0005515 protein binding | 3484 | 5500 | 8706 | 16483 | 1.199314412 | 5.84E-83 | 1.43E-79 | 7.15E-80 |
| GOTERM_CC_DIRECT | GO:0005654 nucleoplasm | 1239 | 5703 | 2561 | 17701 | 1.501606565 | 5.42E-76 | 6.56E-73 | 6.56E-73 |
| GOTERM_CC_DIRECT | GO:0005829 cytosol | 1475 | 5703 | 3217 | 17701 | 1.423099906 | 7.38E-72 | 8.93E-69 | 4.47E-69 |
| UP_TISSUE | Brain | 3137 | 5944 | 8256 | 18913 | 1.209000432 | 6.27E-66 | 3.03E-63 | 1.51E-63 |
| UP_KEYWORDS | Cytoskeleton | 597 | 6096 | 1112 | 20042 | 1.765085078 | 7.87E-62 | 5.01E-59 | 5.56E-60 |
| GOTERM_CC_DIRECT | GO:0016020 membrane | 942 | 5703 | 1901 | 17701 | 1.538024368 | 3.90E-62 | 4.72E-59 | 1.57E-59 |
| UP_KEYWORDS | Proteomics identification | 1086 | 6096 | 2405 | 20042 | 1.484604744 | 1.28E-59 | 8.13E-57 | 8.13E-58 |
| GOTERM_CC_DIRECT | GO:0005737 cytoplasm | 1999 | 5703 | 4799 | 17701 | 1.292874812 | 3.06E-59 | 3.71E-56 | 9.27E-57 |
| UP_KEYWORDS | Kinase | 414 | 6096 | 709 | 20042 | 1.919774441 | 3.28E-55 | 2.09E-52 | 1.90E-53 |
| INTERPRO | IPR016024:Armadillo-type fold | 253 | 5863 | 346 | 18205 | 2.270467091 | 3.91E-55 | 1.92E-51 | 1.92E-51 |
| UP_KEYWORDS | Ubl conjugation | 792 | 6096 | 1667 | 20042 | 1.562016731 | 6.11E-53 | 3.89E-50 | 3.24E-51 |
| INTERPRO | IPR011993:Pleckstrin homology-like domain | 290 | 5863 | 427 | 18205 | 2.108826799 | 3.19E-52 | 1.56E-48 | 7.81E-49 |
| UP_SEQ_FEATURE | binding site:ATP | 333 | 6055 | 558 | 20064 | 1.977485949 | 4.82E-48 | 5.67E-44 | 1.42E-44 |
| INTERPRO | IPR011009:Protein kinase-like domain | 331 | 5863 | 530 | 18205 | 1.939201388 | 3.28E-47 | 1.61E-43 | 5.36E-44 |
| UP_KEYWORDS | Transferase | 754 | 6096 | 1627 | 20042 | 1.523631323 | 3.14E-45 | 2.00E-42 | 1.54E-43 |
| UP_SEQ_FEATURE | mutagenesis site | 957 | 6055 | 2191 | 20064 | 1.447347889 | 8.06E-46 | 9.48E-42 | 1.90E-42 |
| UP_KEYWORDS | Disease mutation | 1053 | 6096 | 2464 | 20042 | 1.405024079 | 8.55E-44 | 5.44E-41 | 3.89E-42 |
| UP_SEQ_FEATURE | domain:Protein kinase | 291 | 6055 | 478 | 20064 | 2.017290596 | 2.26E-44 | 2.65E-40 | 4.42E-41 |
| INTERPRO | IPR015943:WD40/YVTN repeat-like-containing domain | 229 | 5863 | 330 | 18205 | 2.154727386 | 1.13E-43 | 5.56E-40 | 1.39E-40 |
| UP_KEYWORDS | Serine/threonine-protein kinase | 249 | 6096 | 395 | 20042 | 2.07251819 | 4.46E-41 | 2.84E-38 | 1.89E-39 |
| INTERPRO | IPR000719:Protein kinase, catalytic domain | 301 | 5863 | 486 | 18205 | 1.923096225 | 6.65E-42 | 3.26E-38 | 6.52E-39 |
| UP_SEQ_FEATURE | active site:Proton acceptor | 367 | 6055 | 672 | 20064 | 1.809673233 | 1.04E-40 | 1.22E-36 | 1.75E-37 |
| INTERPRO | IPR017986:WD40-repeat-containing domain | 209 | 5863 | 301 | 18205 | 2.156009051 | 5.96E-40 | 2.92E-36 | 4.87E-37 |
| UP_KEYWORDS | Helicase | 118 | 6096 | 141 | 20042 | 2.751433331 | 2.20E-38 | 1.40E-35 | 8.73E-37 |
| UP_KEYWORDS | WD repeat | 190 | 6096 | 281 | 20042 | 2.223020054 | 1.33E-37 | 8.48E-35 | 4.99E-36 |
| UP_TISSUE | Testis | 1761 | 5944 | 4482 | 18913 | 1.250170151 | 4.52E-38 | 2.18E-35 | 7.28E-36 |
| INTERPRO | IPR017441:Protein kinase, ATP binding site | 244 | 5863 | 381 | 18205 | 1.988545991 | 1.86E-37 | 9.13E-34 | 1.30E-34 |
| INTERPRO | IPR027417:P-loop containing nucleoside triphosphate hydrolase | 458 | 5863 | 871 | 18205 | 1.632744059 | 4.01E-37 | 1.97E-33 | 2.46E-34 |
| UP_KEYWORDS | Hydrolase | 730 | 6096 | 1653 | 20042 | 1.451931428 | 4.71E-35 | 3.00E-32 | 1.66E-33 |
| INTERPRO | IPR011989:Armadillo-like helical | 156 | 5863 | 212 | 18205 | 2.284859641 | 1.18E-34 | 5.79E-31 | 6.43E-32 |
| INTERPRO | IPR001849:Pleckstrin homology domain | 191 | 5863 | 281 | 18205 | 2.110560648 | 1.40E-34 | 6.85E-31 | 6.85E-32 |
| UP_SEQ_FEATURE | repeat:WD 1 | 184 | 6055 | 278 | 20064 | 2.193190716 | 4.78E-35 | 5.62E-31 | 7.03E-32 |
| UP_SEQ_FEATURE | repeat:WD 2 | 184 | 6055 | 278 | 20064 | 2.193190716 | 4.78E-35 | 5.62E-31 | 7.03E-32 |

| | | | | | | | | | |
|---|---|---|---|---|---|---|---|---|---|
| UP_KEYWORDS | Cell projection | 351 | 6096 | 675 | 20042 | 1.709619423 | 1.84E-32 | 1.17E-29 | 6.15E-31 |
| UP_SEQ_FEATURE | repeat:WD 3 | 178 | 6055 | 269 | 20064 | 2.19265899 | 6.64E-34 | 7.80E-30 | 8.67E-31 |
| INTERPRO | IPR001680:WD40 repeat | 184 | 5863 | 271 | 18205 | 2.108236467 | 3.06E-33 | 1.50E-29 | 1.37E-30 |
| UP_KEYWORDS | Nucleus | 1911 | 6096 | 5183 | 20042 | 1.212203623 | 1.09E-31 | 6.91E-29 | 3.46E-30 |
| UP_SEQ_FEATURE | domain:PH | 163 | 6055 | 245 | 20064 | 2.204575069 | 1.60E-31 | 1.88E-27 | 1.88E-28 |
| UP_SEQ_FEATURE | repeat:WD 5 | 158 | 6055 | 237 | 20064 | 2.209083402 | 9.92E-31 | 1.17E-26 | 1.06E-27 |
| UP_SEQ_FEATURE | repeat:WD 4 | 166 | 6055 | 255 | 20064 | 2.157104969 | 2.08E-30 | 2.45E-26 | 2.04E-27 |
| GOTERM_MF_DIRECT | GO:0004674 protein serine/threonine kinase activity | 212 | 5500 | 331 | 16483 | 1.919470475 | 2.76E-30 | 6.76E-27 | 2.25E-27 |
| INTERPRO | IPR001650:Helicase, C-terminal | 92 | 5863 | 108 | 18205 | 2.645055938 | 4.11E-29 | 2.02E-25 | 1.68E-26 |
| INTERPRO | IPR014001:Helicase, superfamily 1/2, ATP-binding domain | 93 | 5863 | 110 | 18205 | 2.625191881 | 6.47E-29 | 3.17E-25 | 2.44E-26 |
| UP_KEYWORDS | Chromatin regulator | 177 | 6096 | 287 | 20042 | 2.027624215 | 9.68E-28 | 6.15E-25 | 2.93E-26 |
| UP_KEYWORDS | Guanine-nucleotide releasing factor | 108 | 6096 | 144 | 20042 | 2.465797244 | 1.49E-27 | 9.45E-25 | 4.29E-26 |
| GOTERM_CC_DIRECT | GO:0005813 centrosome | 243 | 5703 | 416 | 17701 | 1.813039949 | 1.99E-28 | 2.41E-25 | 4.82E-26 |
| UP_SEQ_FEATURE | domain:Helicase ATP-binding | 93 | 6055 | 114 | 20064 | 2.703220479 | 6.09E-29 | 7.16E-25 | 5.51E-26 |
| UP_SEQ_FEATURE | domain:Helicase C-terminal | 89 | 6055 | 108 | 20064 | 2.730672539 | 2.50E-28 | 2.94E-24 | 2.10E-25 |
| UP_KEYWORDS | DNA damage | 199 | 6096 | 341 | 20042 | 1.918645754 | 1.05E-26 | 6.69E-24 | 2.91E-25 |
| INTERPRO | IPR002290:Serine/threonine- / dual specificity protein kinase, catalytic domain | 176 | 5863 | 274 | 18205 | 1.994494734 | 1.98E-27 | 9.71E-24 | 6.94E-25 |
| UP_KEYWORDS | Isopeptide bond | 462 | 6096 | 1008 | 20042 | 1.506876094 | 3.27E-26 | 2.08E-23 | 8.65E-25 |
| UP_KEYWORDS | Cell cycle | 319 | 6096 | 640 | 20042 | 1.638727752 | 1.80E-25 | 1.15E-22 | 4.59E-24 |
| UP_KEYWORDS | SH3 domain | 139 | 6096 | 215 | 20042 | 2.125555454 | 8.49E-25 | 5.40E-22 | 2.08E-23 |
| INTERPRO | IPR008271:Serine/threonine-protein kinase, active site | 191 | 5863 | 312 | 18205 | 1.900857507 | 6.36E-26 | 3.12E-22 | 2.08E-23 |
| GOTERM_BP_DIRECT | GO:0043547 positive regulation of GTPase activity | 275 | 5487 | 481 | 16412 | 1.710071092 | 3.74E-27 | 2.86E-23 | 2.86E-23 |
| UP_SEQ_FEATURE | compositionally biased region:Ser-rich | 239 | 6055 | 441 | 20064 | 1.7958195 | 4.41E-26 | 5.19E-22 | 3.46E-23 |
| INTERPRO | IPR011011:Zinc finger, FYVE/PHD-type | 105 | 5863 | 138 | 18205 | 2.362549963 | 1.75E-25 | 8.58E-22 | 5.36E-23 |
| UP_SEQ_FEATURE | repeat:WD 6 | 131 | 6055 | 196 | 20064 | 2.214718819 | 9.09E-26 | 1.07E-21 | 6.68E-23 |
| UP_KEYWORDS | DNA repair | 167 | 6096 | 287 | 20042 | 1.913069174 | 2.23E-22 | 1.42E-19 | 5.25E-21 |
| INTERPRO | IPR003593:AAA+ ATPase domain | 106 | 5863 | 145 | 18205 | 2.269910073 | 2.24E-23 | 1.10E-19 | 6.45E-21 |
| UP_KEYWORDS | Ligase | 206 | 6096 | 383 | 20042 | 1.768335012 | 1.21E-21 | 7.67E-19 | 2.65E-20 |
| UP_KEYWORDS | Protein transport | 295 | 6096 | 606 | 20042 | 1.600462458 | 1.19E-21 | 7.54E-19 | 2.69E-20 |
| UP_TISSUE | Placenta | 1358 | 5944 | 3558 | 18913 | 1.21443828 | 5.94E-22 | 2.87E-19 | 7.18E-20 |
| INTERPRO | IPR001452:Src homology-3 domain | 141 | 5863 | 219 | 18205 | 1.999151867 | 2.75E-22 | 1.35E-18 | 7.48E-20 |
| GOTERM_BP_DIRECT | GO:0006468 protein phosphorylation | 251 | 5487 | 447 | 16412 | 1.679549262 | 2.36E-23 | 1.81E-19 | 9.03E-20 |
| UP_KEYWORDS | Mental retardation | 158 | 6096 | 273 | 20042 | 1.902788594 | 6.58E-21 | 4.18E-18 | 1.39E-19 |
| GOTERM_CC_DIRECT | GO:0030027 lamellipodium | 109 | 5703 | 157 | 17701 | 2.154870998 | 3.74E-21 | 4.52E-18 | 7.53E-19 |
| UP_SEQ_FEATURE | domain:SH3 | 115 | 6055 | 176 | 20064 | 2.165152766 | 1.62E-21 | 1.91E-17 | 1.12E-18 |
| UP_KEYWORDS | GTPase activation | 121 | 6096 | 195 | 20042 | 2.040078404 | 1.45E-19 | 9.20E-17 | 2.97E-18 |
| UP_KEYWORDS | Cell division | 198 | 6096 | 378 | 20042 | 1.722144107 | 3.68E-19 | 2.34E-16 | 7.32E-18 |
| UP_TISSUE | Teratocarcinoma | 272 | 5944 | 546 | 18913 | 1.585104442 | 1.14E-19 | 5.50E-17 | 1.10E-17 |
| UP_KEYWORDS | Actin-binding | 151 | 6096 | 267 | 20042 | 1.859352728 | 9.31E-19 | 5.92E-16 | 1.79E-17 |
| UP_SEQ_FEATURE | repeat:WD 7 | 101 | 6055 | 151 | 20064 | 2.216398248 | 4.28E-20 | 5.04E-16 | 2.80E-17 |
| GOTERM_BP_DIRECT | GO:0046777 protein autophosphorylation | 115 | 5487 | 167 | 16412 | 2.059718725 | 2.10E-20 | 1.60E-16 | 5.35E-17 |
| GOTERM_MF_DIRECT | GO:0005096 GTPase activator activity | 159 | 5500 | 263 | 16483 | 1.811819564 | 2.55E-19 | 6.25E-16 | 1.56E-16 |
| GOTERM_BP_DIRECT | GO:0000278 mitotic cell cycle | 233 | 5487 | 428 | 16412 | 1.628316037 | 1.78E-19 | 1.36E-15 | 3.40E-16 |
| GOTERM_MF_DIRECT | GO:0044822 poly(A) RNA binding | 507 | 5500 | 1120 | 16483 | 1.356636526 | 4.98E-18 | 1.22E-14 | 2.44E-15 |
| INTERPRO | IPR001965:Zinc finger, PHD-type | 70 | 5863 | 91 | 18205 | 2.388512051 | 1.23E-17 | 6.05E-14 | 3.18E-15 |
| UP_KEYWORDS | Magnesium | 258 | 6096 | 550 | 20042 | 1.542244094 | 2.60E-16 | 1.41E-13 | 4.11E-15 |

| | | | | | | | | | |
|---|---|---|---|---|---|---|---|---|---|
| UP_KEYWORDS | Transport | 758 | 6096 | 1965 | 20042 | 1.268243807 | 3.57E-16 | 2.12E-13 | 6.11E-15 |
| UP_SEQ_FEATURE | compositionally biased region:Poly-Glu | 253 | 6055 | 531 | 20064 | 1.578808194 | 9.95E-18 | 1.17E-13 | 6.15E-15 |
| UP_TISSUE | Uterus | 735 | 5944 | 1833 | 18913 | 1.275870206 | 1.57E-16 | 5.36E-14 | 8.88E-15 |
| UP_KEYWORDS | Metal-binding | 1311 | 6096 | 3640 | 20042 | 1.184124611 | 7.66E-16 | 4.94E-13 | 1.38E-14 |
| UP_TISSUE | Platelet | 276 | 5944 | 579 | 18913 | 1.516743492 | 2.05E-16 | 1.07E-13 | 1.53E-14 |
| INTERPRO | IPR019775:WD40 repeat, conserved site | 106 | 5863 | 166 | 18205 | 1.982752775 | 1.26E-16 | 5.44E-13 | 2.72E-14 |
| GOTERM_CC_DIRECT | GO:0005794 Golgi apparatus | 368 | 5703 | 802 | 17701 | 1.424189832 | 1.97E-16 | 2.69E-13 | 3.84E-14 |
| UP_KEYWORDS | TPR repeat | 101 | 6096 | 167 | 20042 | 1.988387398 | 2.67E-15 | 1.69E-12 | 4.59E-14 |

**Supplementary Note: read mapping likelihood.** Let the partial read counts for an isoform $k$ be

$$(\tilde{n_k})_{v=1}^{V} = \left( \sum_{j=1}^{M} \sum_{l=1}^{T} \zeta_{jl}^{k} \sum_{i=1}^{N_j} \phi_{ji}^{l} * \mathbb{I}_{w_{ji}=v} \right) \tag{1}$$

Then, the likelihood for reads $w_{ji}$ for isoform $k$ is

$$P(w_{ji}|\zeta_{ji}, \phi_{ji}, \lambda_k) = \prod_{\forall j} \frac{\Gamma\left(\left(\sum_{v=1}^{V} n_k^v\right) + 1\right) \Gamma\left(\sum_k \lambda_{kv}\right)}{\Gamma\left(\sum_{v=1}^{V} n_k^v + \sum_v \lambda_{kv}\right)} \prod_{v=1}^{V} \frac{\Gamma\left(n_k^v + \lambda_{kv}\right)}{\Gamma\left(n_k^v + 1\right) \Gamma\left(\lambda_{kv}\right)}$$

## Methods

**BEERS simulations.** Single-end simulated data were generated by the *benchmarker for evaluating the effectiveness of RNA-Seq software* (BEERS) [4] software. The parameter sets for our experiments were a constant read length of $100bp$ with a number of novel isoforms (not including full length transcript) in $\{2, 3, 4, 6\}$ and a constant number of novel isoforms of $3$ with a varying read length in $\{50, 200, 400\}$ for seven configurations. We divided RefSeq gene models into three equal exon size groups according to exon count after removing genes with one or two exons, yielding intervals of genes with 3-6 exons, 7-12 exons, and 12-312 exons. For each parameter configuration, we randomly sampled $5$ RefSeq gene models from each exon size group from the gene feature files supplied by BEERS for $105$ simulated gene models; in total, BEERS generated $10,000$ reads for each gene model with no sequencing or read mapping errors, no intron contamination, $0$ substitution and indel frequencies, and high quality read tails.

For each of the gene models, we generated $100$ individuals consisting of aligned RNA-seq reads drawn from the BEERS simulated read pool. The start position of a read was sampled from a gamma distribution with a parameter that decreases linearly with the position to simulate a 5' bias. The exonic composition of novel splice forms were generated by BEERS and isoform proportions for each individual were sampled from a Dirichlet distribution with concentration parameter $1$. The output of this simulation is a file with a row for each read with entries being the sample, mapped isoform, covered exons, start position, reference strand, sequence read content, and CIGAR .mapping string; this file was used to generate the input for BIISQ, CEM, Cufflinks,

and SLIDE.

**PacBio simulations.** We downloaded full length non-chimeric human transcriptome data from liver, heart, and brain from the Iso-Seq protocol which included unaligned sequence read and General Feature Format (GFF) reference files for each tissue [1]. We constructed a reference set of genes and their transcripts across tissues. For each gene, we created a standard set of exons by parsing its transcripts and collapsing overlapping exons. We then mapped genes across the three tissues based on a base-pair overlap of 95%; genes without unique mappings were discarded. For each gene, we then mapped transcripts across tissues: transcripts were successfully mapped if the mapped transcript contained the same number of exons as the original, and the positions of their exons overlapped by 95%. This process was conservative by design to develop a confident baseline of trans-tissue isoforms and yielded seven genes having at least two isoform transcripts across two or more tissues (see Supplementary Table 1): *BLOC1S6*, *ZFAND6*, *CYTH1*, *APP*, *C1orf43*, *SPARCL1*, and *RNF14*.

We extracted the gene sequences of the identified transcripts from human genome version hg19 (Table 1). We mapped the Iso-Seq sequence reads to the gene sequences using both GMAP and STARlong algorithms [5]. We constructed an Iso-Seq short-read simulator (ISSRS) that includes sequencing parameters, a gene reference file containing exon boundaries, and an aligned input file. ISSRS produces SAM files that contain shorter sequence reads but retain the biases and errors present in the Iso-Seq data by copying the CIGAR substring of the shorter sequence reads. In brief, the simulator works as follows: (1) compute usable Iso-Seq reads: for each mapped Iso-Seq read, determine if the proportion $t$ of its mapped bases align to exons from the reference file; (2) for each usable aligned read, determine the amount of sampling based on an input coverage $c$; (3) sample reads from each usable aligned read by attempting to add insert sizes distributed normally with mean 10bp and 40bp standard deviation; (4) output sampled reads while preserving the CIGAR string from the aligned Iso-Seq transcripts in SAM and BIISQ format. For step (1), STARlong mappings yielded fewer false positives than GMAP but GMAP produced many more usable alignments. Because aligned Iso-Seq transcripts are not guaranteed to completely overlap

with exons, step (3) is repeated until 1000 failures in which case the transcript is skipped. This can occur when the sequencing parameters and the Iso-Seq transcript do not produce useful reads.

For the seven transcripts defined in Table 1, we simulated reads with lengths 50bp, 100bp, and 200bp and approximate coverage values (of the input Iso-Seq transcripts) of 0.25, 0.5, 1, and 2 for 50 replicates of the brain and heart tissues (liver did not express these transcripts). Simulated reads that did not match the exons of an expressed isoform were discarded. The coverage values were approximate due to removing Iso-Seq transcripts that did not generate useful read alignments.

**GEUVADIS data processing.** The Genetic European Variation in Health and Disease (GEUVADIS) RNA-sequencing project consists of RNA-seq data from lymphoblastoid cell lines (LCLs) of 666 individuals from the 1000 Genomes Project [6]. BIISQ requires read-terms – mapped RNA-seq read start positions, end positions, and exons covered tuples – and a model of transcription for each gene indicating contiguous transcribed subsequences including exons or retained introns.

To build the transcription model, we first extracted the protein coding and basic (subset of representative transcripts for each gene) transcripts from the comprehensive gene annotations in GENCODE release 19 for human genome assembly version GRCh37.p13. We then built a set of representative exons for each protein coding gene. Most genes had a single transcript annotated as *basic*; for the remaining genes, we retained the transcript with the largest number of exons.

To build the read-terms, we mapped the raw RNA-seq reads with STAR 2-pass to the human genome version 19. Then, we filtered unmapped, non-primary reads that failed quality checks or were marked as duplicates and intersected the remaining mapped reads to our model of transcription (producing the intersection file). The full catalog of read-terms is built by parsing the intersection files of each sample. Each intersection file is then parsed again with the read-term catalog to determine which read-terms are expressed by each sample. A final step reduces the number of read-terms by collapsing read-terms with a similar start position and exon content to an approximate target number of read-terms of 2500.

**Execution of isoform quantification methods.** We compared results from BIISQ with the deterministic method Cufflinks [7], CEM [8], and SLIDE [9]. CEM and Cufflinks are capable of using exon-based reference annotations to influence isoform discovery but Cufflinks is the only method that does not require high-quality gene annotation.

**Statistics for evaluation.** Isoform discovery results are evaluated under two independent sets of assumptions: perfect reconstruction and maximum cardinality minimum weight matchings [10]. A perfect reconstruction is analogous to conventional precision and recall (see Supplementary Figure 13). Precision and recall were calculated based exact full length isoform matches between true (simulated) and estimated isoforms in the usual way (i.e., precision = true positives (TP)/(TP+ false positives (FP)), recall = TP/(TP+false negatives (FN))). *Partial* precision and recall were calculated by defining a maximum cardinality minimum weight matching $M$ between each computed transcript and the true transcripts as follows. Let $k \in 1 : K_C$ and $k \in 1 : K_T$ be the set of estimated and true isoforms respectively which are Boolean vectors of length $E$ exons $\{1, 2, ..., E\}$, where a 1 at position $e$ signifies that exon $e$ is contained within that isoform and $k[e]$ indexes the position of the Boolean vector $k$. We define the distance between an inferred and true isoform $d_{k_T,k_C}$ for all $k_T \in K_T$ and $k_C \in K_C$ to be the Hamming distance. The Hamming distance counts the number of mismatched exons between the estimated and true isoforms. The maximum cardinality minimum weight $M$ is then the solution to the optimization problem

$$\min M = \sum_{k \in 1:K_C} \sum_{l \in 1:K_T} x_{kl} d_{kl} \tag{2}$$

$$\textbf{s.t.} \sum_{k \in 1:K_C} x_{kl} = 1 \qquad \forall l \in 1 : K_T \tag{3}$$

$$\sum_{l \in 1:K_T} x_{kl} = 1 \qquad \forall k \in 1 : K_C \tag{4}$$

$$x_{kl} \in \{0, 1\} \qquad \forall k \in 1 : K_C, \forall l \in 1 : K_T \tag{5}$$

For ease of computation and to ensure conditions 3 and 4 hold, the size of the true and inferred isoform sets must be balanced. Therefore, we add *dummy* isoforms to the smaller set which are connected to each isoform on the opposing set with a large distance $\gg \max(d_{ij})$. If the total number of isoforms is $I$, the augmented assignment problem can be solved in $O(I^3)$ time [11]. Let

$M(k)$ be the $d_{kl}$ in matching $M$ for estimated isoform $k \in K_C$. If $M(k) = 0$, ($M(k) > 0$) then $k$ is a true (false) positive; if $M(k) \leq p|E|$ ($M(k) > p|E|$) then $k$ is a $p$-partial true (false) positive ($p$-TP and $p$-FP). Any true isoform not matched by a $p$-partial true positive is a $p$-partial false negative ($p$-FN). Using these definitions of $p$-TP, $p$-FP, and $p$-FN, we can compute $p$-precision and $p$-recall as above. Note that when $p = 0$, $p$-TP, $p$-FP, and $p$-FN reduce to true and false positives and false negatives.

**Bayesian nonparametric discovery of isoforms and individual specific quantification (BIISQ).** In the following model specification, let there be $M$ input samples (indexed by $j$) each with $N_j$ reads (indexed by $i$). A particular gene contains $E$ exons (indexed by $e$) and the set of global and individual specific isoforms are indexed by $k$ and $l$ respectively. Random variable subscripts indicated by an asterisk denote the full ordered set of indices. We assume RNA-seq reads have been aligned to the transcriptome and our observations are $V$ read-terms which are compositions of the mapped position and sequence.

In our model, our observations are the reads from multiple samples, and our goal is to infer both the global and local sample-specific distributions of the isoforms. We represent each isoform as a probability vector over read terms, as inspired by the topic modeling application using hierarchical Dirichlet process (HDP) [12]. However, an important aspect of isoform discovery is inferring the exon composition of each isoform. We achieve the interpretability by explicitly modeling the isoforms and their exon compositions. We start from introducing the following latent variables. We denote the collection of global isoform as $\boldsymbol{\beta} = (\boldsymbol{\beta}_k)_{k=1}^{\infty}$, where each isoform $\boldsymbol{\beta}_k$ is sampled from a Dirichlet distribution regularized by the exons composition.

Let $\mathbf{b_k} = (\mathbf{b_{k1}}, \mathbf{b_{k2}}, \cdots \mathbf{b_{kV}})$ representing the read term composition of an isoform $k$. Recall that trivially, the $V$ read terms are unique and we assume a consistent ordering of the read terms. Similarly, $\mathbf{b'_k} = (\mathbf{b'_{k1}}, \mathbf{b'_{k2}}, \cdots \mathbf{b'_{kE}})$ is a vector of discrete variable capturing whether exon $e$ is included in the $k$th isoform ($b'_{ke} = 1$) or not ($b'_{ke} = 0$), which is modeled by a Bernoulli distribution with isoform-specific parameter $\pi_k$. We further sample $\pi_k$ from a beta prior and thus this beta-Bernoulli hierarchy produces a beta posterior. Here we link the isoforms and their

exon compositions by computing a read-term-to-exon mapping function $g(x_v, \boldsymbol{b}'_k)$, which indicates whether or not a read-term $x_v$ maps to exon composition $\boldsymbol{b}'_k$.

**The mapping function** $g$**.** Central to our modeling procedure is the function $g$ which maps $E$ dimensional elements $\mathbf{b'_k}$ to $V$ dimensional elements $\mathbf{b_k}$. For simplicity, we number the $E$ exons from $1$ to $E$ according to their spatial ordering (from 5' to 3'). For a read-term $v$, let $M_v$ be the set of indices corresponding to exons $e$ which intersect the read-term, and let $max(M_v)$ and $min(M_v)$ be the maximum and minimum exon index in $M_v$ respectively. Furthermore, let $C(M_v)$ the complement of the set $M_v$ with respect to the set of exons $\{min(M_v, \cdots, max(M_v)\}$. We define the mapping function $g$ as follows:

$$g(x_v, b'_k) = \left(\prod_{e \in M_v} \mathbb{I}_{E[b'_{ke}]>t}\right) \left(\prod_{e \in C(M_v)} 1 - \mathbb{I}_{E[b'_{ke}]>t}\right)$$

Intuitively, the mapping function indicates whether all of the exons included in read-term $v$ are also included in isoform $k$ and all of the exons not included between splice junctions of $v$ are also not included in isoform $k$. For paired-end reads, the mapping function must also check whether the insert size of the read is consistent with the distances between exons in the isoform. However, in both cases, the mapping function is peaked at $0$ or $1$ indicating whether the read-term maps to the isoform.

**Generative model for** BIISQ**.** The generative model of read terms $\{x_1, \ldots, x_v, \ldots, x_V\}$ for isoform $k$ is modeled as a Dirichlet distribution $\beta_k$ and represented as the normalized vector of $V$ independent Gamma distributions. In practice, we allow for some uncertainty $\epsilon$ in the mapping function so

$\beta_k$ is well defined.

$$
\begin{aligned}
\beta_k &= \left(\frac{\tilde{\beta_{k1}}}{\tilde{\beta_k}}, \ldots, \frac{\tilde{\beta_{kV}}}{\tilde{\beta_k}}\right) \sim Dirichlet(b_{k1}\alpha_1, \ldots, b_{kV}\alpha_V) \quad \boldsymbol{\beta}_k \in \mathbb{R}^V \\
\tilde{\beta_{kv}} &\sim Gamma\left(b_{kv}\eta, \alpha_v\right) \quad \text{for } v \in \{1, 2, \cdots, V\} \\
\tilde{\beta_k} &= \sum_{v=1}^{V} \tilde{\beta_{kv}} \sim Gamma\left(\sum_{v=1}^{V} b_{kv}\eta, \alpha_v\right) \\
b_{kv} &= \begin{cases} g(x_v, b'_k) - \epsilon & \text{if } g(x_v, b'_k) = 1 \\ g(x_v, b'_k) + \epsilon & \text{if } g(x_v, b'_k) = 0 \end{cases} \quad \text{for } v \in \{1, 2, \cdots, V\} \\
b'_{ke} &\sim \text{Bernoulli}(\pi_k), \quad \text{for } e \in \{1, 2, \cdots, E\} \\
\pi_k &\sim \text{Beta}(r, s).
\end{aligned} \tag{6}
$$

Next, we denote the global proportion of an isoform $\beta_k$ as $t_k$. BIISQ assumes a Dirichlet process prior on the global isoforms with the base distribution $U_{\mathbb{N}}$ and a concentration parameter $\omega$,

$$G_0 \sim \text{DP}(\omega, U_{\mathbb{N}}). \tag{7}$$

Here $U_{\mathbb{N}}$ denotes the countably infinite set of positive integers, whose binary representation is used to denote the set of all possible isoform collections. Following the sticking-breaking process in [12], we can represent the global isoform distribution as

$$G_0 = \sum_{k=1}^{\infty} t_k \delta_{\boldsymbol{\beta}_k}, \tag{8}$$

where $\delta_{\boldsymbol{\beta}_k}$ represents the probability measure concentrated at isoform $\boldsymbol{\beta}_k$ and has the proportion given by the stick length $t_k$. The proportion for each isoform $t_k$ is generated by the following distributions

$$
\begin{aligned}
t'_k &\sim \text{Beta}(1, \omega), \\
t_k &= t'_k \prod_{x=1}^{k-1} (1 - t'_x).
\end{aligned} \tag{9}
$$

To model sample-specific isoform distributions, we sample it from a Dirichlet process with base distribution as the global isoform distribution $G_0$ and concentration parameter $\alpha$:

$$G_j|\alpha, G_0 \sim \text{DP}(\alpha, G_0). \tag{10}$$

Specifically, a sample-specific isoform distribution consists of a sample-specific collection of isoforms indexed by $\boldsymbol{c_j} = (c_{j,l})_{l=1}^{\infty}$ and corresponding proportions $\boldsymbol{\psi_j} = (\psi_{j,l})_{l=1}^{\infty}$. The indices of sample-specific isoforms $c_{j,l}$ is sampled from the global isoform distribution by

$$c_{j,l} \sim \text{Multinomial}(\boldsymbol{t}), \boldsymbol{t} = (t_k)_{k=1}^{\infty}. \tag{11}$$

Following the stick-breaking process again, we can write the sample-specific isoform distribution as

$$G_j = \sum_{l=1}^{\infty} \psi_{j,l} \delta_{c_{j,l}}, \tag{12}$$

with the sample-specific isoform proportions

$$\begin{aligned} \psi'_{j,l} &\sim \text{Beta}(1, \alpha), \\ \psi_{j,l} &= \psi'_{j,l} \prod_{x=1}^{l-1} (1 - \psi'_{j,x}). \end{aligned} \tag{13}$$

Because draws from the base distribution are discrete, the individual isoform Dirichlet process priors will share global isoform atoms with probability 1. Moreover, the Dirichlet process as a prior distribution on partitions favors larger clusters; that is, the probability of a new observation joining an existing cluster is proportional to the size of that cluster, leading to a *rich-get-richer* phenomenon.

Finally, for each read we observed from the $j$th sample, denoted as $w_{j,i}$, we first model the corresponding isoform assignment by $z_{j,i}$, which is drawn from a multinomial distribution based on the sample-specific isoform proportion $\boldsymbol{\psi_j} = (\psi_{j,l})_{l=1}^{\infty}$:

$$z_{j,i} \sim \text{Multinomial}(\boldsymbol{\psi_j}). \tag{14}$$

Based on the assignment to the sample-specific isoforms, We model each read from a multinomial distribution with probability vector determined by the true global isoforms, or

$$w_{j,i} \sim \text{Multinomial}(\boldsymbol{\beta}_{c_{j,l'}}), \quad l' = z_{j,i}. \tag{15}$$

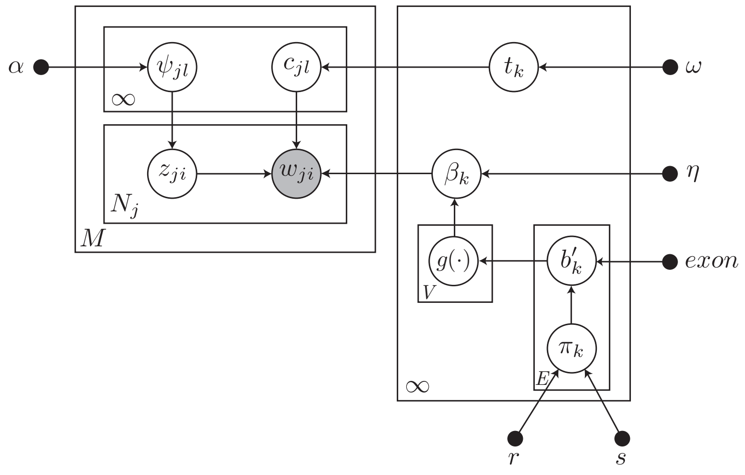


Figure 24: **A graphical model for the generation of reads in RNA-seq data from $M$ samples.** The left block denotes the sample-specific isoform distribution, and the right block denotes the population isoform distribution. The shaded circle denotes the observations (i.e., mapped reads), and the white circles denote the latent variables. The small solid circles on the sides denote the fixed hyperparameters.

Figure 24 summarized the hierarchical generative model we described above. Once the model is fitted to mapped RNA-seq data, BIISQ parameters may be interpreted as biologically informative estimates of:

- $\boldsymbol{\beta}$: the isoforms in the population;
- $t_k$: the proportion of each isoform in the population;
- $\boldsymbol{\psi_j}$: the proportions of the isoforms in each sample $j$;
- $\boldsymbol{b'_k}$: exon composition or the probability of inclusion of each exon in each isoform.

**Stochastic variational inference.** We developed a stochastic variational inference (SVI) method to tractably and robustly estimate posterior probabilities in the BIISQ model, following prior work on SVI for the hierarchical Dirichlet process (HDP) [13]. We modified this method for the BIISQ-

specific model parameters as follows. To handle the expansion and contraction of the population-wide isoforms, we implemented a split-merge step in SVIand executed this step every $30$ iterations.

Variational inference combined with the mean-field assumption converts inference into a tractable optimization problem and one of the most frequently used techniques for optimization is coordinate ascent. In coordinate ascent, we iterate through variational parameters optimizing a single factor while keeping other variables fixed. It is guaranteed to converge to a local optimum. [13] derived the variational update equations for the similar HDP model, which are repeated here for completeness; BIISQ has additional model parameters so capture the composition of isoforms and these updates are derived below.

We define a variational parameter for each model variable (Table 12).

Table 12: Model parameters (arguments of posterior distribution density), their variational distribution and counterpart variational parameters, the complete conditional parameter and relevant expectations.

| Model param. | Distribution | Variational param. | Conditional distribution | Relevant expectation(s) |
|---|---|---|---|---|
| $z_{ij}$ | multinomial (*) | $\phi_{ij}$ | $\log(\psi_{jl}) + \sum_{k=1}^{K} \mathbb{I}_{c_{jl}=k} \log(\beta_{k,w_{ij}})$ | $\mathbb{E}(\mathbb{I}_{z_{ji}=c_{jl}}) = \phi_{ij}^{l}$ |
| $\sigma_{jl}^{-1}(\psi)$ | beta | $\left(\gamma_{jl}^{1}, \gamma_{jl}^{2}\right)$ | $\left(1 + \sum_{i=1}^{N_j} \mathbb{I}_{z_{ji}=c_{jl}}, \alpha + \sum_{i=1}^{N_j} \sum_{k>l} \mathbb{I}_{z_{ji}=c_{jk}}\right)$ | $\mathbb{E}(\log(\psi_{jl})) = \boldsymbol{\psi}(\gamma_{jl}^{1}) - \boldsymbol{\psi}(\gamma_{jl}^{1} + \gamma_{jl}^{2}) + \sum_{x=1}^{l-1} \left(\boldsymbol{\psi}(\gamma_{jx}^{2}) - \boldsymbol{\psi}(\gamma_{jx}^{1} + \gamma_{jx}^{2})\right)$ |
| $c_{jl}$ | multinomial (*) | $\zeta_{jl}$ | $\log(t_k) + \sum_{i=1}^{N_j} \mathbb{I}_{z_{ji}=c_{jl}} \log(\beta_{k,w_{ji}})$ | $\mathbb{E}(\mathbb{I}_{c_{jl}=k}) = \zeta_{jl}^{k}$ |
| $\sigma_{k}^{-1}(t)$ | beta | $\left(a_k^1, a_k^2\right)$ | $\left(1 + \sum_{j=1}^{M} \sum_{l=1}^{T} \mathbb{I}_{c_{jl}=k}, \omega + \sum_{j=1}^{M} \sum_{l=1}^{T} \sum_{x>l} \mathbb{I}_{c_{jl}=x}\right)$ | $\mathbb{E}(\log(t_k)) = \boldsymbol{\psi}(a_k^1) - \boldsymbol{\psi}(a_k^1 + a_k^2) + \sum_{x=1}^{k-1} \left(\boldsymbol{\psi}(a_x^2) - \boldsymbol{\psi}(a_x^1 + a_x^2)\right)$ |
| $\beta_k$ | dirichlet | $\lambda_k$ | $g_v(b'_k) * \left(\eta + \sum_{j=1}^{M} \sum_{l=1}^{T} \mathbb{I}_{c_{jl}=k} \sum_{i=1}^{N_j} \mathbb{I}_{z_{ji}=c_{jl}} \mathbb{I}_{w_{ji}=v}\right)$ | $\mathbb{E}(\log(\beta_{kv})) = \boldsymbol{\psi}(\lambda_{kv}) - \boldsymbol{\psi}\left(\sum_{v'=1}^{V} \lambda_{kv'}\right)$ |
| $\pi_k$ | beta | $\left(\rho_k^1, \rho_k^2\right)$ | $\left(r + \sum_{e=1}^{E} b'_{ke}, s + E - \sum_{e=1}^{E} b'_{ke}\right)$ | $\mathbb{E}(\log \pi_k) = \boldsymbol{\psi}(\rho_k^1) - \boldsymbol{\psi}(\rho_k^1 + \rho_k^2)$ |
| | | | | $\mathbb{E}(\log(1 - \pi_k)) = \boldsymbol{\psi}(\rho_k^2) - \boldsymbol{\psi}(\rho_k^1 + \rho_k^2)$ |
| $b'_{ke}$ | bernoulli | $\mu_{ke}$ | $\log P(b'_{ke} = 1 \vert \pi_k) + \log P(\beta_k \vert b'_{ke} = 1, (b'_{kf})_{f \neq e}, \eta, exons)$ | $\mathbb{E}(b'_{ke}) = \mu_{ke}$, $\mathbb{E}g_v(b'_k)$ |

If the maximum number of isoforms globally and individually is $K$ and $T$ respectively, then the truncated variational distribution is:

$$q(\beta, z, \psi, c, t, b, \pi) = \left(\prod_{k=1}^{K} q(t_k|a_k^1, a_k^2) q(\pi_k|\rho_k) q(\beta_k|\lambda_k) \prod_{e=1}^{E} q(b'_{ke}|\mu_{ke})\right) * \left(\prod_{j=1}^{M}\prod_{l=1}^{T} q(\psi_{jl}|\gamma_{jl}^1, \gamma_{jl}^2) q(c_{jl}|\zeta_{jl}) \prod_{j=1}^{M}\right) * \left(\prod_{i=1}^{N_j} q(z_{ij}|\phi_{ij})\right)$$

The complete conditional distributions for variables $z, \psi, c, t$ remain unchanged with respect to [13], however, the $\beta_k$ is modeled with $V$ gamma distributed random variables $(\tilde{\beta_{kv}})_{v=1}^{V}$ which factor in the mapping function $g(\cdot)$.

$$\tilde{\beta_{kv}}|z, c, w, b', exons, \eta \sim Dirichlet\left(\mathbf{b}_k \cdot \left(\eta + \sum_{j=1}^{M}\sum_{l=1}^{T} \mathbb{I}_{c_{jl}=k} \sum_{i=1}^{N_j} \mathbb{I}_{z_{ji}=c_{jl}} \mathbb{I}_{w_{ji}=v}\right)\right) \quad (16)$$

The read-term mapping function $g_v(b'_k)$ ensures components of the Dirichlet are only valid if the read-term $v$ maps to exon $b'_k$. The inner sum counts the number of reads mapping to individual isoform $l$ while the outer double sum accounts for multiple individuals and the mapping between individual isoform and global isoform.

The exon-mapping **b'** and read-term mapping **b** variables are novel to BIISQ; we marginalize over the $\pi$ variables, but **b'** is an interpretable indicator for isoform composition and thus derive its variational update below. Let $S$ be the set of read-terms $(x_v)_{v=1}^{|S|}$ containing the exon $e \in \{min(M_v), ..., max(M_v)\}$. The conditional for $b'_e$ is:

$$P(b'_{ke}|b_k, \tilde{\beta_k}, \pi, \beta, \kappa, \eta, exons) \propto \prod_{v \in S} P(\tilde{\beta_{kv}}|b'_k, b_k, \kappa, \eta) \int_{\pi} P(b'_{ke}|\pi, exons) P(\pi|r, s) \quad (17)$$

which is a product of Gamma distributions and a beta-Bernoulli. Unfortunately, this is not a known distribution and we cannot exploit conjugacy.We derive the variational update $q_e^*(b'_e)$ using the

expected value of the exponentiated log of the conditional distribution.

$$
\begin{aligned}
q^*_{ke}(b'_{ke}) &\propto exp\left\{\mathbb{E}_{-b'_{ke}}\left[\log\prod_{v\in S}P(\tilde{\beta_{kv}}|\mathbf{b}'_k,\mathbf{b}_k,\eta,\kappa)+\log\int_\pi P(b'_{ke}|\pi,exons)P(\pi|r,s)\right]\right\} \\
&= exp\left\{\mathbb{E}_{-b'_{ke}}\left[\log\prod_{v\in S}Gamma(b_{kv}\eta,\kappa)+\log\int_\pi Bern(b'_{ke}|\pi)Beta(\pi|r,s)\right]\right\} \\
&= exp\Bigg\{\mathbb{E}_{-b'_{ke}}\left[\log\prod_{v\in S}\left(\frac{1}{\Gamma(b_k\eta)\kappa^{b_k\eta}}\tilde{\beta_{kv}}^{b_k\eta-1}e^{-\tilde{\beta_{kv}}/\kappa}\right)\right] \\
&\quad +\mathbb{E}_{-b'_{ke}}\left[\log\left(\frac{(b'_e)^{r-1+\mathbb{I}_{b'_e=1}}(1-b'_e)^{s-1+\mathbb{I}_{b'_e=0}}}{B(r,s)}\right)\right]\Bigg\} \\
&= exp\Bigg\{\mathbb{E}_{-b'_{ke}}\left[\sum_{v\in S}-\log\Gamma\left(b_k\eta\right)-b_k\eta\log\left(\kappa\right)+\left(b_k\eta-1\right)\log\tilde{\beta_{kv}}-\tilde{\beta_{kv}}/\kappa\right] \\
&\quad +(r-1+\mathbb{I}_{b'_e=1})\log\left(b'_e\right)+(s-1+\mathbb{I}_{b'_e=0})\log\left(1-b'_e\right)\Bigg\} \\
&= exp\Bigg\{\sum_{v\in S}-\mathbb{E}_{-b'_{ke}}\left[\log\Gamma\left(b_k\eta\right)\right]-\mathbb{E}_{-b'_{ke}}[b_k]\eta\log\left(\kappa\right) \\
&\quad +\mathbb{E}_{-b'_{ke}}\left[\left(b_k\eta-1\right)\log\tilde{\beta_{kv}}\right]-\frac{1}{\kappa}\mathbb{E}_{-b'_{ke}}[\tilde{\beta_{kv}}] \\
&\quad +(r-1+\mathbb{I}_{b'_e=1})\log\left(b'_e\right)+(s-1+\mathbb{I}_{b'_e=0})\log\left(1-b'_e\right)\Bigg\}
\end{aligned}
$$

$$
\begin{aligned}
q_e^*(b_e') &\propto exp\left\{\mathbb{E}_{-e}\left[\log Dir(\beta|b_e', b_{-e}', \eta, exons) + \log\int_\pi Bern(b_e'|\pi)Beta(\pi|r,s)\right]\right\} \\
&\propto exp\Bigg\{\mathbb{E}_{-e}\left[\log\left(\frac{\Gamma(\sum_{v=1}^V \eta * g_v(b'))}{\prod_{v=1}^V \Gamma(\eta * g_v(b'))}\prod_{v=1}^V \beta_v^{(\eta * g_v(b')-1)}\right)\right] + \\
&\quad \mathbb{E}_{-e}\left[\log\left(\frac{(b_e')^{r-1+\mathbb{I}_{b_e'=1}}(1-b_e')^{s-1+\mathbb{I}_{b_e'=0}}}{B(r,s)}\right)\right]\Bigg\} \\
&\propto exp\Bigg\{\mathbb{E}_{-e}\left[\log\left(\Gamma\left(\sum_{v=1}^V \eta * g_v(b')\right)\right) - \log\left(\prod_{v=1}^V \Gamma(\eta * g_v(b'))\right) + \log\left(\prod_{v=1}^V \beta_v^{(\eta * g_v(b')-1)}\right)\right] \\
&\quad +(r-1+\mathbb{I}_{b_e'=1})\log(b_e') + (s-1+\mathbb{I}_{b_e'=0})\log(1-b_e')\Bigg\} \\
&\sim exp\Bigg\{\log\left(\Gamma\left(\sum_{v=1}^V \eta * g_v(b')\right)\right) - \sum_{v=1}^V \log(\Gamma(\eta * g_v(b'))) + \sum_{v=1}^V (\eta * g_v(b')-1)\mathbb{E}_{-e}[\log(\beta_v)] \\
&\quad +(r-1+\mathbb{I}_{b_e'=1})\log(b_e') + (s-1+\mathbb{I}_{b_e'=0})\log(1-b_e')\Bigg\}
\end{aligned}
$$

where $\mathbb{I}_{b_e'=x}$ is an indicator function for the exon corresponding to $b_e'$ being in isoform $k$. Because $g(\cdot)$ is defined in terms of expectations, it's value is constant, so

$$
\begin{aligned}
&= exp\Bigg\{\sum_{v\in S} - \log\Gamma(b_k\eta) - b_k\eta\log(\kappa) \\
&\quad +(b_k\eta - 1)\mathbb{E}_{\tilde{\beta_{kv}}}\left[\log\tilde{\beta_{kv}}\right] - \frac{1}{\kappa}\mathbb{E}_{\tilde{\beta_{kv}}}[\tilde{\beta_{kv}}] \\
&\quad +(r-1+\mathbb{I}_{b_e'=1})\log(b_e') + (s-1+\mathbb{I}_{b_e'=0})\log(1-b_e')\Bigg\}
\end{aligned}
$$

An exon is either included in the isoform or not, we compute the update for $q_e^*(b_e')$ with $e=0$ and also with $e=1$ and then normalize.

Table 13: **Updates for variational parameters in the BIISQ model.**

$$\phi^l_{ji} \propto \exp(E_q \log \psi_{jl} + \sum_{k=1}^{K} E_q \mathbb{I}(c_{jl} = k) E_q \log \beta_{k,w_{ji}})$$

$$\phi^l_{ji} \propto \exp\left(\boldsymbol{\psi}(\gamma^1_{jl}) - \boldsymbol{\psi}(\gamma^1_{jl} + \gamma^2_{jl}) + \sum_{x=1}^{l-1} \boldsymbol{\psi}(\gamma^2_{jx}) - \boldsymbol{\psi}(\gamma^1_{jx} + \gamma^2_{jx})\right)$$
$$\prod_{k=1}^{K} \exp \zeta^k_{jl} * \exp\left(\boldsymbol{\psi}(\lambda_{kv}) - \boldsymbol{\psi}(\sum_{v'=1}^{V} \lambda_{kv'})\right)$$

---

$$\gamma^1_{jl} \leftarrow 1 + \sum_{i=1}^{N_j} E_q \mathbb{I}(z_{ji} = c_{jl}) \leftarrow 1 + \sum_{i=1}^{N_j} \phi^l_{ji}$$

$$\gamma^2_{jl} \leftarrow \alpha + \sum_{i=1}^{N_j} \sum_{x>l} E_q \mathbb{I}(z_{ji} = c_{jx}) \leftarrow \alpha + \sum_{i=1}^{N_j} \sum_{x>l} \phi^x_{ji}$$

---

$$\zeta^k_{jl} \propto \exp\left(E_q \log t_k + \sum_{i=1}^{N_j} E_q \mathbb{I}(z_{ji} = c_{jl}) E_q \log \beta_{k,w_{ji}}\right)$$

$$\zeta^k_{jl} \propto \exp\left(\boldsymbol{\psi}(a^1_{jl}) - \boldsymbol{\psi}(a^1_{jl} + a^2_{jl}) + \sum_{x=1}^{l-1} \boldsymbol{\psi}(a^2_{jx}) - \boldsymbol{\psi}(a^1_{jx} + a^2_{jx})\right)$$
$$\prod_{i=1}^{N_j} \exp \phi^l_{ji} * \exp\left(\boldsymbol{\psi}(\lambda_{kv}) - \boldsymbol{\psi}(\sum_{v'=1}^{V} \lambda_{kv'})\right)$$

---

$$a^1_k \leftarrow 1 + \sum_{j=1}^{M} \sum_{l=1}^{T} E_q \mathbb{I}(c_{jl} = k) \leftarrow 1 + \sum_{j=1}^{M} \sum_{l=1}^{T} \zeta^k_{jl}$$

$$a^2_k \leftarrow \omega + \sum_{j=1}^{M} \sum_{l=1}^{T} \sum_{x>k} E_q \mathbb{I}(c_{jl} = x) \leftarrow \omega + \sum_{j=1}^{M} \sum_{l=1}^{T} \sum_{x>k} \zeta^x_{jl}$$

---

$$\lambda^v_k \leftarrow E_q g_v(b'_k) * \left(\eta + \sum_{j=1}^{M} \sum_{l=1}^{T} E_q \mathbb{I}_{c_{jl}=k} \sum_{i=1}^{N_j} E_q \mathbb{I}_{z_{ji}=c_{jl}} * \mathbb{I}_{w_{ji}=v}\right)$$

$$\lambda^v_k \leftarrow E_q g_v(b'_k) * \left(\eta + \sum_{j=1}^{M} \sum_{l=1}^{T} \zeta j l^k \sum_{i=1}^{N_j} \phi^l_{ji} * \mathbb{I}_{w_{ji}=v}\right)$$

---

**Additional notes for the $\mu$ update.** To update the variational parameter for $\beta_k$ we iterate through each exon and compute the probability conditional on the exon being turned on and off. This involves computing the expectation of a log Gamma function of a sum of $g_v(b')$. We approximate this expectation using the variational parameter $\mu$ in the summation; tests comparing monte carlo estimates to this approximation showed that the correlation is very high.

**Initialization.** The BIISQ model is nonparametric, and therefore both the total number of isoforms and sample-specific isoform proportions can be as large as the data support, but tend to be approximately $\log(n)$.Because of the presence of exon exclusion splicing, we truncate the total number of isoforms to $2^E - 1$, the theoretical maximum. For genes with many exons, $2^E - 1$ is prohibitively large and initializing the exon selector $\boldsymbol{b'_k}$ vector with $2^E - 1$ isoforms is computationally intractable. Thus, we use the following protocol to initialize isoforms

There are several different methods for initializing isoforms.

1. random: generate a random binary vectors corresponding to random isoforms
2. random: generate isoforms with exon inclusion probabilities following the Beta prior distribution
3. read-term naive: while there is a read-term without an alignment to an isoform, generate a random isoform with the exons specified in read-term
4. read-term cluster: cluster read-terms that are consistent. Generate an isoform for each cluster.

**Algorithm 1: Stochastic variational inference BIISQ.**

**input :** $V$ read-terms, $N_j$ reads for $j$ individuals, convergence criteria
**init :** isoforms $\mu$, Dirichlet parameters $\lambda$ using $\mu$ and $g_v(b')$, $a_1 = 1$, $a_2 = \omega$, step size $\delta_t$
**output:** $\mu_{ke}, \gamma_{jl}, \phi_{ij}$

**while** *(likelihood not converged)* **do**
  // Update individual plate
  **while** *(local parameters not converged)* **do**
    **for** $j$ *in* $(1 : M)$ **do**
      **for** $l$ *in* $(1 : T)$ **do**
        $\gamma^1_{jl} \leftarrow 1 + \sum_{i=1}^{N_j} \phi^l_{ji}$
        $\gamma^2_{jl} \leftarrow \alpha + \sum_{i=1}^{N_j} \sum_{x>l} \phi^x_{ji}$
        **for** $k$ *in* $(1 : K)$ **do**
          $\zeta^k_{jl} \propto \exp\left(E_q \log t_k + \sum_{i=1}^{N_j} E_q \mathbb{I}(z_{ji} = c_{jl}) E_q \log \beta_{k,w_{ji}}\right)$
        **for** $i$ *in* $(1 : N_j)$ **do**
          $\phi^l_{ji} \propto \exp(E_q \log \psi_{jl} + \sum_{k=1}^{K} E_q \mathbb{I}(c_{jl} = k) E_q \log \beta_{k,w_{ji}})$
  // Update isoform plate
  **for** $k$ *in* $(1 : K)$ **do**
    $\hat{a}^1_k \leftarrow 1 + \sum_{j=1}^{M} \sum_{l=1}^{T} \zeta^k_{jl}$
    $\hat{a}^2_k \leftarrow \omega + \sum_{j=1}^{M} \sum_{l=1}^{T} \sum_{x>k} \zeta^x_{jl}$
    **for** $v$ *in* $(1 : V)$ **do**
      $\hat{\lambda}^v_k \leftarrow E_q g_v(b'_k) * \left(\eta + \sum_{j=1}^{M} \sum_{l=1}^{T} \zeta jl^k \sum_{i=1}^{N_j} \phi^l_{ji} * \mathbb{I}_{w_{ji}=v}\right)$
    **for** $e$ *in* $(1 : E)$ **do**
      $\hat{\mu}_{ke} \leftarrow\propto exp \left\{\mathbb{E}_{-e}\left[\log Dir(\beta | b'_e, b'_{-e}, \eta, exons) + \log \int_\pi Bern(b'_e | \pi) Beta(\pi | r, s)\right]\right\}$
  $a^t \leftarrow (1 - \delta_t) a^{t-1} + \delta_t \hat{a}$
  $\lambda^t \leftarrow (1 - \delta_t) \lambda^{t-1} + \delta_t \hat{\lambda}$
  $\mu^t \leftarrow (1 - \delta_t) \mu^{t-1} + \delta_t \hat{\mu}$

1. Biosciences, P. Data Release: Whole Human Transcriptome from Brain, Heart, and Liver. http://www.pacb.com/blog/data-release-whole-human-transcriptome/ (2016). Accessed: 2016-01-15.

2. ENCODE Project Consortium *et al.* An integrated encyclopedia of DNA elements in the human genome. *Nature* **489**, 57–74 (2012).

3. Ernst, J. & Kellis, M. Discovery and characterization of chromatin states for systematic annotation of the human genome. *Nature biotechnology* **28**, 817–825 (2010).

4. Grant, G. R. *et al.* Comparative analysis of RNA-Seq alignment algorithms and the RNA-Seq unified mapper (RUM). *Bioinformatics* **27**, 2518–2528 (2011).

5. Biosciences, P. Bioinfx study: Optimizing STAR aligner for Iso Seq data. (2015). URL https://github.com/PacificBiosciences/cDNA_primer/wiki/. Accessed: 2016-03-29.

6. Lappalainen, T. *et al.* Transcriptome and genome sequencing uncovers functional variation in humans. *Nature* **501**, 506–511 (2013).

7. Trapnell, C. *et al.* Transcript assembly and quantification by RNA-Seq reveals unannotated transcripts and isoform switching during cell differentiation. *Nature biotechnology* **28**, 511–5 (2010).

8. Li, W., Feng, J. & Jiang, T. IsoLasso: A LASSO Regression Approach to RNA-Seq Based Transcriptome Assembly. *Journal of Computational Biology* **18**, 1693–1707 (2011).

9. Li, J. J., Jiang, C.-R., Brown, J. B., Huang, H. & Bickel, P. J. Sparse linear modeling of next-generation mRNA sequencing (RNA-Seq) data for isoform discovery and abundance estimation. *Proceedings of the National Academy of Sciences* **108**, 19867–19872 (2011).

10. Steijger, T. *et al.* Assessment of transcript reconstruction methods for RNA-seq. *Nat Methods* **10**, 1177–1184 (2013).

11. Edmonds, J. & Karp, R. M. Theoretical improvements in algorithmic efficiency for network flow problems. *J. ACM* **19**, 248–264 (1972).

12. Teh, Y. W., Jordan, M. I., Beal, M. J. & Blei, D. M. Hierarchical Dirichlet Processes. *Journal of the american statistical association* **101** (2006).

13. Hoffman, M. D., Blei, D. M., Wang, C. & Paisley, J. W. Stochastic variational inference. *Journal of Machine Learning Research* **14**, 1303–1347 (2013).
